# Supplementary material for: Inference on an heteroscedastic Gompertz tumor growth model
Source: arXiv:2401.15382 ancillary file (2024-01-27)
Supplement: Supplementary file 1 [file Supplementary_Material.pdf]

# Supplementary Material: Inference on an heteroscedastic Gompertz tumor growth model

G. Albano<sup>a,\*</sup>, V. Giorno<sup>b</sup>, P. Román-Román<sup>c,d</sup>, S. Román-Román<sup>e</sup>, J. J. Serrano-Pérez<sup>c</sup>, F. Torres-Ruiz<sup>c,d</sup>

<sup>a</sup>*Dipartimento di Studi Politici e Sociali, Università of Salerno, Italy*

<sup>b</sup>*Dipartimento di Informatica, Università of Salerno, Italy*

<sup>c</sup>*Departamento de Estadística e Investigación Operativa, Universidad de Granada, Spain*

<sup>d</sup>*Instituto de Matemáticas (IEMath-GR), Universidad de Granada, Spain*

<sup>e</sup>*Dép. de Recherche Translationnelle, Institut Curie, France*

---

---

---

\*Corresponding author.

*Email addresses:* pialbano@unisa.it (G. Albano), giorno@unisa.it (V. Giorno), proman@ugr.es (P. Román-Román), sergio.Roman-Roman@curie.fr (S. Román-Román), jjserra@ugr.es (J. J. Serrano-Pérez), fdeasis@ugr.es (F. Torres-Ruiz)

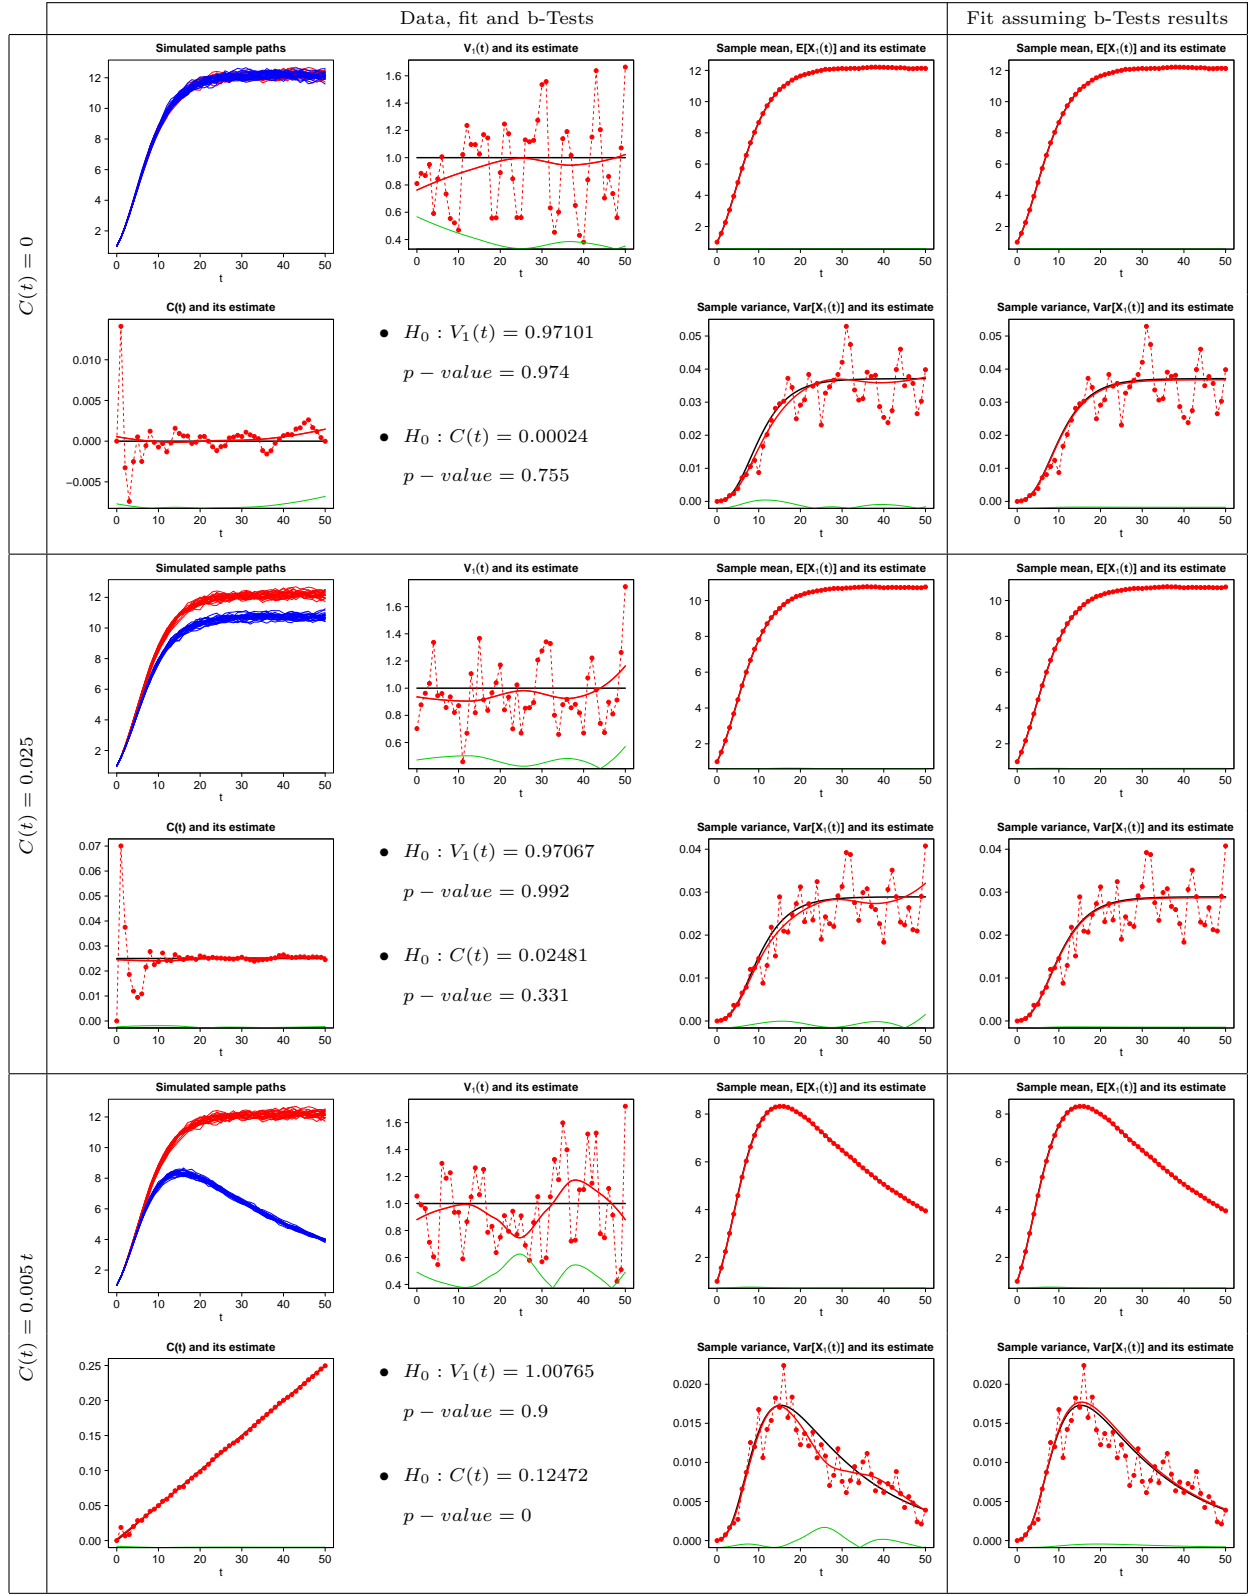

Table 1: Simulated data of the models (12) and (13) (in red and blue, respectively) with  $\alpha = 0.5$ ,  $\beta = 0.2$ ,  $\sigma = 0.01$ ,  $V_1(t) = 1$  and different types of functions  $C(t)$ ; estimates of  $C(t)$  and  $V_1(t)$  in model (13); concatenated bootstrap tests (b-Tests); and fit of simulated data of model (13).

|                 | Data, fit and b-Tests                                                                                                                                                      |                                                                                                                                                                                                                                                                                                 |                                                                                                                                                                              | Fit assuming b-Tests results                                                                                                                                                   |
|-----------------|----------------------------------------------------------------------------------------------------------------------------------------------------------------------------|-------------------------------------------------------------------------------------------------------------------------------------------------------------------------------------------------------------------------------------------------------------------------------------------------|------------------------------------------------------------------------------------------------------------------------------------------------------------------------------|--------------------------------------------------------------------------------------------------------------------------------------------------------------------------------|
| $C(t) = 0$      | 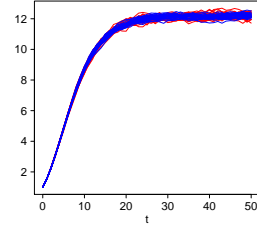<br>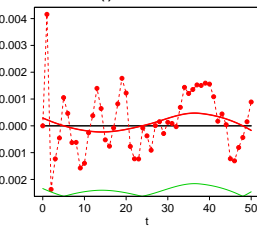     | 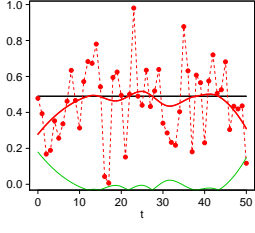<br><ul style="list-style-type: none"> <li>• <math>H_0 : V_1(t) = 0.47435</math><br/><math>p - value = 0.959</math></li> <li>• <math>H_0 : C(t) = 3e - 05</math><br/><math>p - value = 0.834</math></li> </ul> | 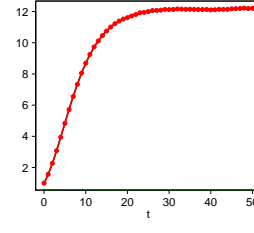<br>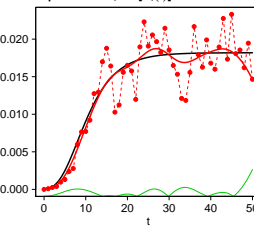     | 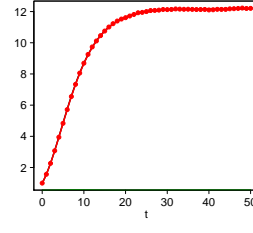<br>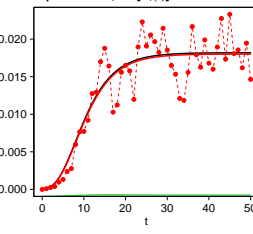     |
| $C(t) = 0.025$  | 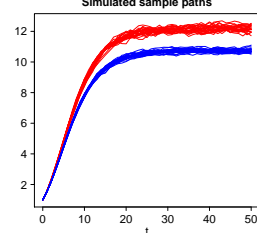<br>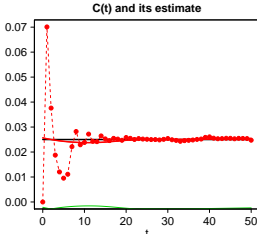   | 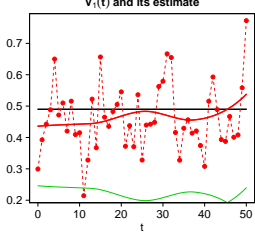<br><ul style="list-style-type: none"> <li>• <math>H_0 : V_1(t) = 0.47611</math><br/><math>p - value = 0.996</math></li> <li>• <math>H_0 : C(t) = 0.02485</math><br/><math>p - value = 0.334</math></li> </ul> | 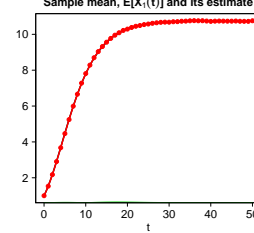<br>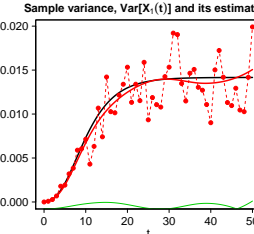   | 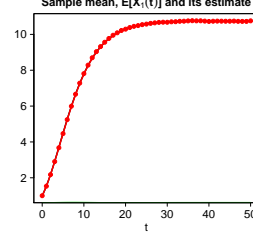<br>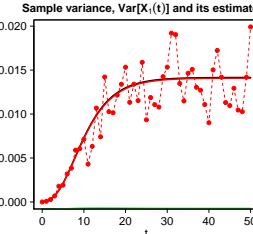   |
| $C(t) = 0.005t$ | 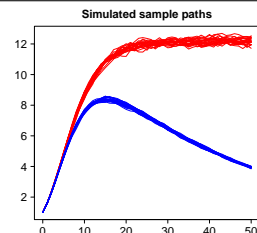<br>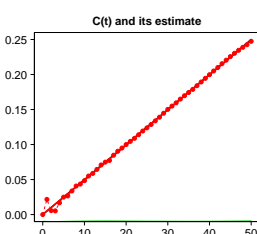 | 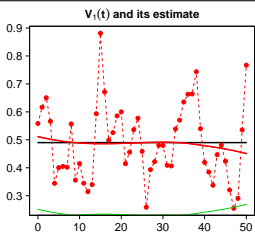<br><ul style="list-style-type: none"> <li>• <math>H_0 : V_1(t) = 0.48587</math><br/><math>p - value = 1</math></li> <li>• <math>H_0 : C(t) = 0.1244</math><br/><math>p - value = 0</math></li> </ul>        | 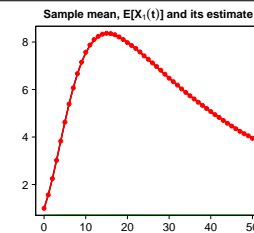<br>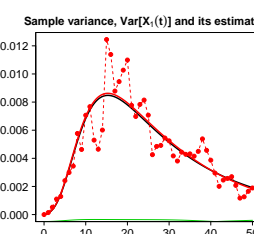 | 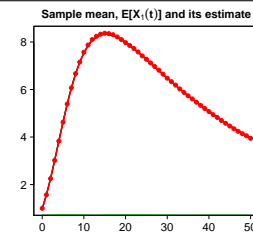<br>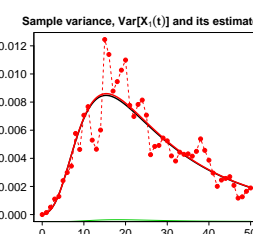 |

Table 2: Simulated data of the models (12) and (13) (in red and blue, respectively) with  $\alpha = 0.5$ ,  $\beta = 0.2$ ,  $\sigma = 0.01$ ,  $V_1(t) = 0.49$  and different types of functions  $C(t)$ ; estimates of  $C(t)$  and  $V_1(t)$  in model (13); concatenated bootstrap tests (b-Tests); and fit of simulated data of model (13).

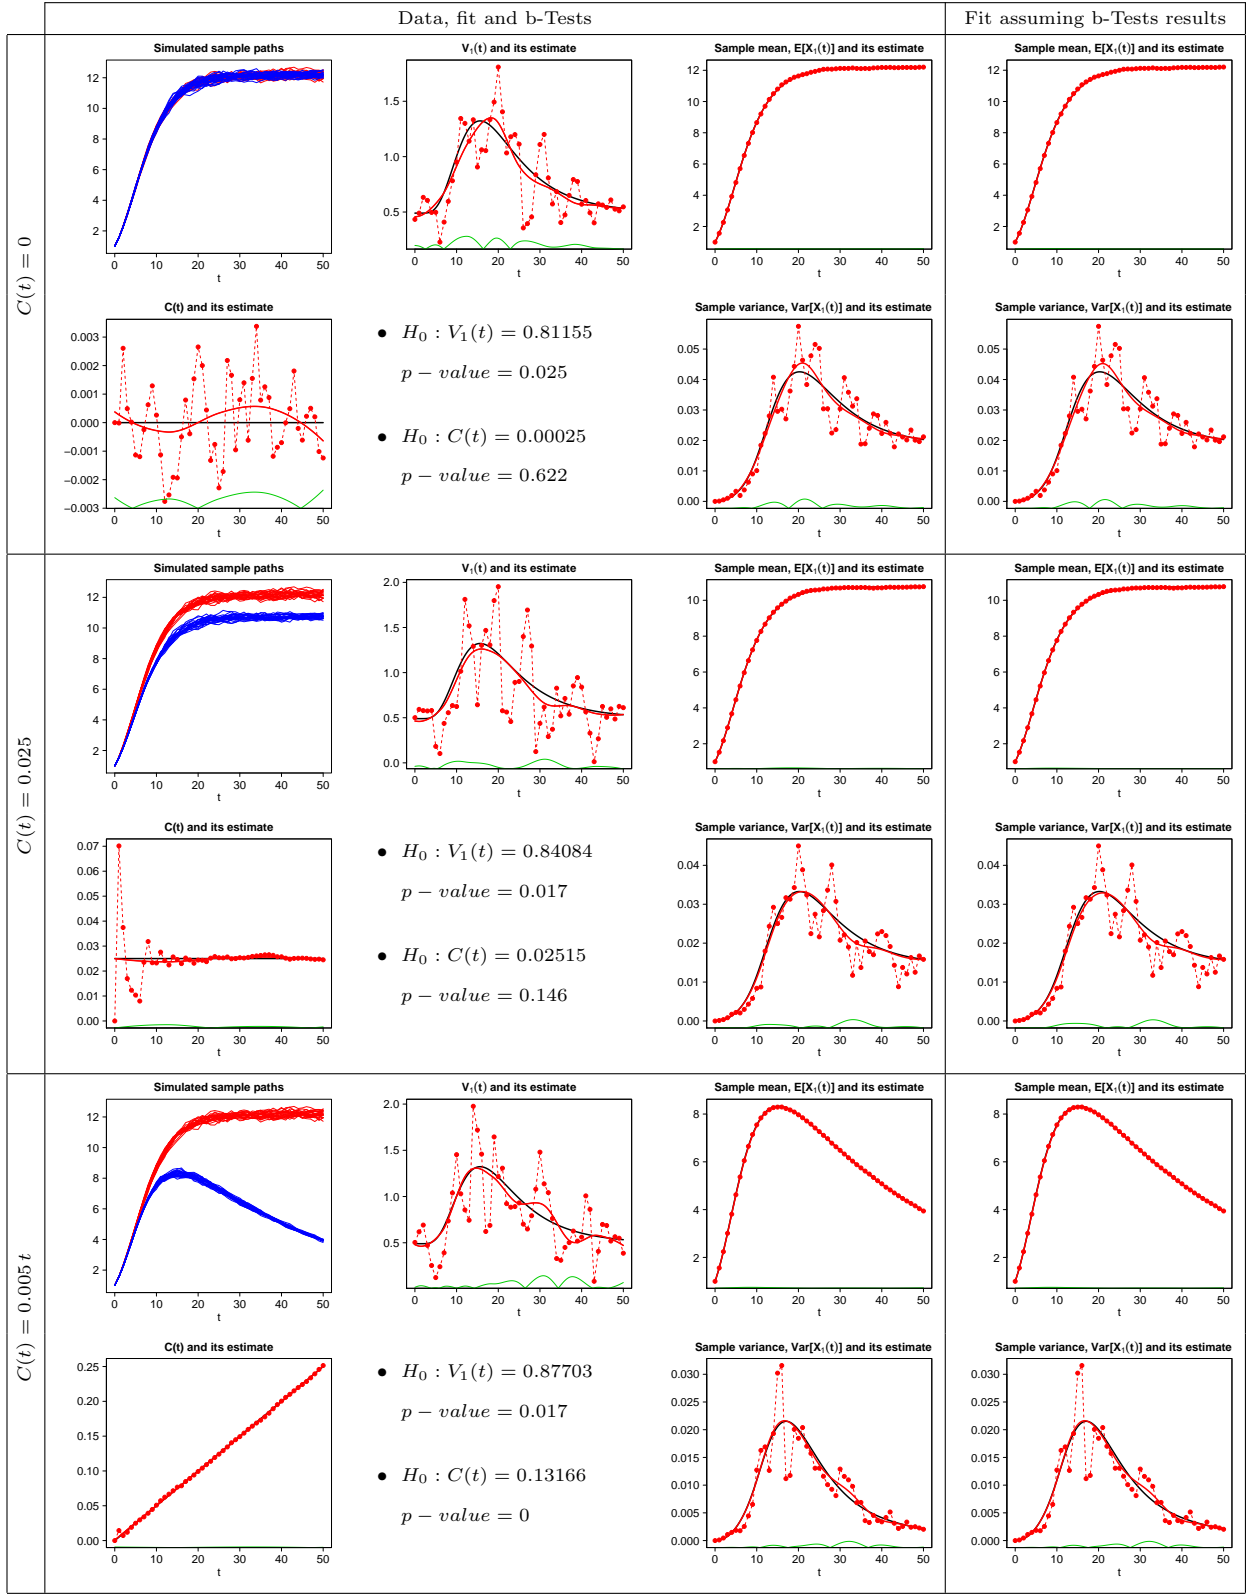

Table 3: Simulated data of the models (12) and (13) (in red and blue, respectively) with  $\alpha = 0.5$ ,  $\beta = 0.2$ ,  $\sigma = 0.01$ ,  $V_1(t) = (0.7 + 10\Lambda(t, 3, 0.5))^2$  and different types of functions  $C(t)$ ; estimates of  $C(t)$  and  $V_1(t)$  in model (13); concatenated bootstrap tests (b-Tests); and fit of simulated data of model (13).

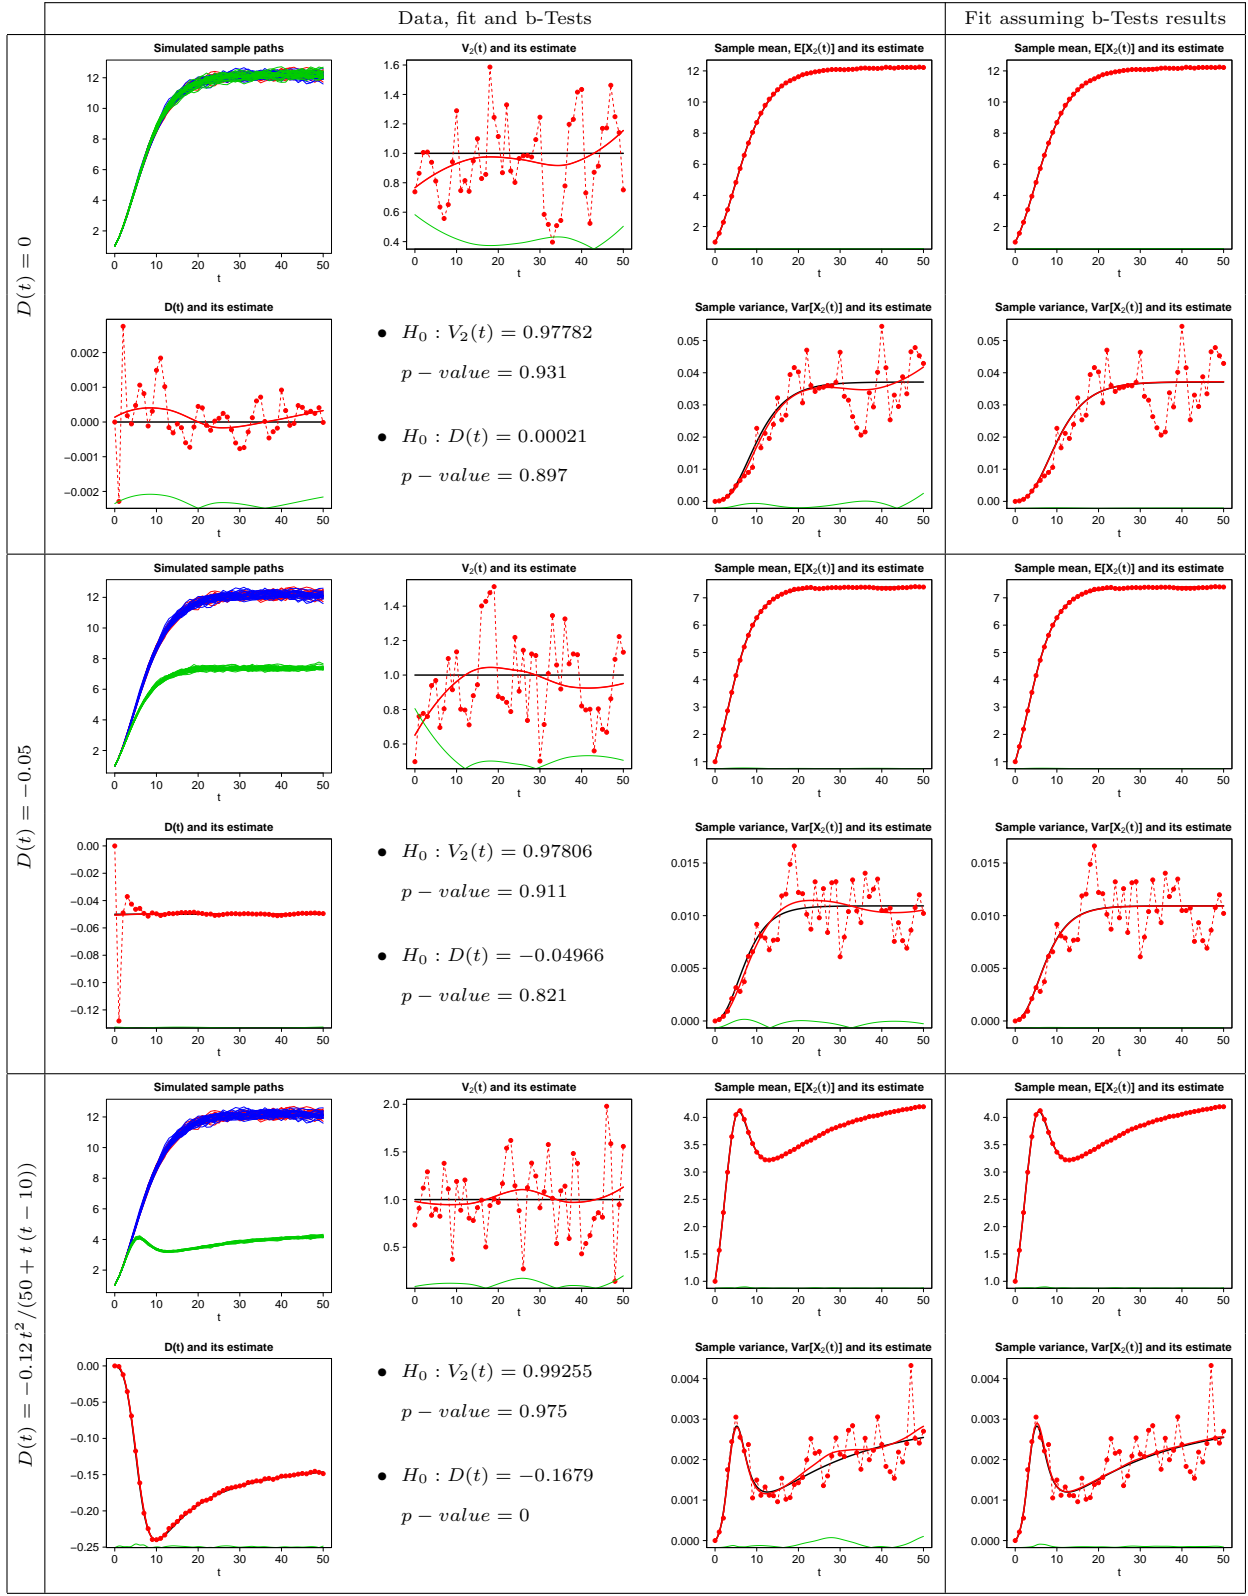

Table 4: Simulated data of the models (12), (13) and (15) (in red, blue and green, respectively) with  $\alpha = 0.5$ ,  $\beta = 0.2$ ,  $\sigma = 0.01$ ,  $V_1(t) = 1$ ,  $C(t) = 0$ ,  $V_2(t) = 1$  and different types of functions  $D(t)$ , estimates of  $D(t)$  and  $V_2(t)$  in model (15); concatenated bootstrap tests (b-Tests); and fit of simulated data of model (15).

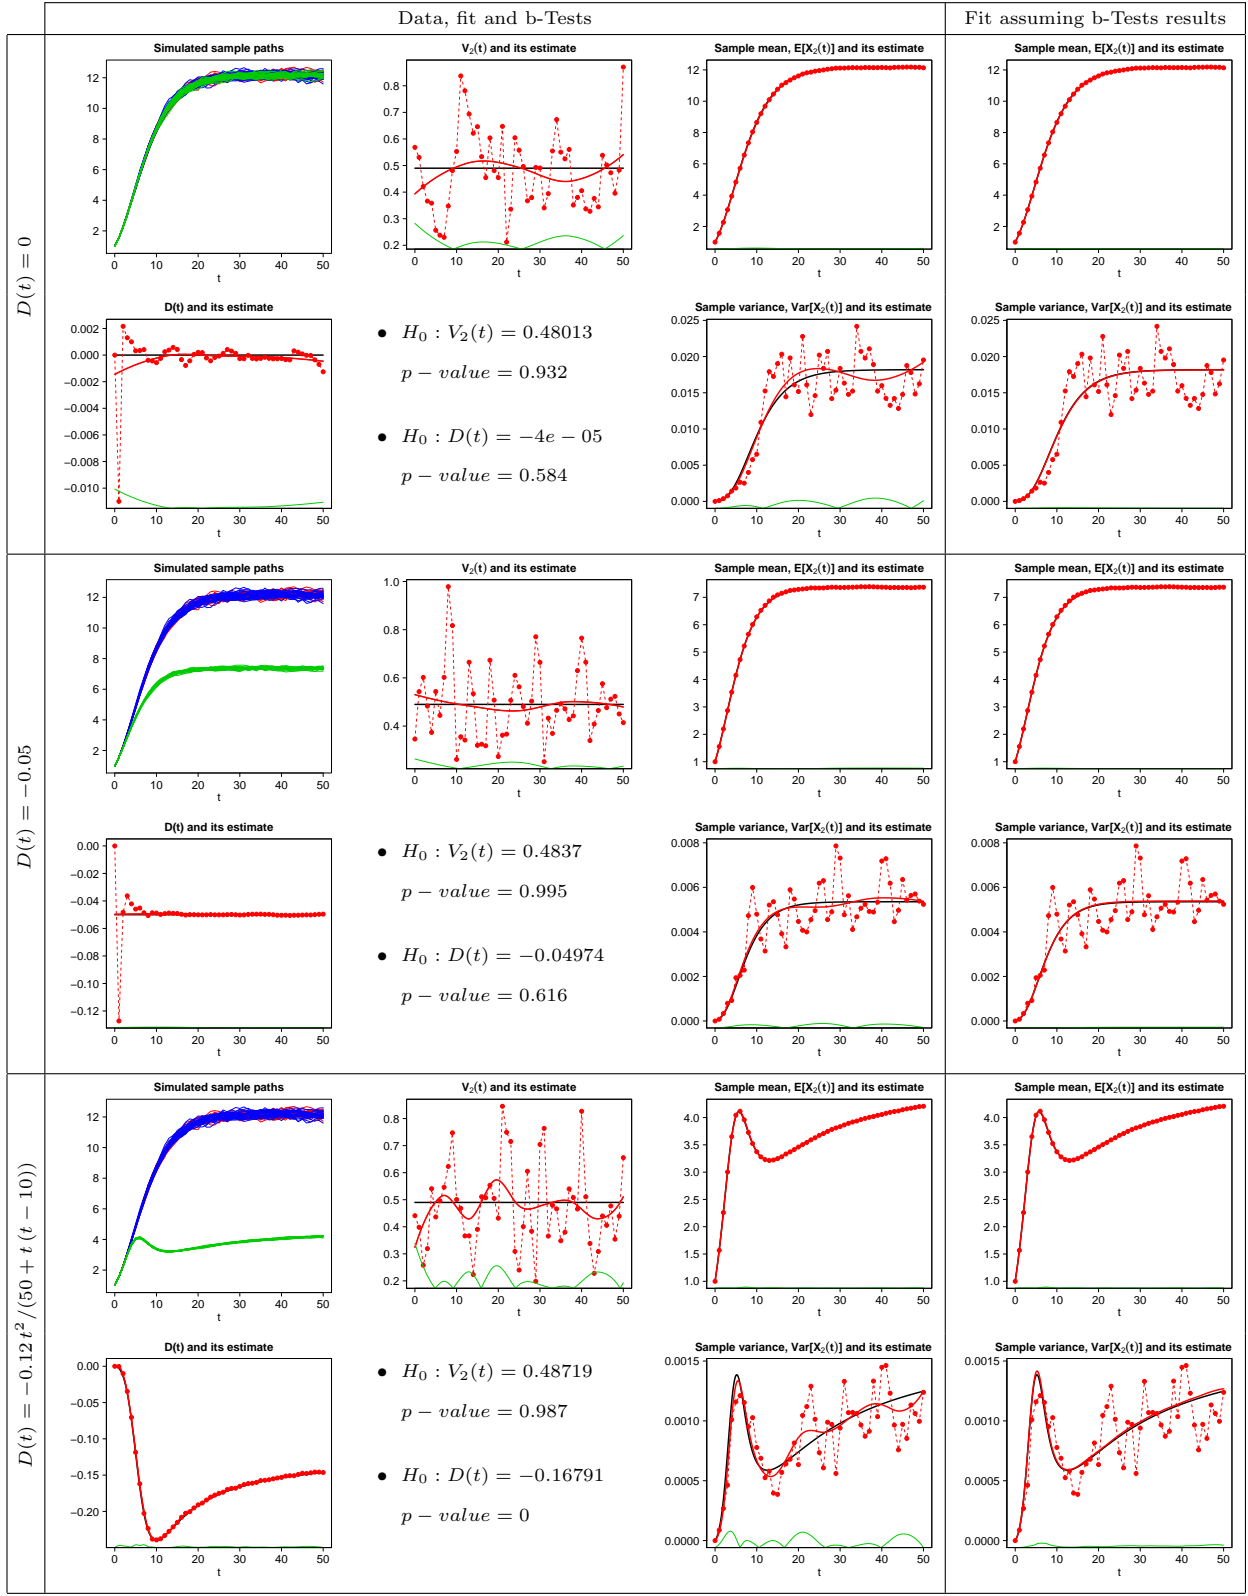

Table 5: Simulated data of the models (12), (13) and (15) (in red, blue and green, respectively) with  $\alpha = 0.5$ ,  $\beta = 0.2$ ,  $\sigma = 0.01$ ,  $V_1(t) = 1$ ,  $C(t) = 0$ ,  $V_2(t) = 0.49$  and different types of functions  $D(t)$ , estimates of  $D(t)$  and  $V_2(t)$  in model (15); concatenated bootstrap tests (b-Tests); and fit of simulated data of model (15).

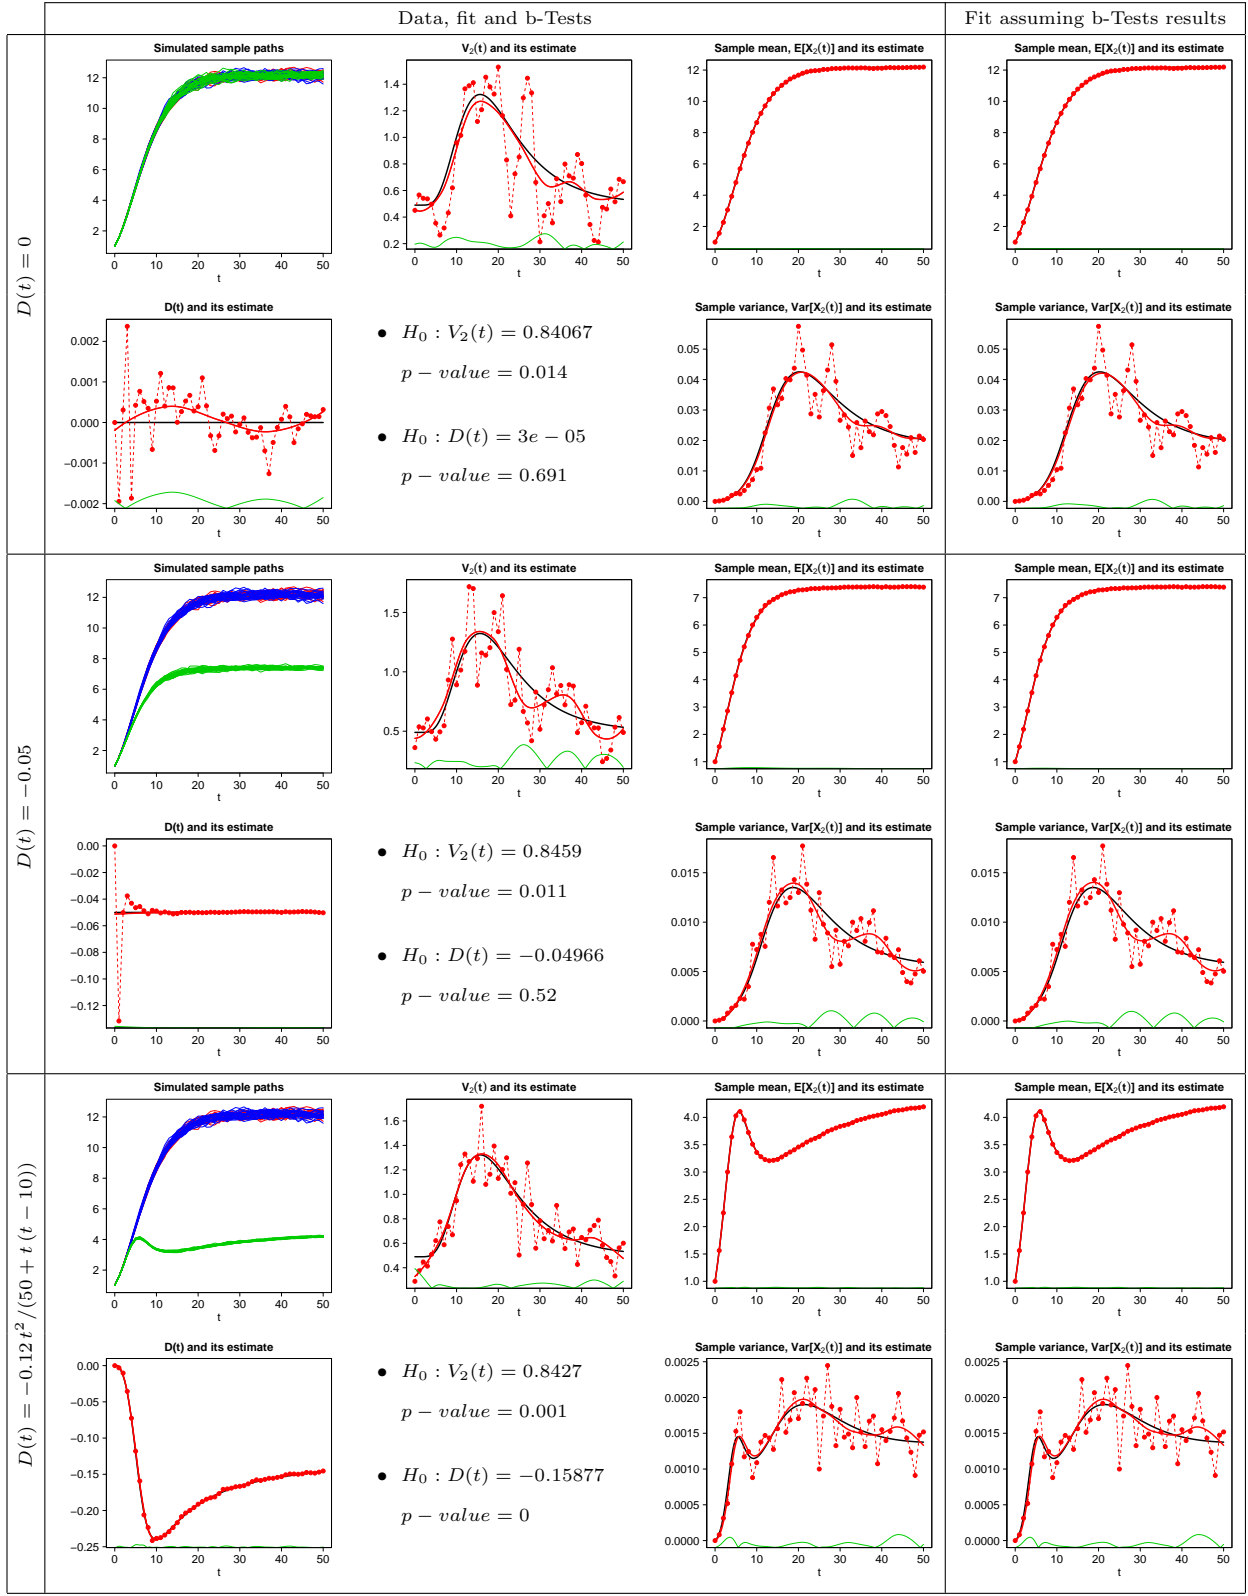

Table 6: Simulated data of the models (12), (13) and (15) (in red, blue and green, respectively) with  $\alpha = 0.5$ ,  $\beta = 0.2$ ,  $\sigma = 0.01$ ,  $V_1(t) = 1$ ,  $C(t) = 0$ ,  $V_2(t) = (0.7 + 10\Lambda(t, 3, 0.5))^2$  and different types of functions  $D(t)$ , estimates of  $D(t)$  and  $V_2(t)$  in model (15); concatenated bootstrap tests (b-Tests); and fit of simulated data of model (15).

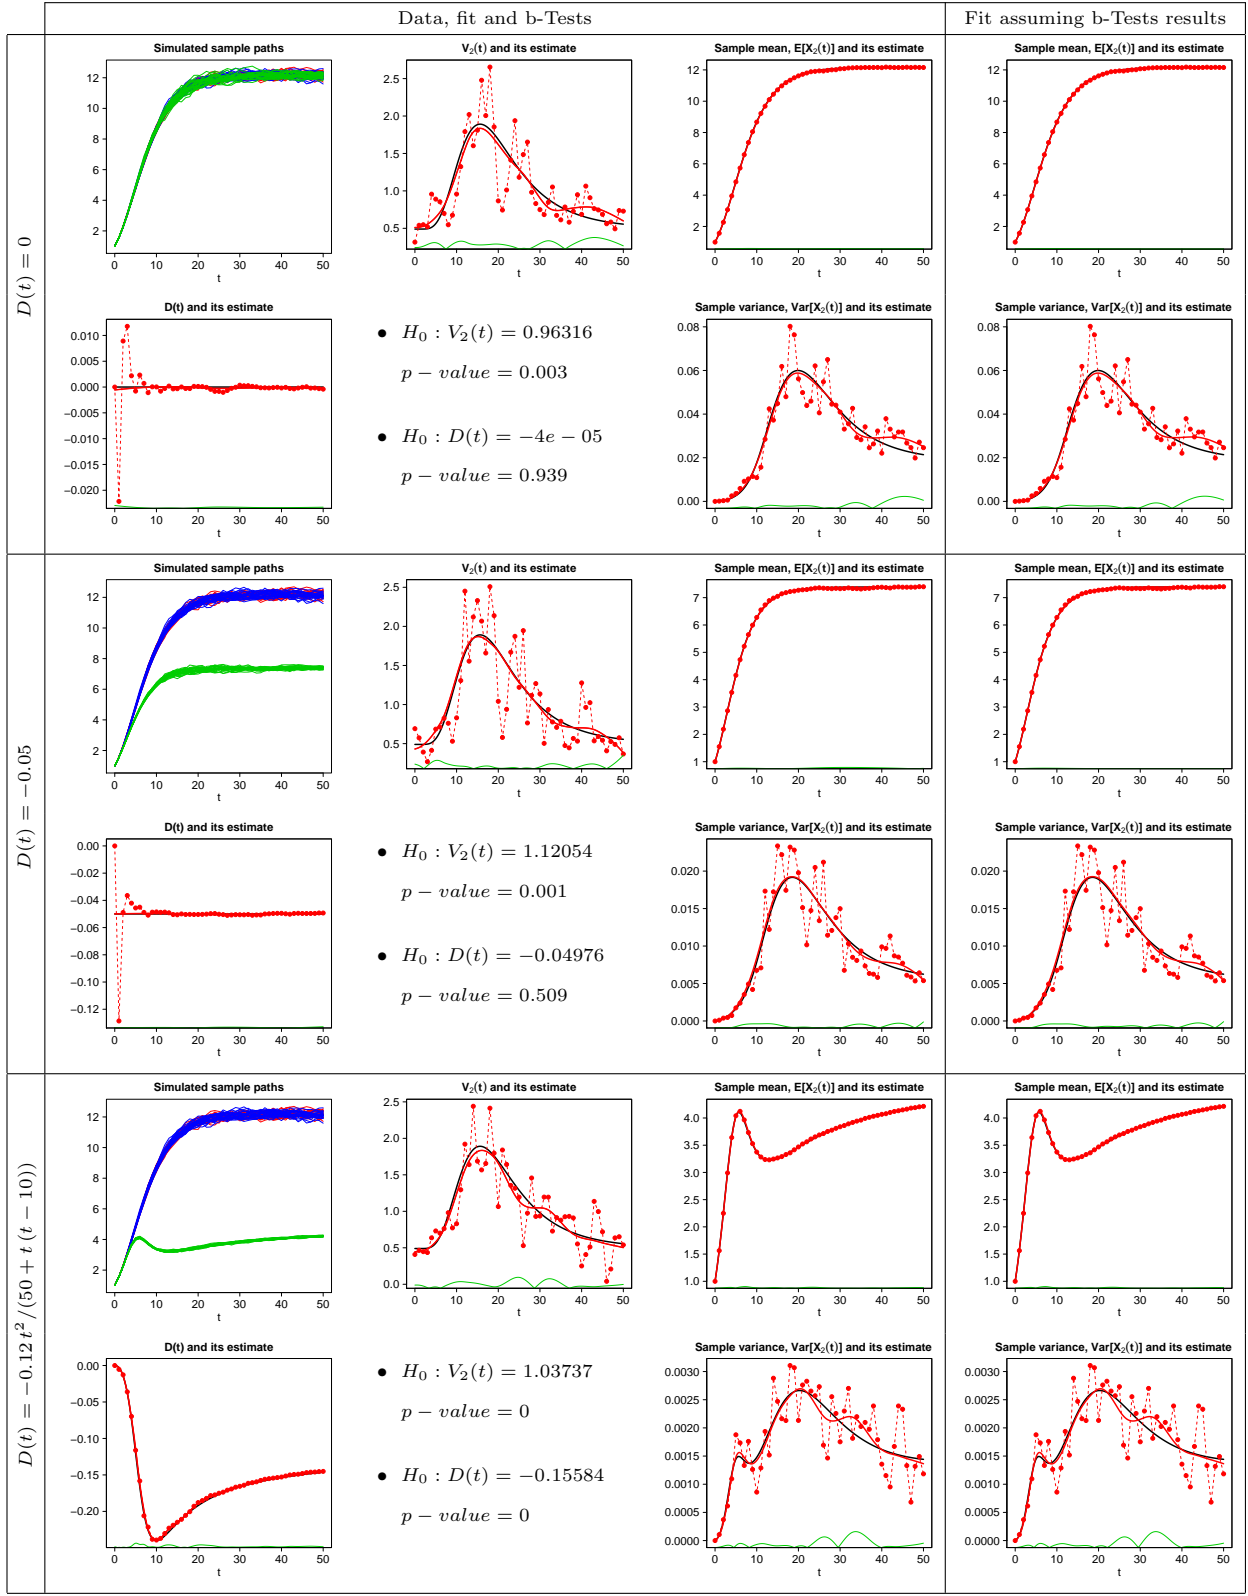

Table 7: Simulated data of the models (12), (13) and (15) (in red, blue and green, respectively) with  $\alpha = 0.5$ ,  $\beta = 0.2$ ,  $\sigma = 0.01$ ,  $V_1(t) = 1$ ,  $C(t) = 0$ ,  $V_2(t) = (0.7 + 15\Lambda(t, 3, 0.5))^2$  and different types of functions  $D(t)$ , estimates of  $D(t)$  and  $V_2(t)$  in model (15); concatenated bootstrap tests (b-Tests); and fit of simulated data of model (15).

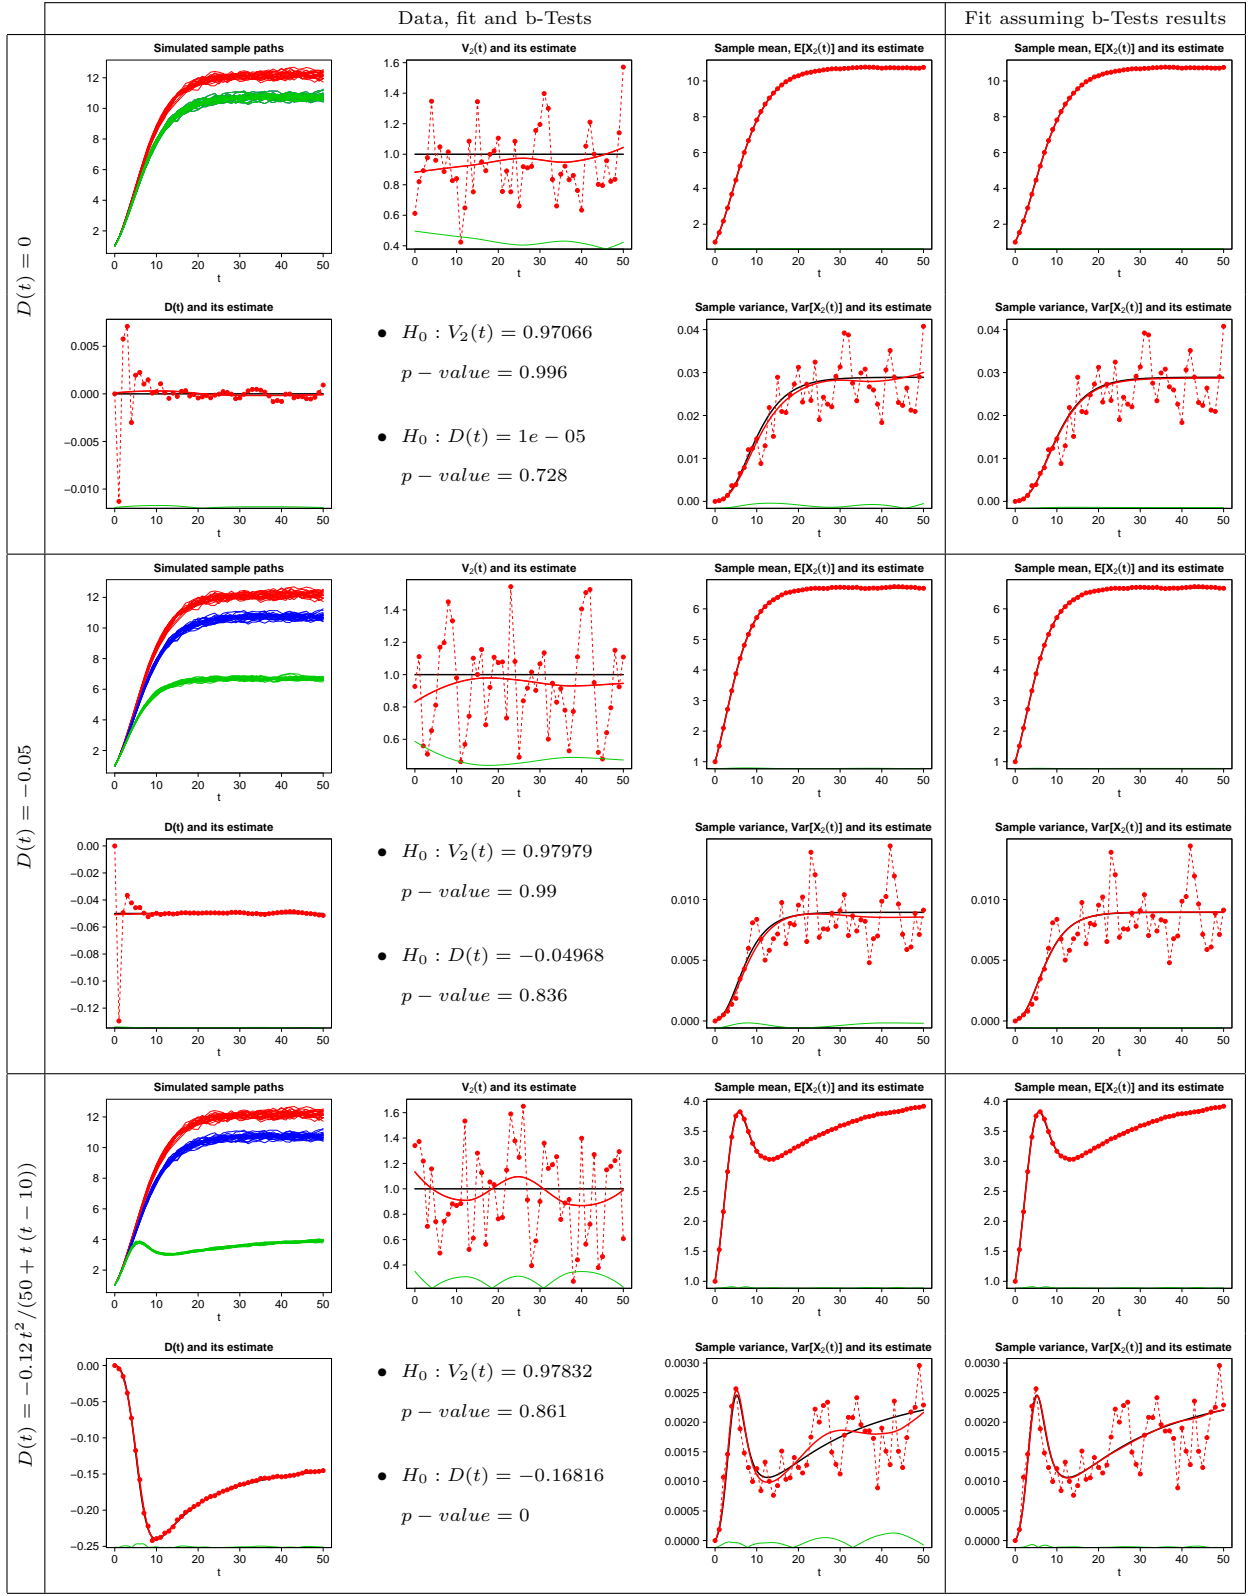

Table 8: Simulated data of the models (12), (13) and (15) (in red, blue and green, respectively) with  $\alpha = 0.5$ ,  $\beta = 0.2$ ,  $\sigma = 0.01$ ,  $V_1(t) = 1$ ,  $C(t) = 0.025$ ,  $V_2(t) = 1$  and different types of functions  $D(t)$ , estimates of  $D(t)$  and  $V_2(t)$  in model (15); concatenated bootstrap tests (b-Tests); and fit of simulated data of model (15).

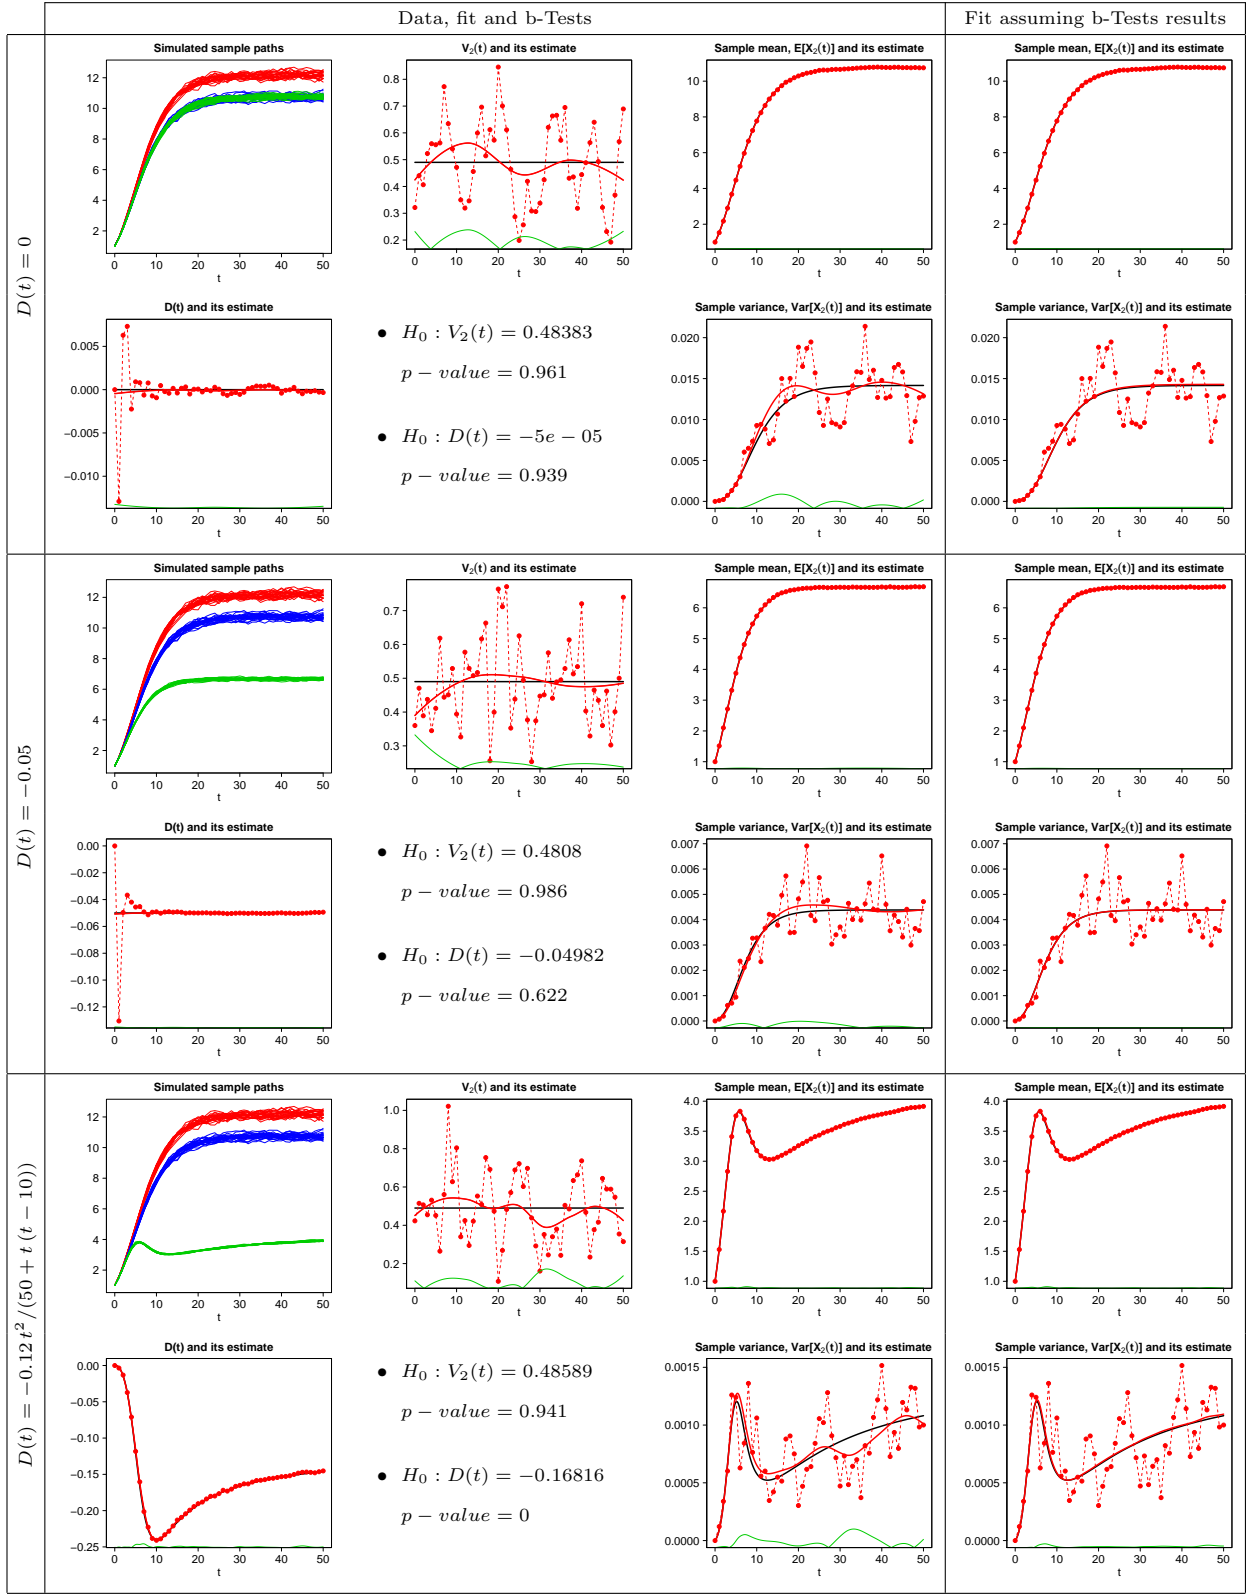

Table 9: Simulated data of the models (12), (13) and (15) (in red, blue and green, respectively) with  $\alpha = 0.5$ ,  $\beta = 0.2$ ,  $\sigma = 0.01$ ,  $V_1(t) = 1$ ,  $C(t) = 0.025$ ,  $V_2(t) = 0.49$  and different types of functions  $D(t)$ , estimates of  $D(t)$  and  $V_2(t)$  in model (15); concatenated bootstrap tests (b-Tests); and fit of simulated data of model (15).

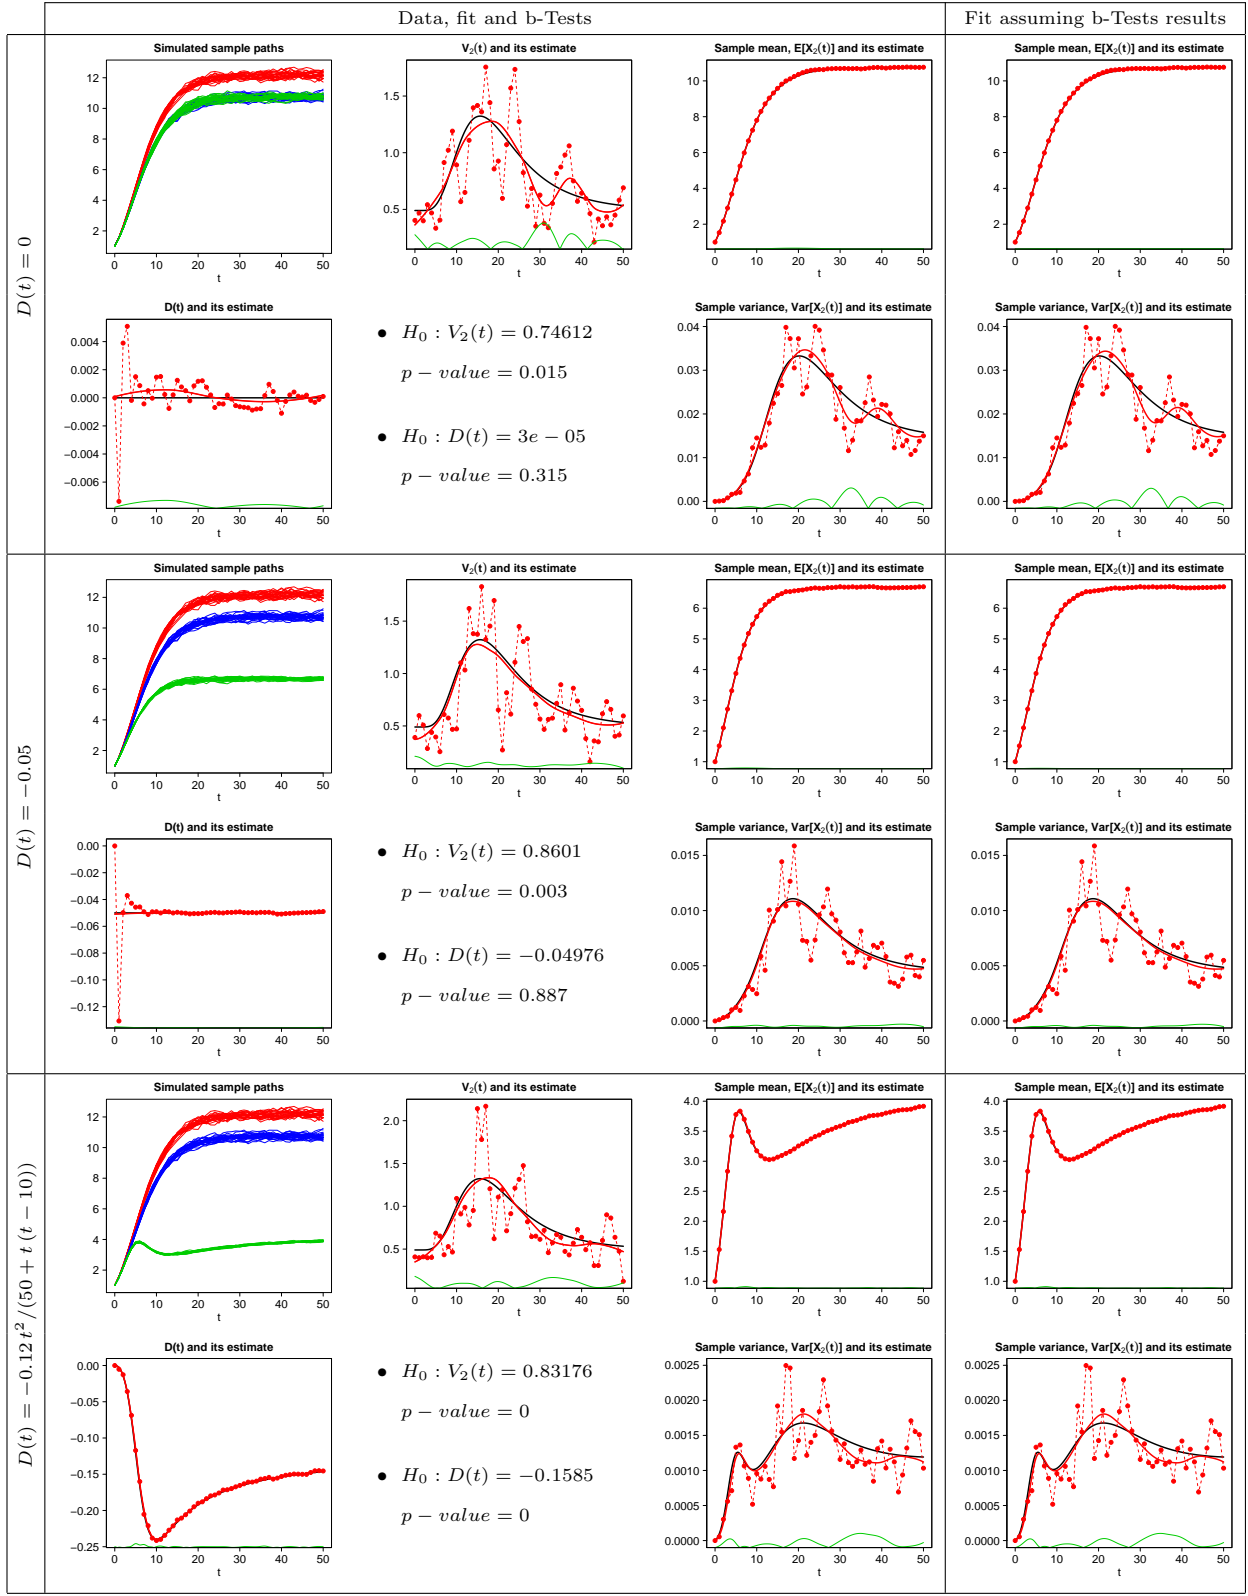

Table 10: Simulated data of the models (12), (13) and (15) (in red, blue and green, respectively) with  $\alpha = 0.5$ ,  $\beta = 0.2$ ,  $\sigma = 0.01$ ,  $V_1(t) = 1$ ,  $C(t) = 0.025$ ,  $V_2(t) = (0.7 + 10\Lambda(t, 3, 0.5))^2$  and different types of functions  $D(t)$ , estimates of  $D(t)$  and  $V_2(t)$  in model (15); concatenated bootstrap tests (b-Tests); and fit of simulated data of model (15).

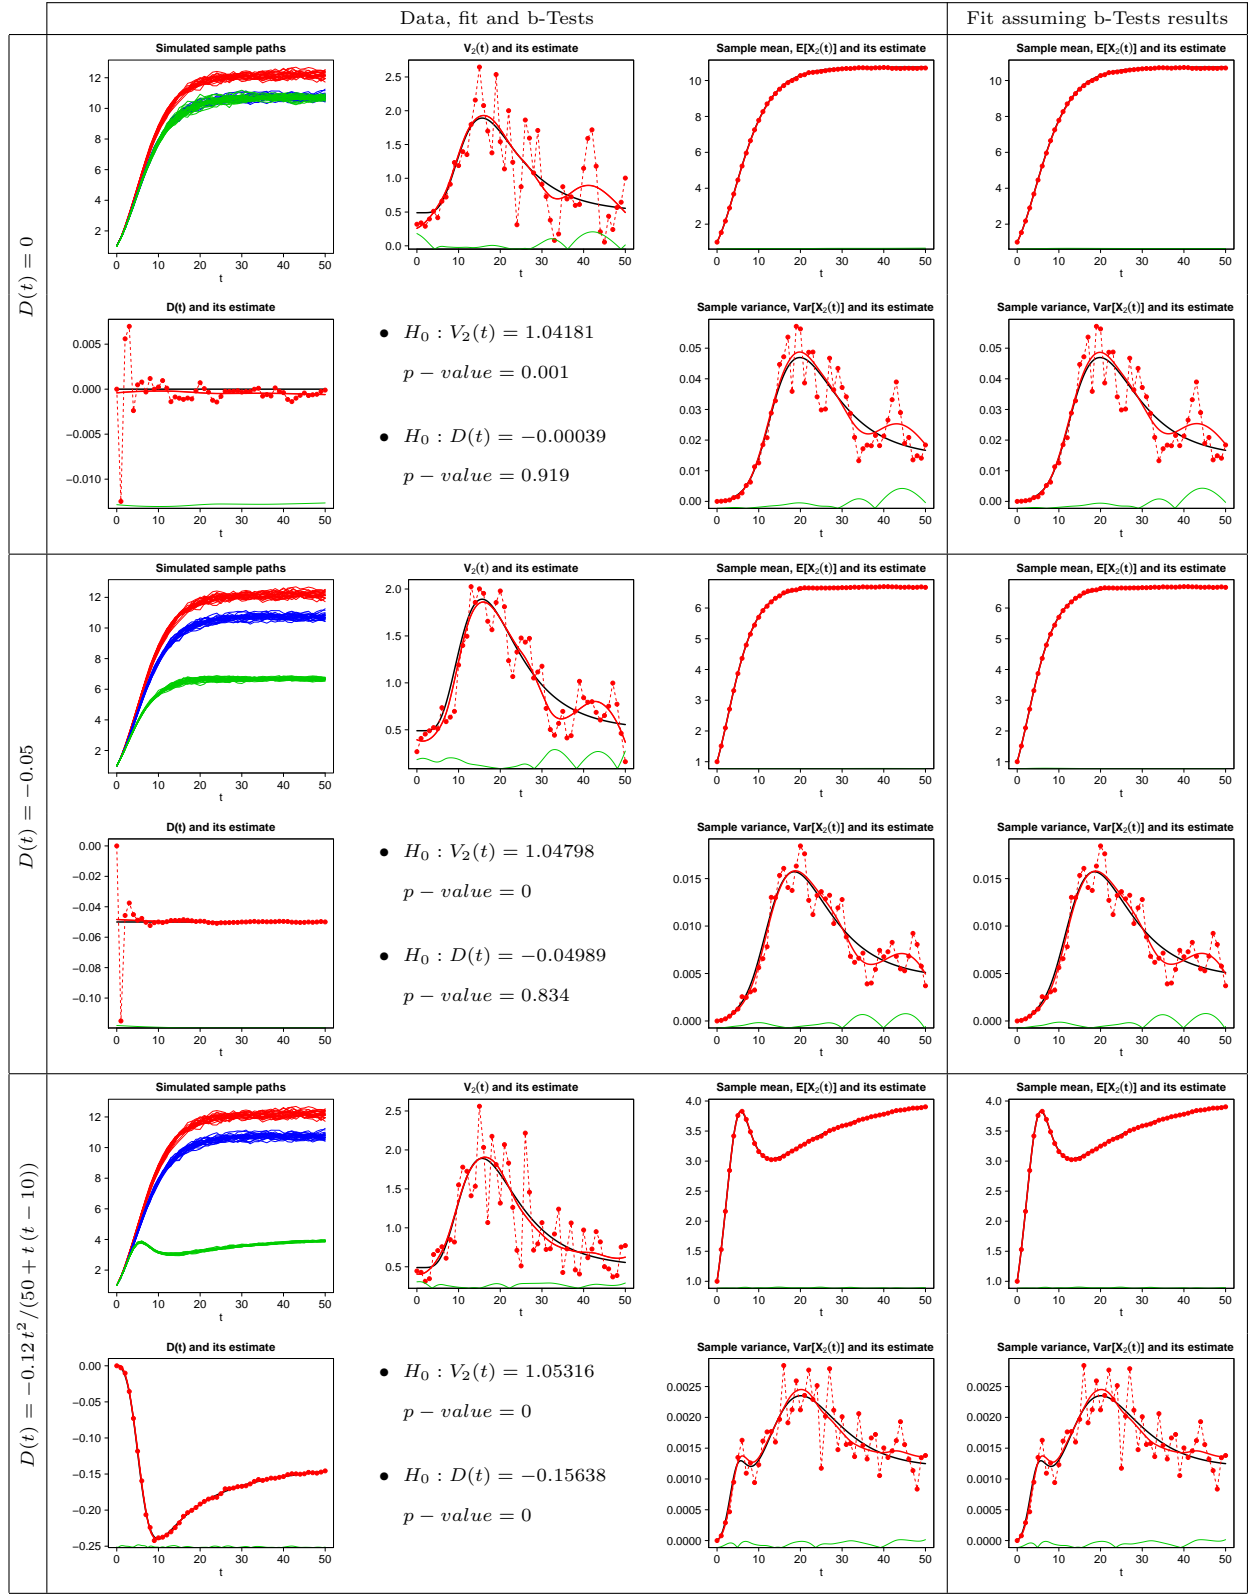

Table 11: Simulated data of the models (12), (13) and (15) (in red, blue and green, respectively) with  $\alpha = 0.5$ ,  $\beta = 0.2$ ,  $\sigma = 0.01$ ,  $V_1(t) = 1$ ,  $C(t) = 0.025$ ,  $V_2(t) = (0.7 + 15\Lambda(t, 3, 0.5))^2$  and different types of functions  $D(t)$ , estimates of  $D(t)$  and  $V_2(t)$  in model (15); concatenated bootstrap tests (b-Tests); and fit of simulated data of model (15).

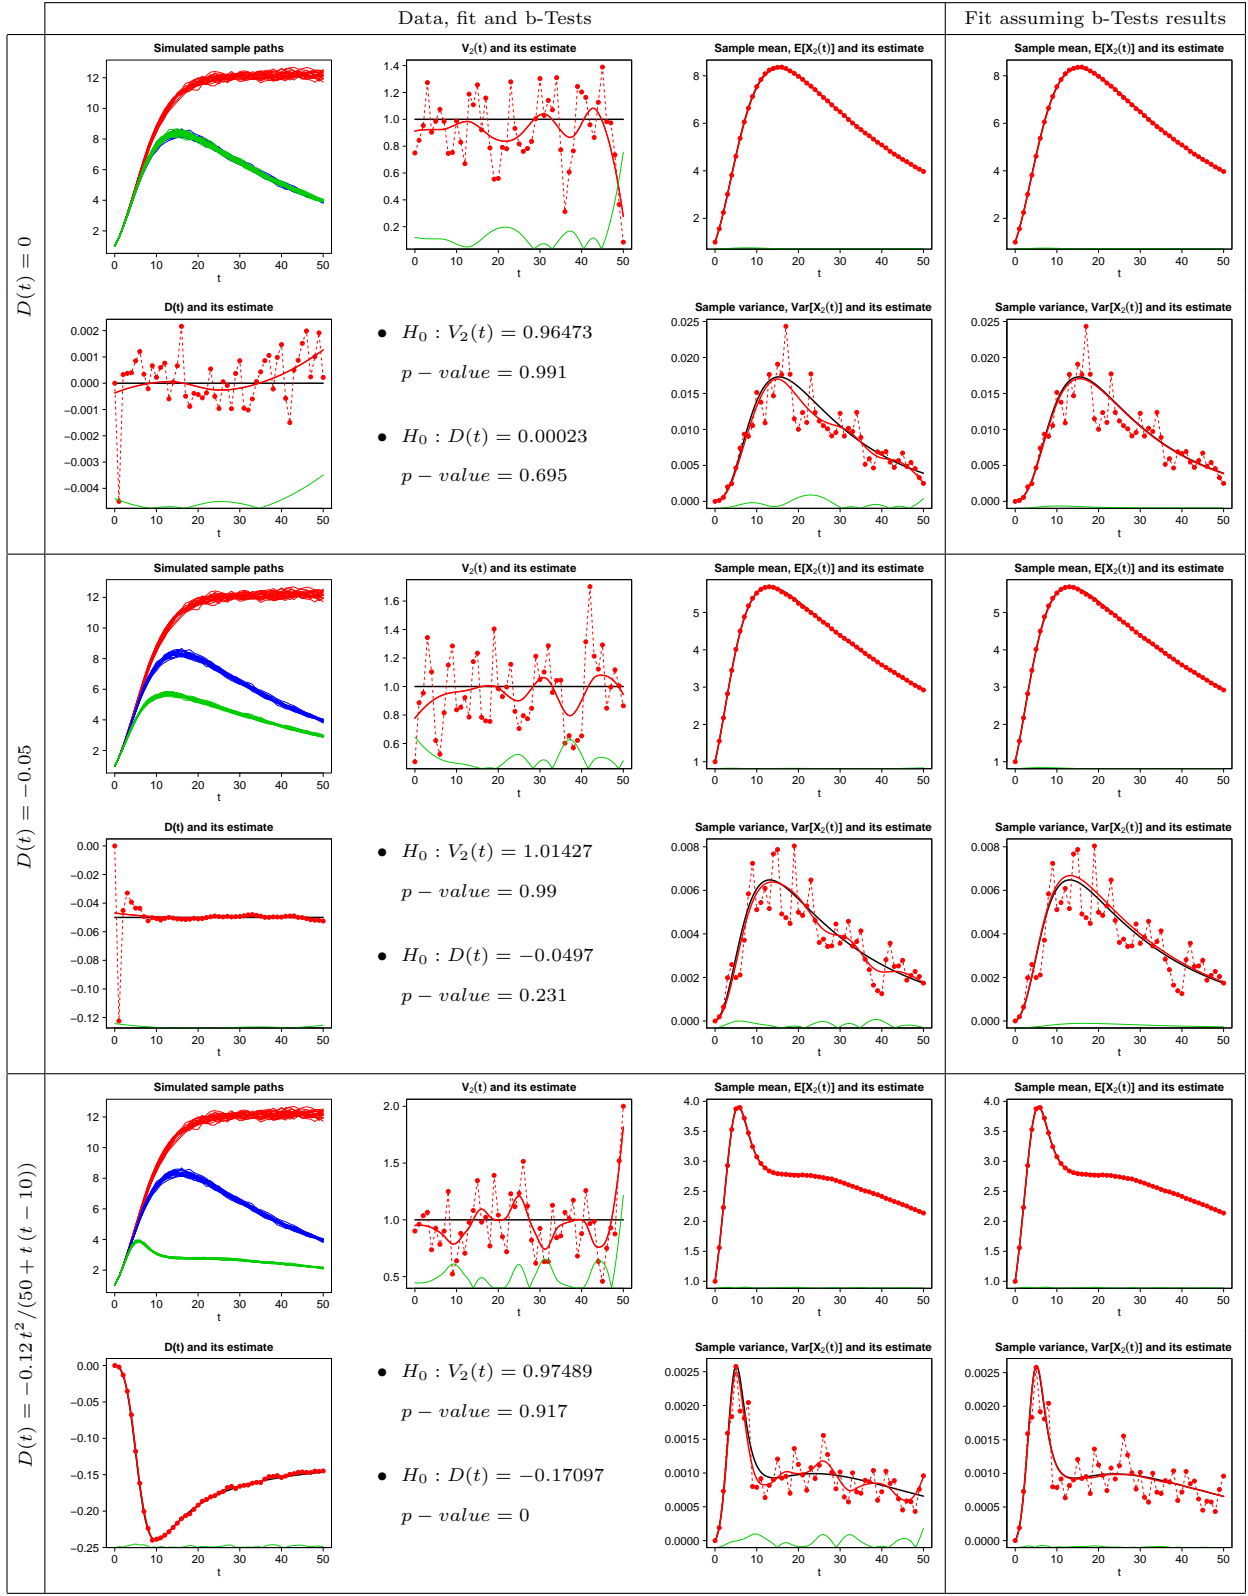

Table 12: Simulated data of the models (12), (13) and (15) (in red, blue and green, respectively) with  $\alpha = 0.5$ ,  $\beta = 0.2$ ,  $\sigma = 0.01$ ,  $V_1(t) = 1$ ,  $C(t) = 0.005t$ ,  $V_2(t) = 1$  and different types of functions  $D(t)$ , estimates of  $D(t)$  and  $V_2(t)$  in model (15); concatenated bootstrap tests (b-Tests); and fit of simulated data of model (15).

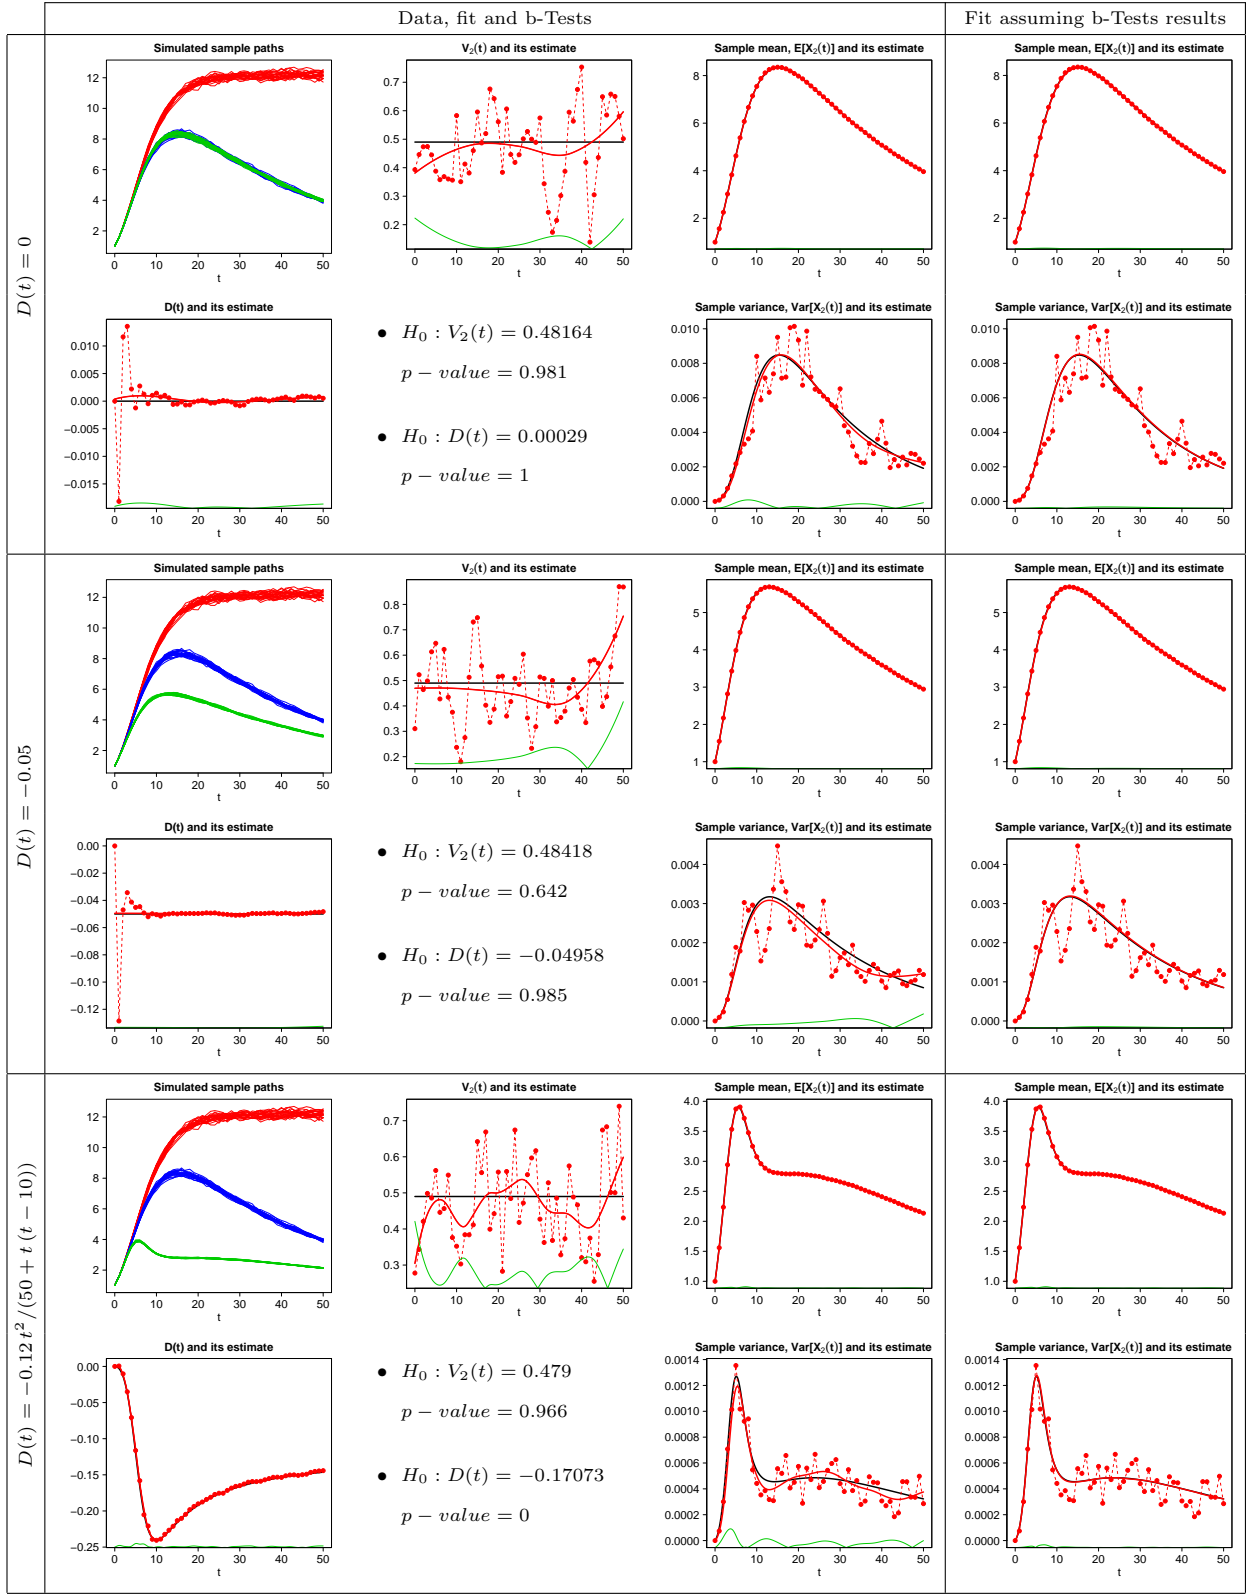

Table 13: Simulated data of the models (12), (13) and (15) (in red, blue and green, respectively) with  $\alpha = 0.5$ ,  $\beta = 0.2$ ,  $\sigma = 0.01$ ,  $V_1(t) = 1$ ,  $C(t) = 0.005t$ ,  $V_2(t) = 0.49$  and different types of functions  $D(t)$ , estimates of  $D(t)$  and  $V_2(t)$  in model (15); concatenated bootstrap tests (b-Tests); and fit of simulated data of model (15).

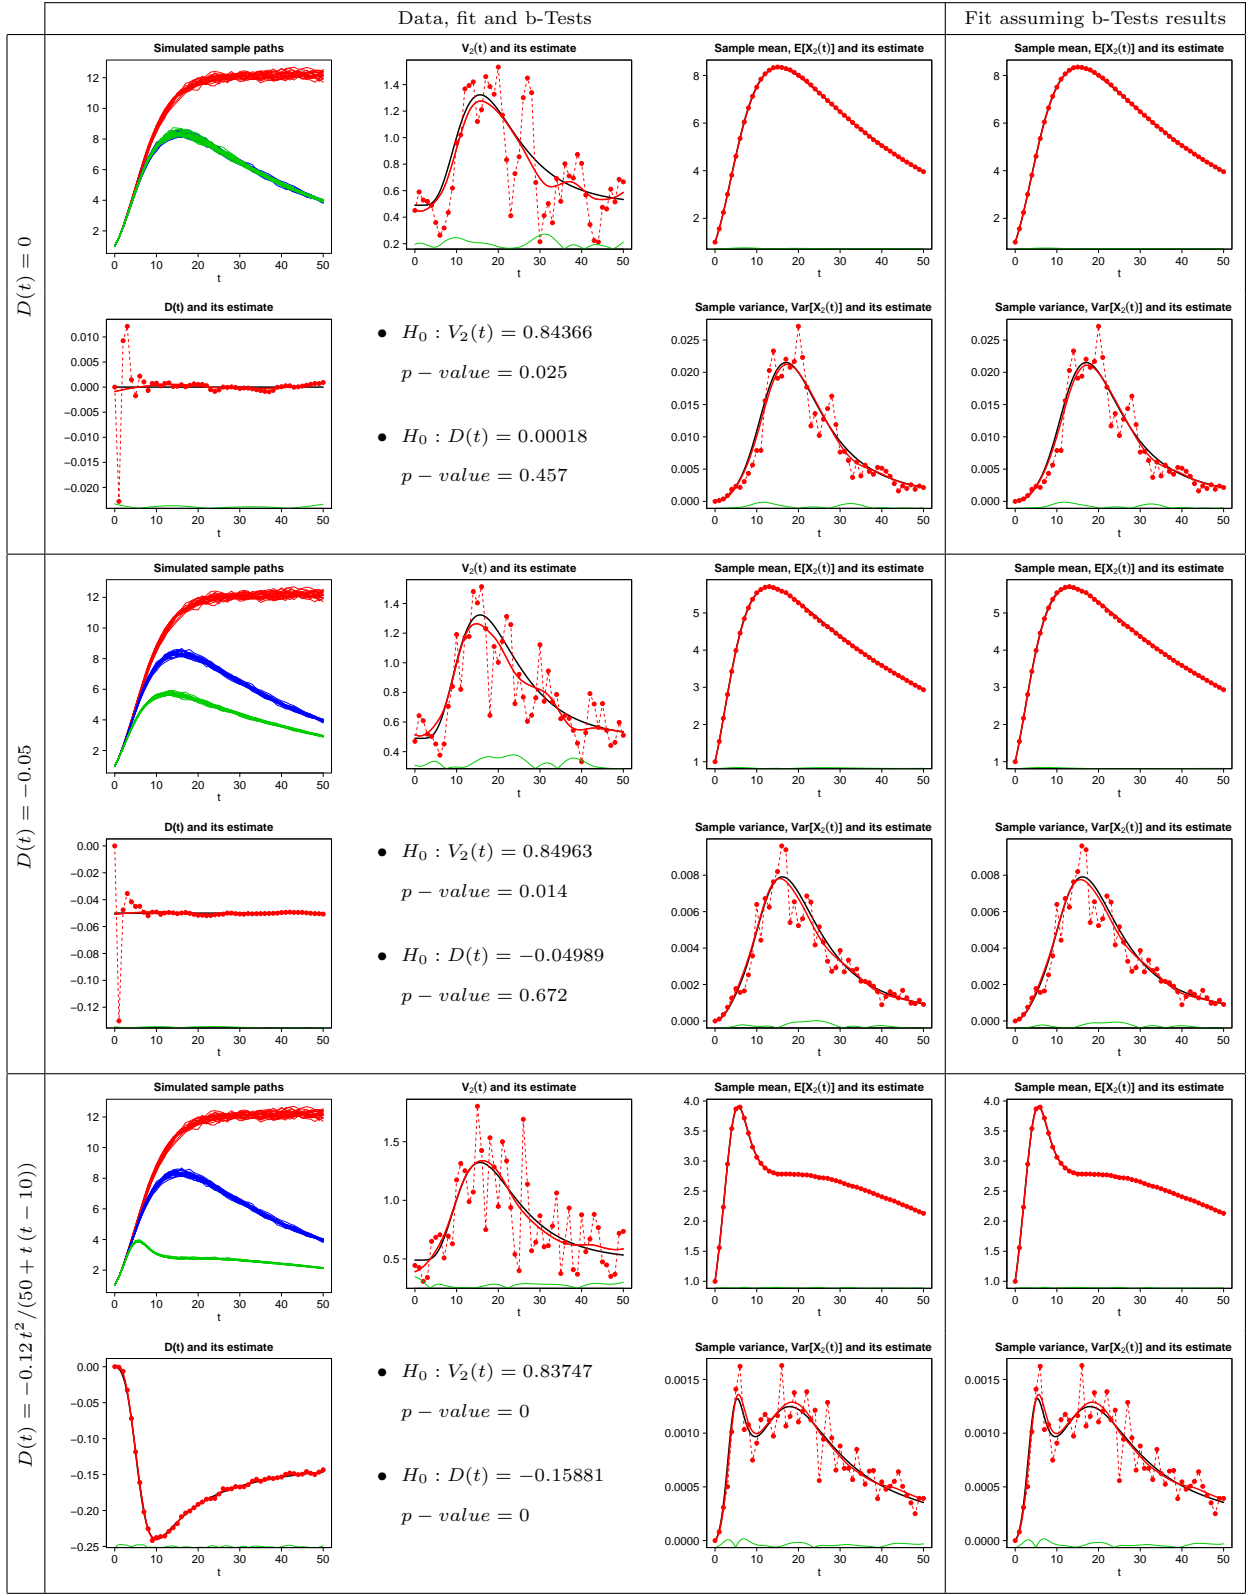

Table 14: Simulated data of the models (12), (13) and (15) (in red, blue and green, respectively) with  $\alpha = 0.5$ ,  $\beta = 0.2$ ,  $\sigma = 0.01$ ,  $V_1(t) = 1$ ,  $C(t) = 0.005t$ ,  $V_2(t) = (0.7 + 10\Lambda(t, 3, 0.5))^2$  and different types of functions  $D(t)$ , estimates of  $D(t)$  and  $V_2(t)$  in model (15); concatenated bootstrap tests (b-Tests); and fit of simulated data of model (15).

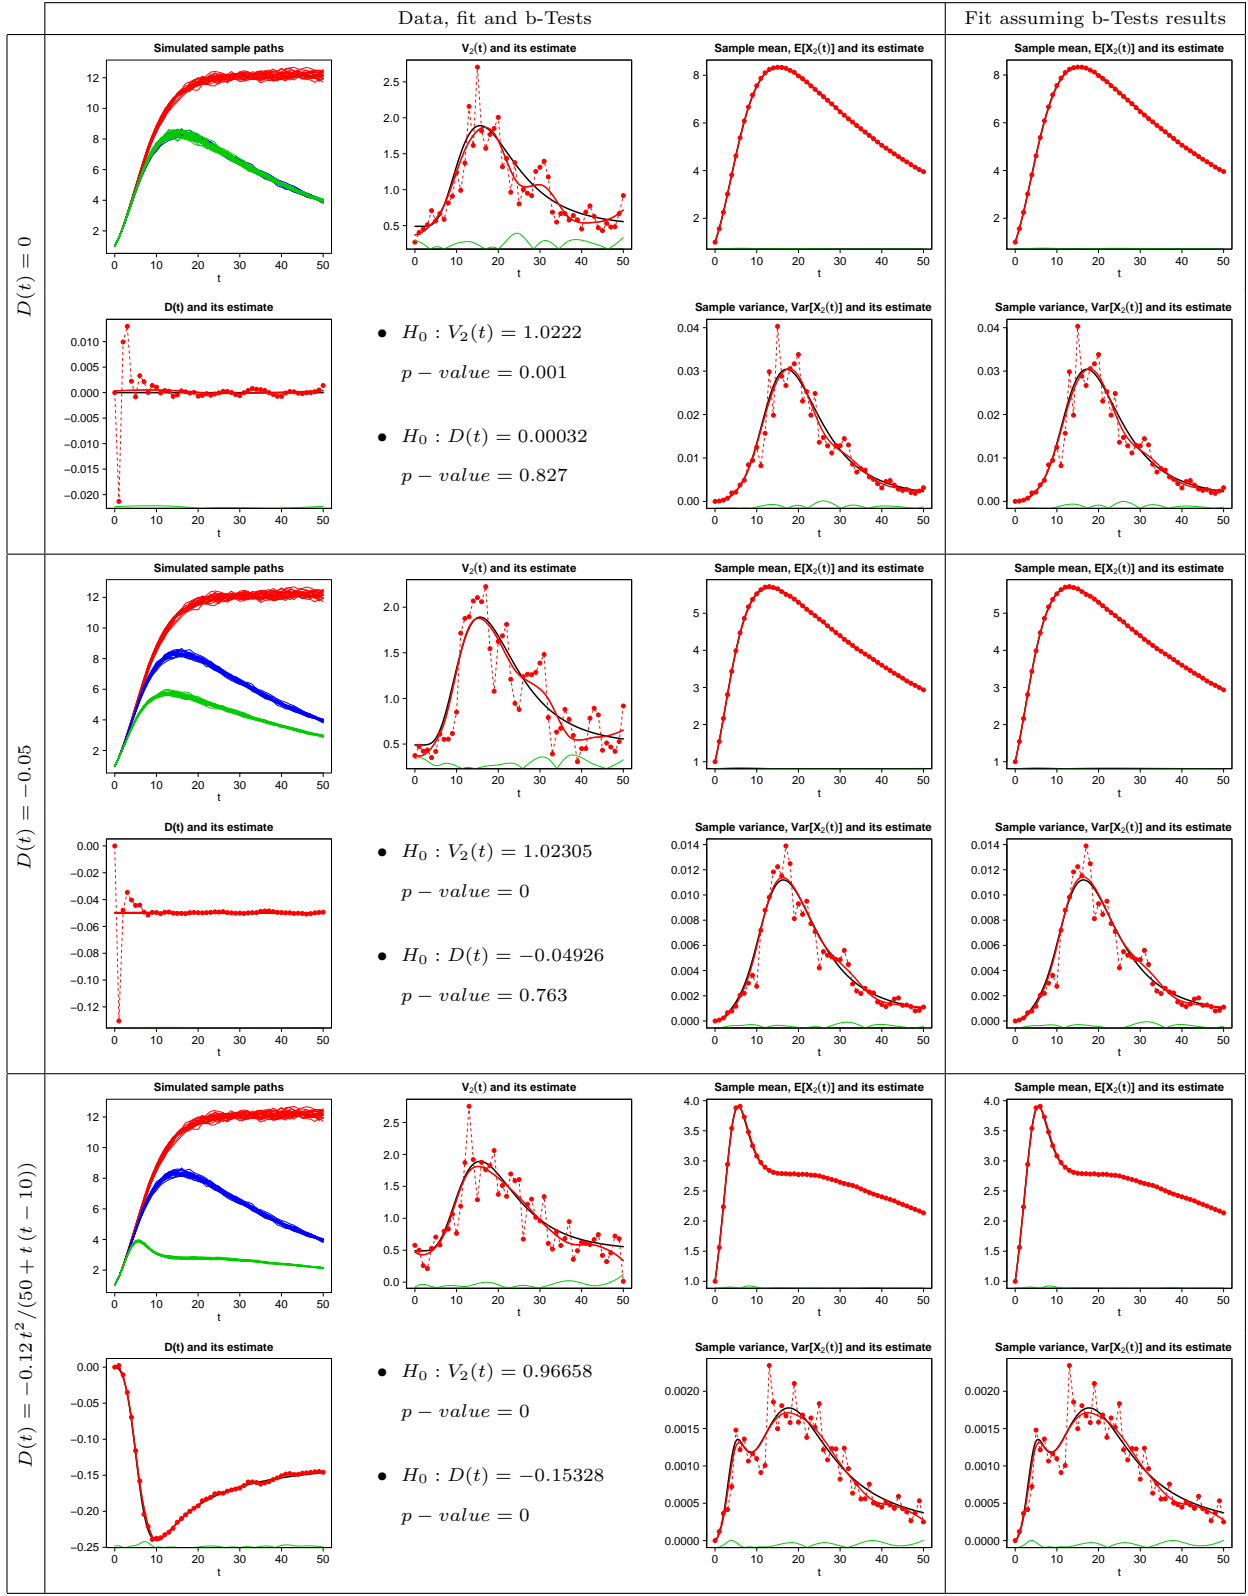

Table 15: Simulated data of the models (12), (13) and (15) (in red, blue and green, respectively) with  $\alpha = 0.5$ ,  $\beta = 0.2$ ,  $\sigma = 0.01$ ,  $V_1(t) = 1$ ,  $C(t) = 0.005t$ ,  $V_2(t) = (0.7 + 15\Lambda(t, 3, 0.5))^2$  and different types of functions  $D(t)$ , estimates of  $D(t)$  and  $V_2(t)$  in model (15); concatenated bootstrap tests (b-Tests); and fit of simulated data of model (15).

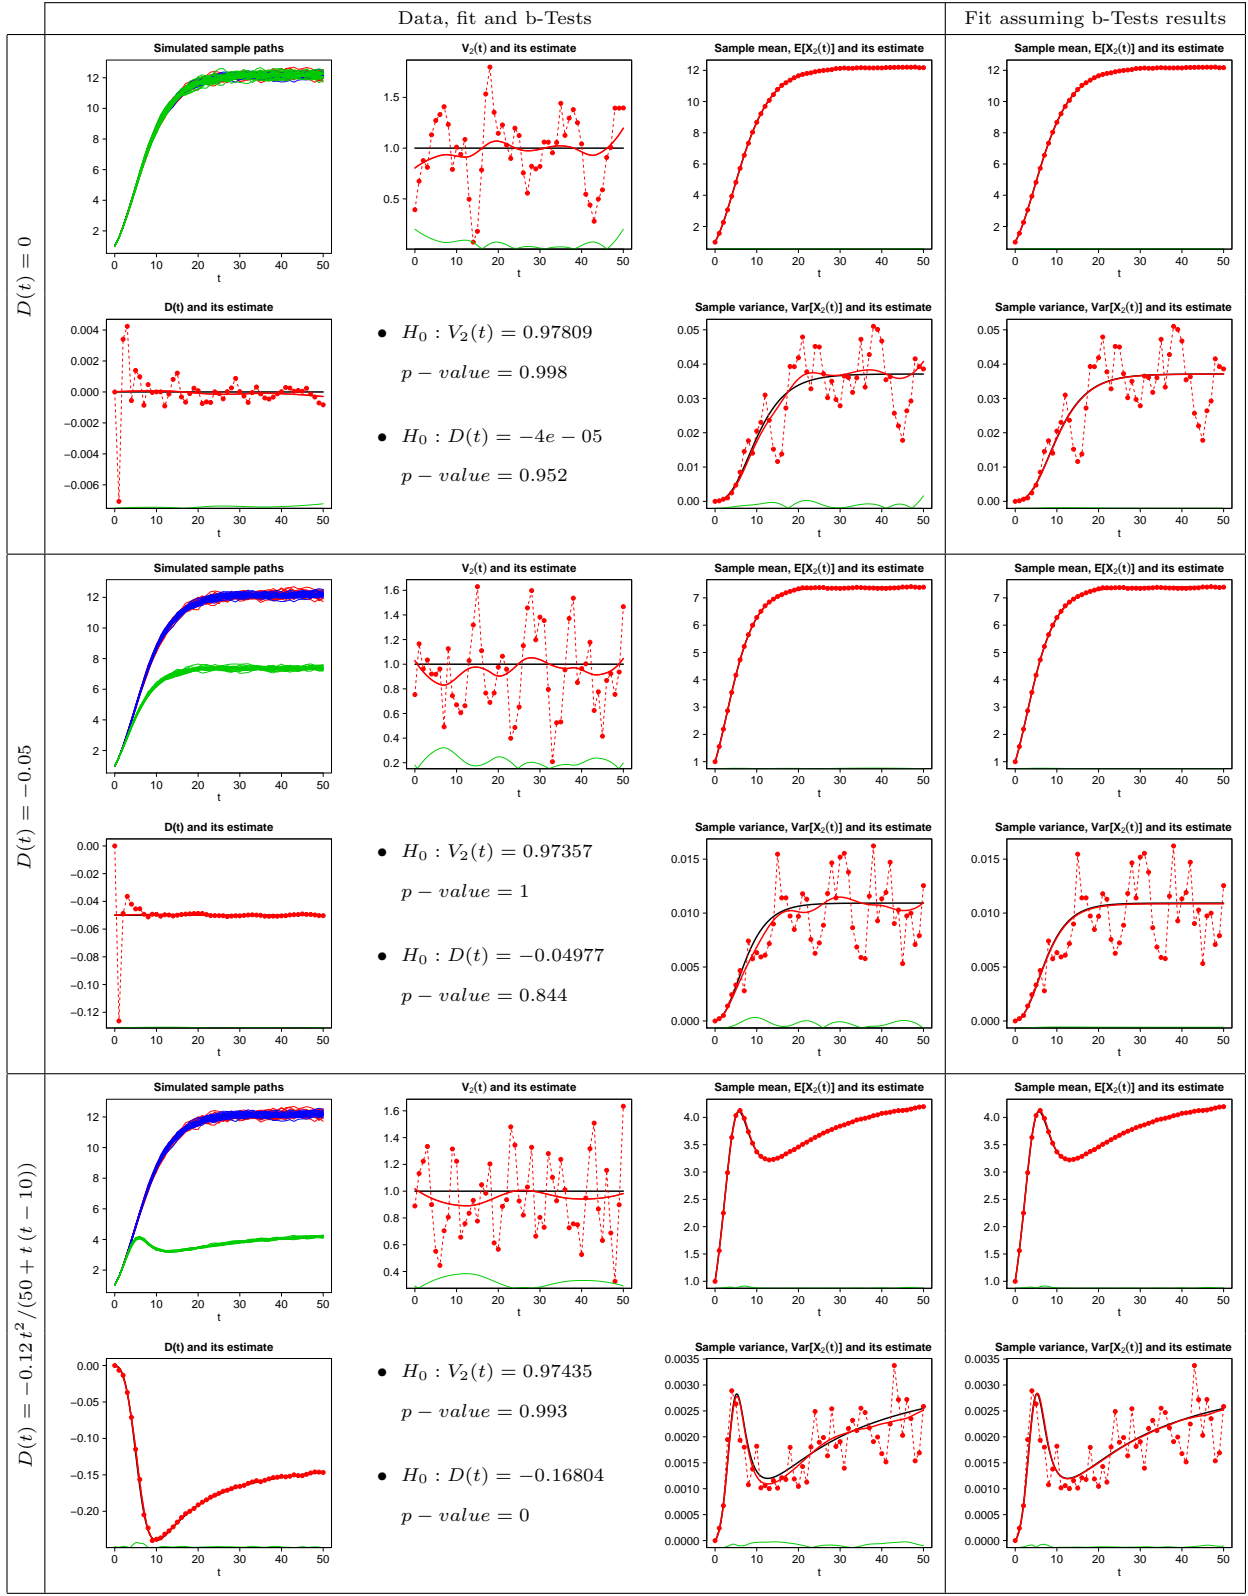

Table 16: Simulated data of the models (12), (13) and (15) (in red, blue and green, respectively) with  $\alpha = 0.5$ ,  $\beta = 0.2$ ,  $\sigma = 0.01$ ,  $V_1(t) = 0.49$ ,  $C(t) = 0$ ,  $V_2(t) = 1$  and different types of functions  $D(t)$ , estimates of  $D(t)$  and  $V_2(t)$  in model (15); concatenated bootstrap tests (b-Tests); and fit of simulated data of model (15).

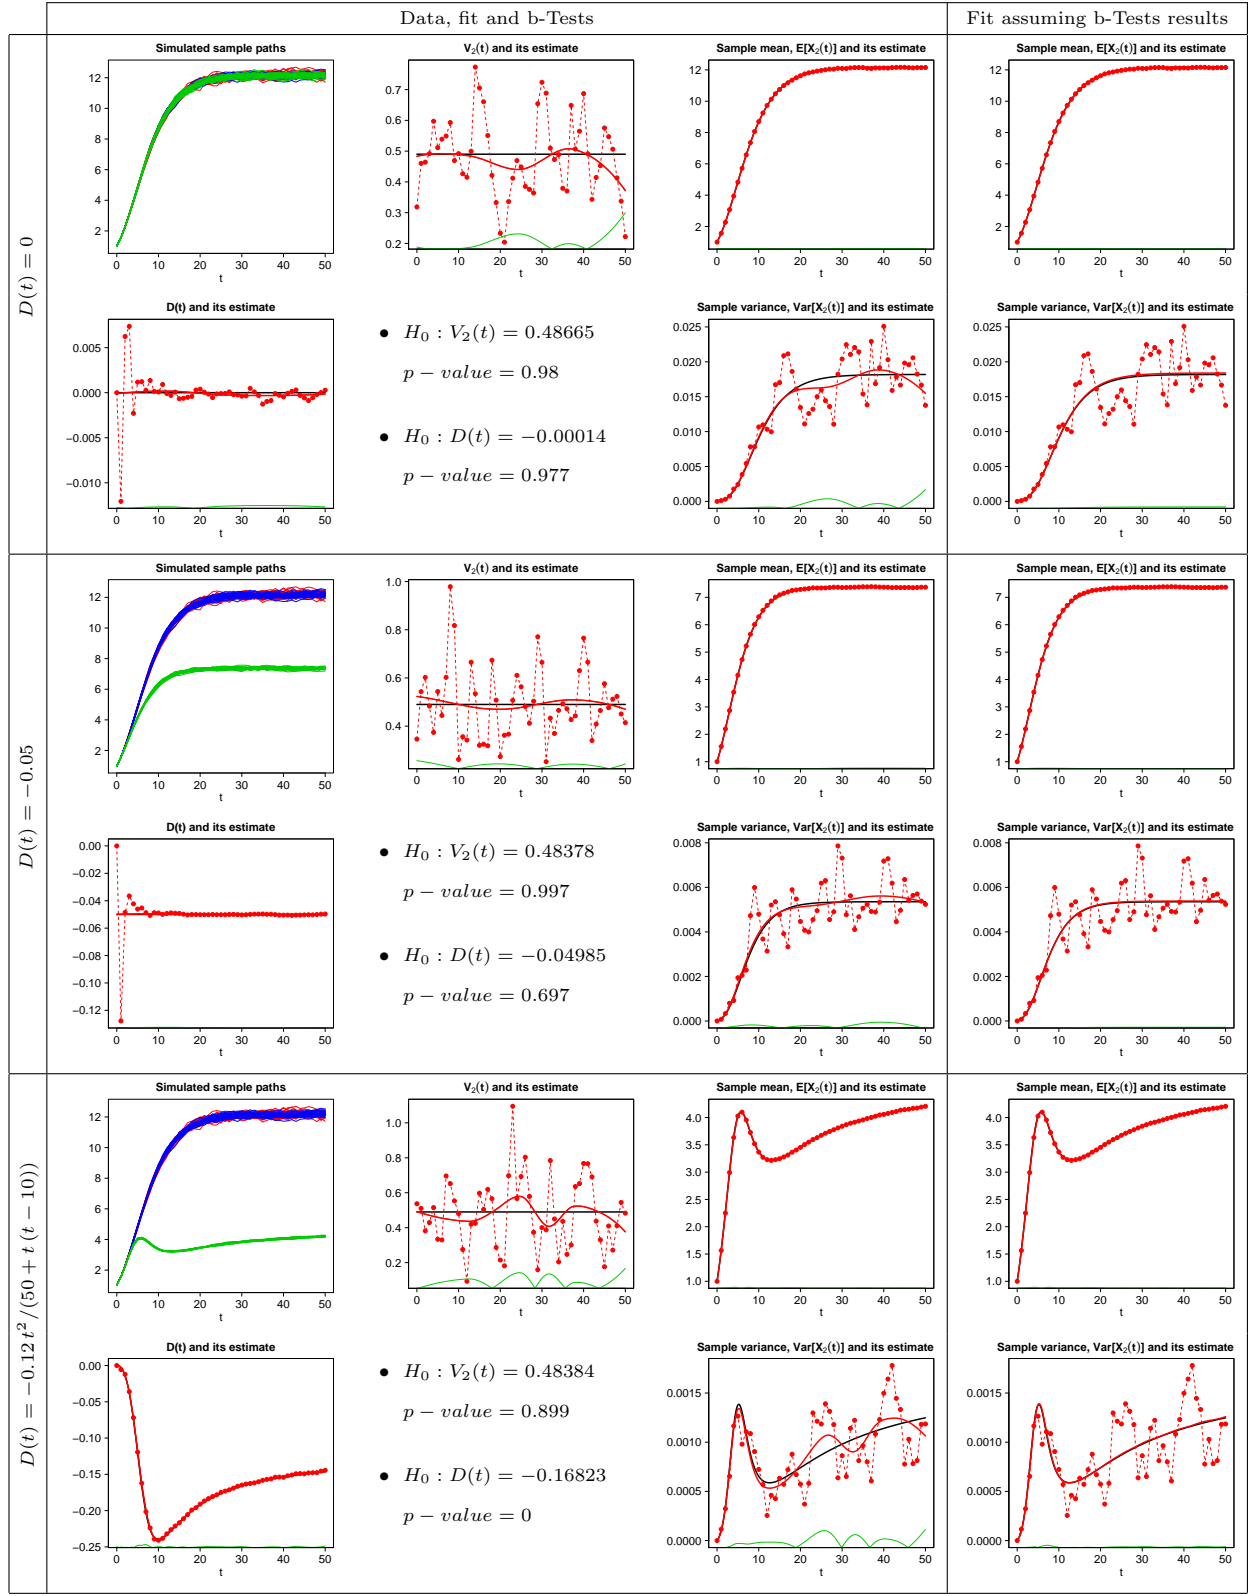

Table 17: Simulated data of the models (12), (13) and (15) (in red, blue and green, respectively) with  $\alpha = 0.5$ ,  $\beta = 0.2$ ,  $\sigma = 0.01$ ,  $V_1(t) = 0.49$ ,  $C(t) = 0$ ,  $V_2(t) = 0.49$  and different types of functions  $D(t)$ , estimates of  $D(t)$  and  $V_2(t)$  in model (15); concatenated bootstrap tests (b-Tests); and fit of simulated data of model (15).

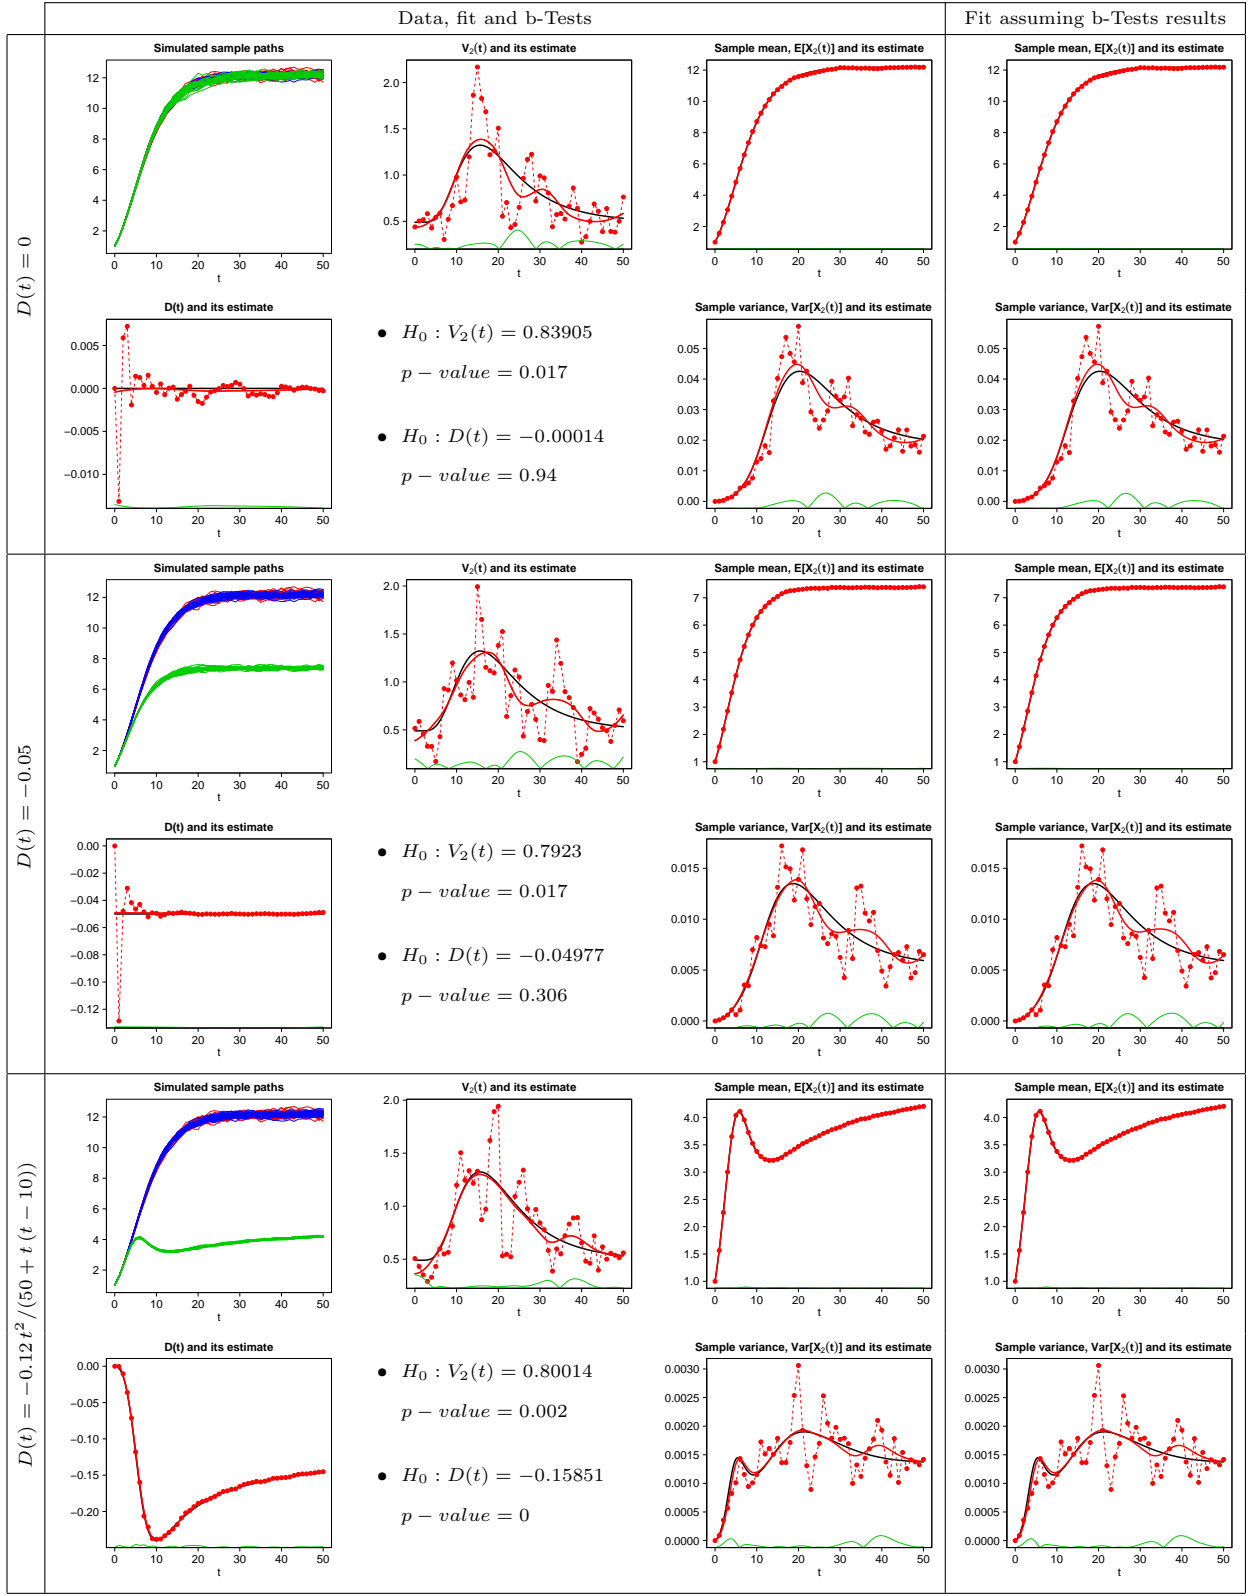

Table 18: Simulated data of the models (12), (13) and (15) (in red, blue and green, respectively) with  $\alpha = 0.5$ ,  $\beta = 0.2$ ,  $\sigma = 0.01$ ,  $V_1(t) = 0.49$ ,  $C(t) = 0$ ,  $V_2(t) = (0.7 + 10\Lambda(t, 3, 0.5))^2$  and different types of functions  $D(t)$ , estimates of  $D(t)$  and  $V_2(t)$  in model (15); concatenated bootstrap tests (b-Tests); and fit of simulated data of model (15).

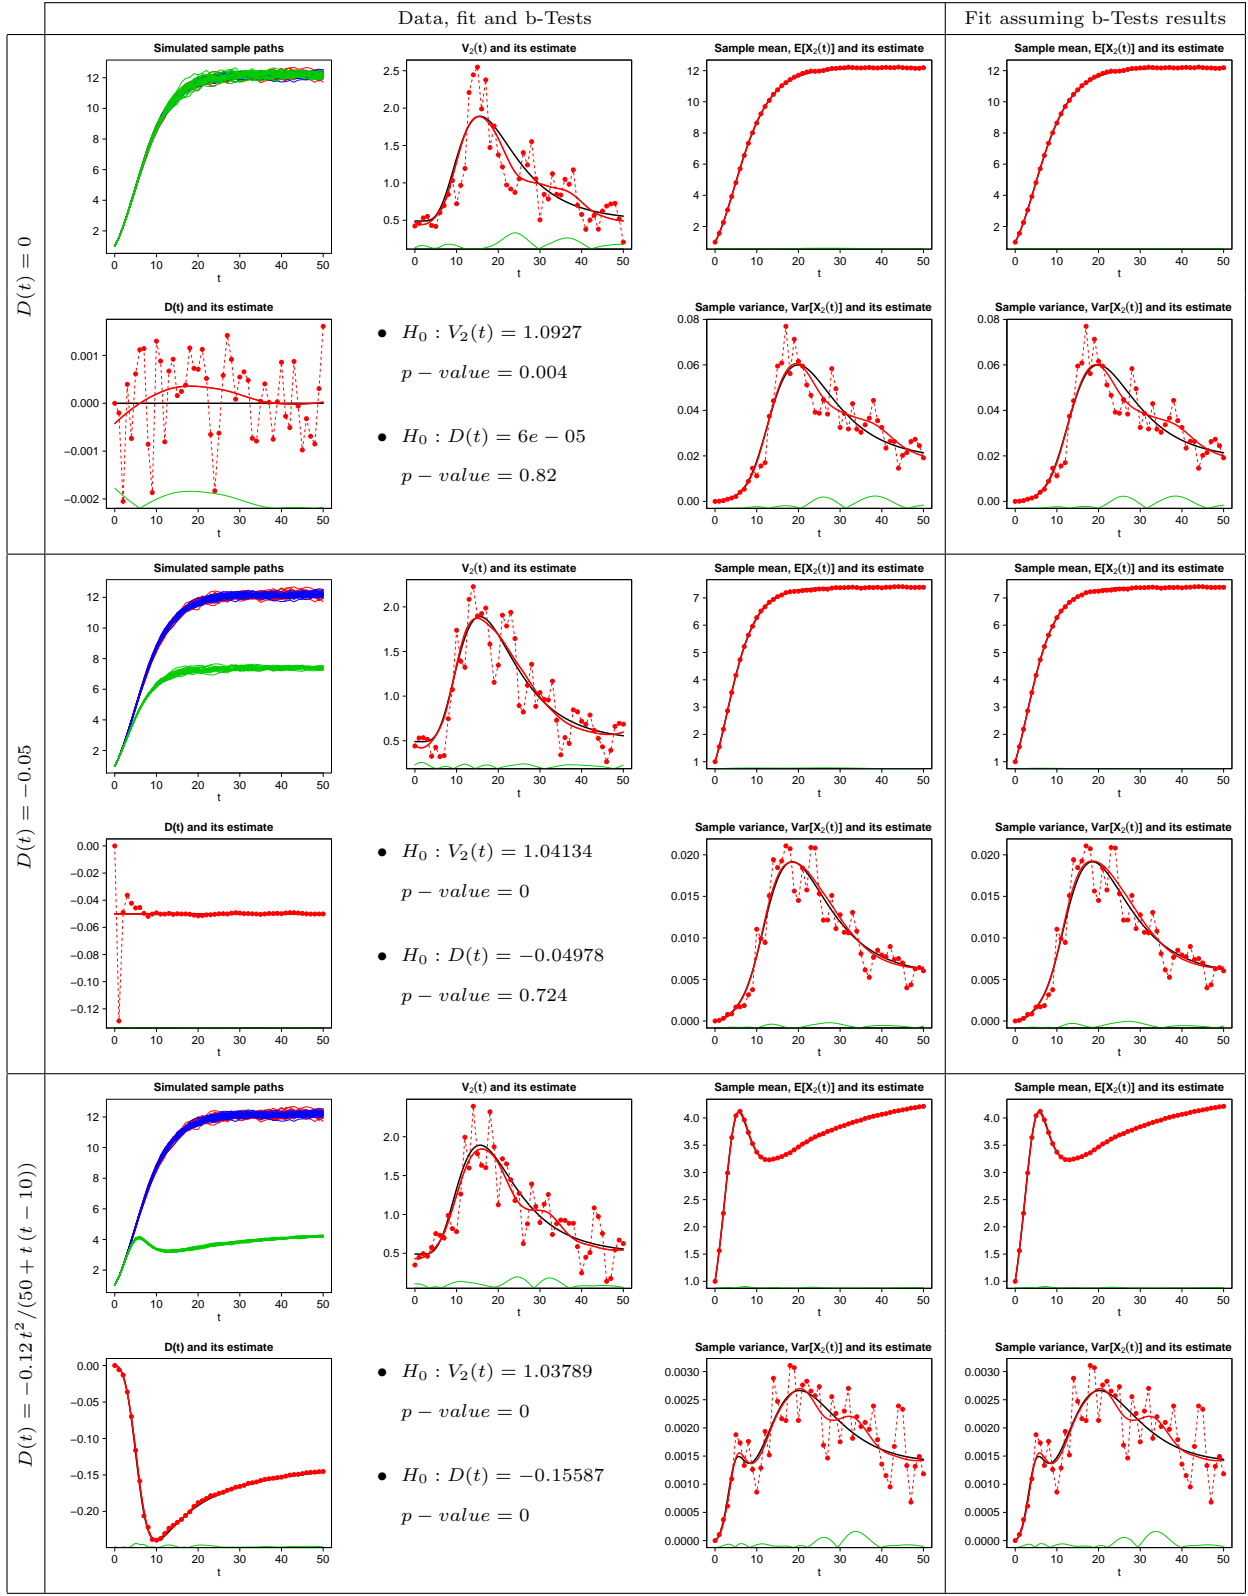

Table 19: Simulated data of the models (12), (13) and (15) (in red, blue and green, respectively) with  $\alpha = 0.5$ ,  $\beta = 0.2$ ,  $\sigma = 0.01$ ,  $V_1(t) = 0.49$ ,  $C(t) = 0$ ,  $V_2(t) = (0.7 + 15\Lambda(t, 3, 0.5))^2$  and different types of functions  $D(t)$ , estimates of  $D(t)$  and  $V_2(t)$  in model (15); concatenated bootstrap tests (b-Tests); and fit of simulated data of model (15).

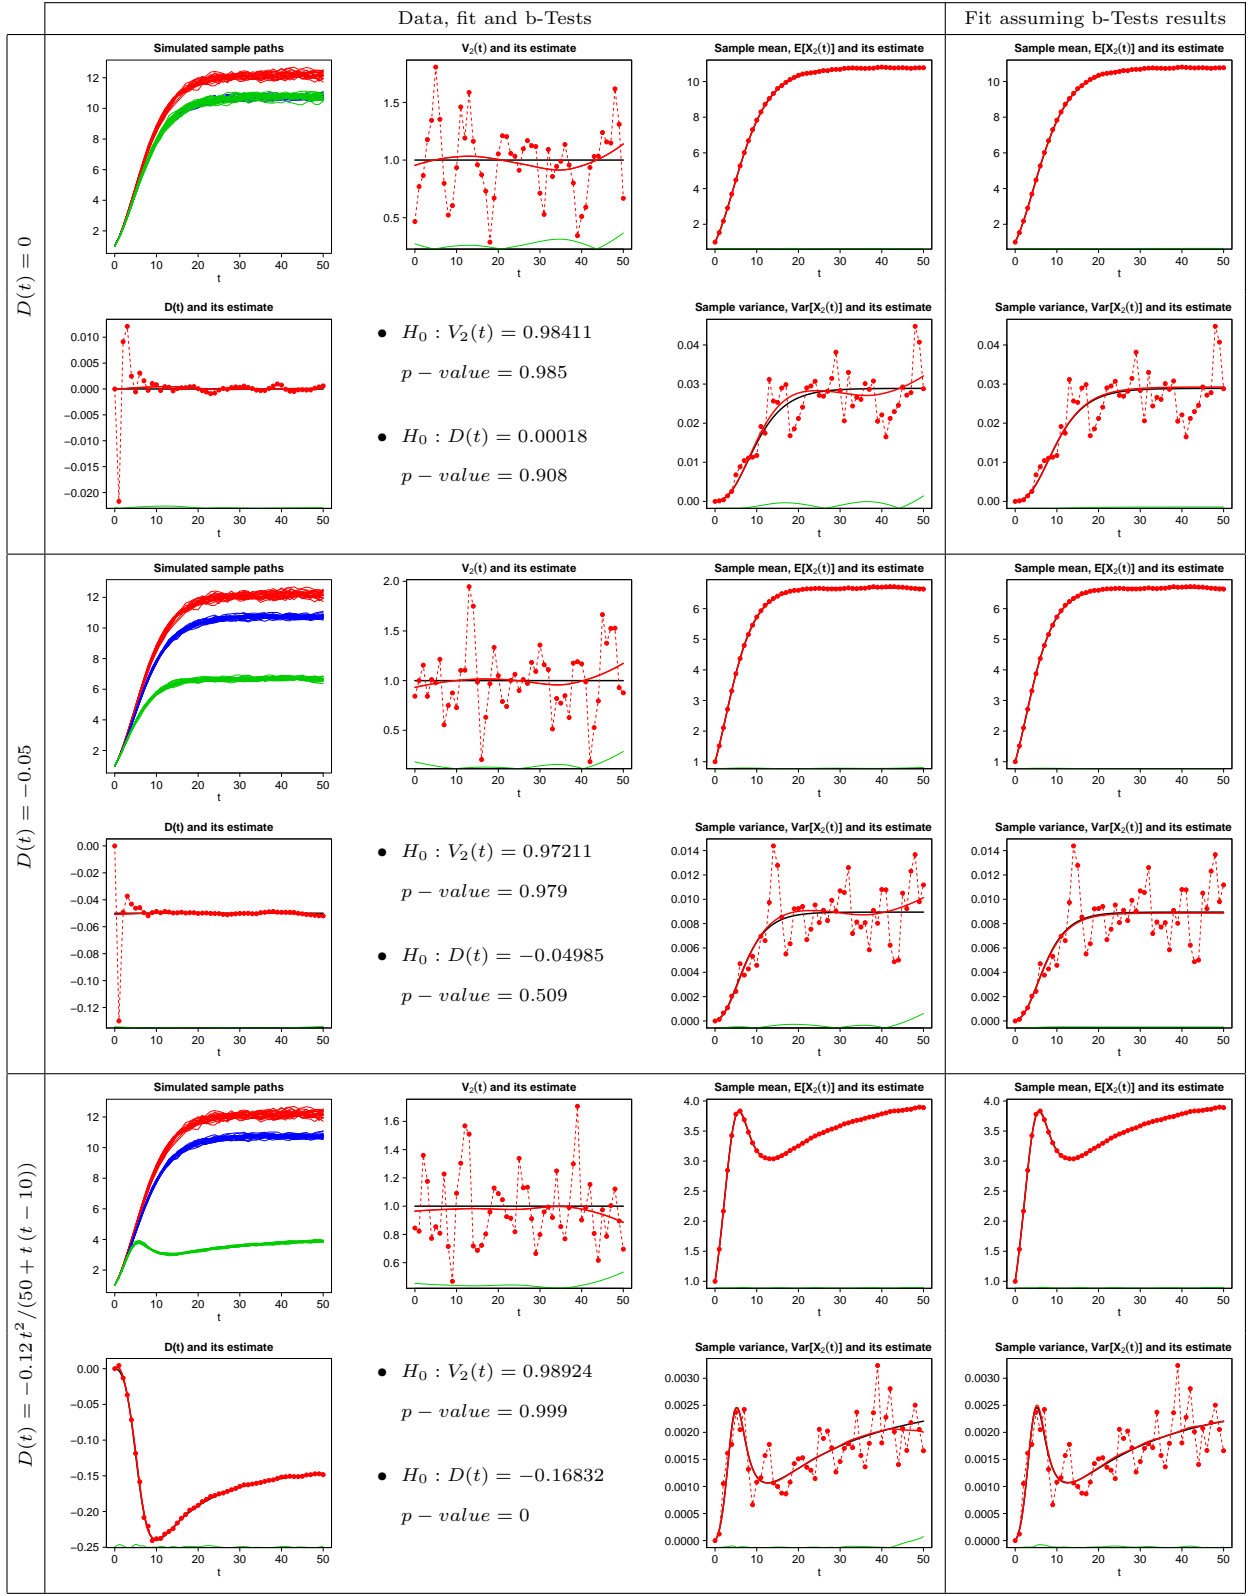

Table 20: Simulated data of the models (12), (13) and (15) (in red, blue and green, respectively) with  $\alpha = 0.5$ ,  $\beta = 0.2$ ,  $\sigma = 0.01$ ,  $V_1(t) = 0.49$ ,  $C(t) = 0.025$ ,  $V_2(t) = 1$  and different types of functions  $D(t)$ , estimates of  $D(t)$  and  $V_2(t)$  in model (15); concatenated bootstrap tests (b-Tests); and fit of simulated data of model (15).

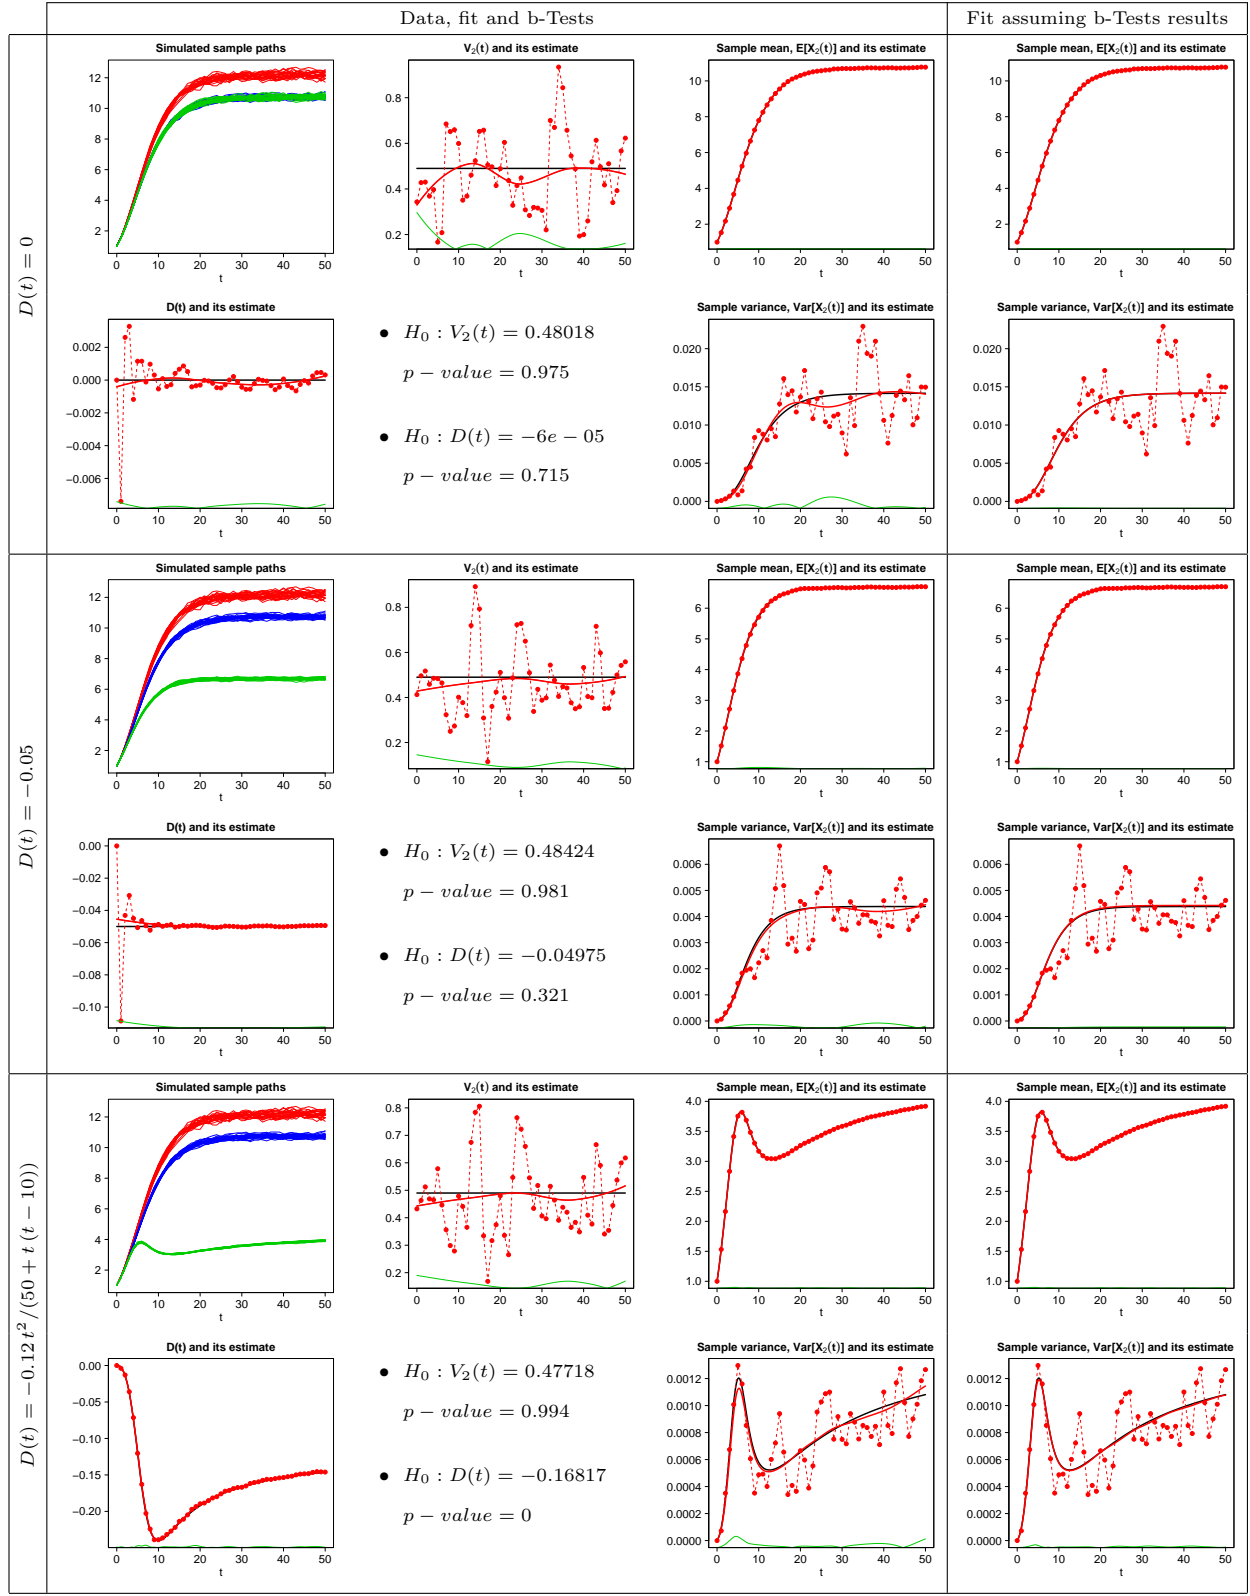

Table 21: Simulated data of the models (12), (13) and (15) (in red, blue and green, respectively) with  $\alpha = 0.5$ ,  $\beta = 0.2$ ,  $\sigma = 0.01$ ,  $V_1(t) = 0.49$ ,  $C(t) = 0.025$ ,  $V_2(t) = 0.49$  and different types of functions  $D(t)$ , estimates of  $D(t)$  and  $V_2(t)$  in model (15); concatenated bootstrap tests (b-Tests); and fit of simulated data of model (15).

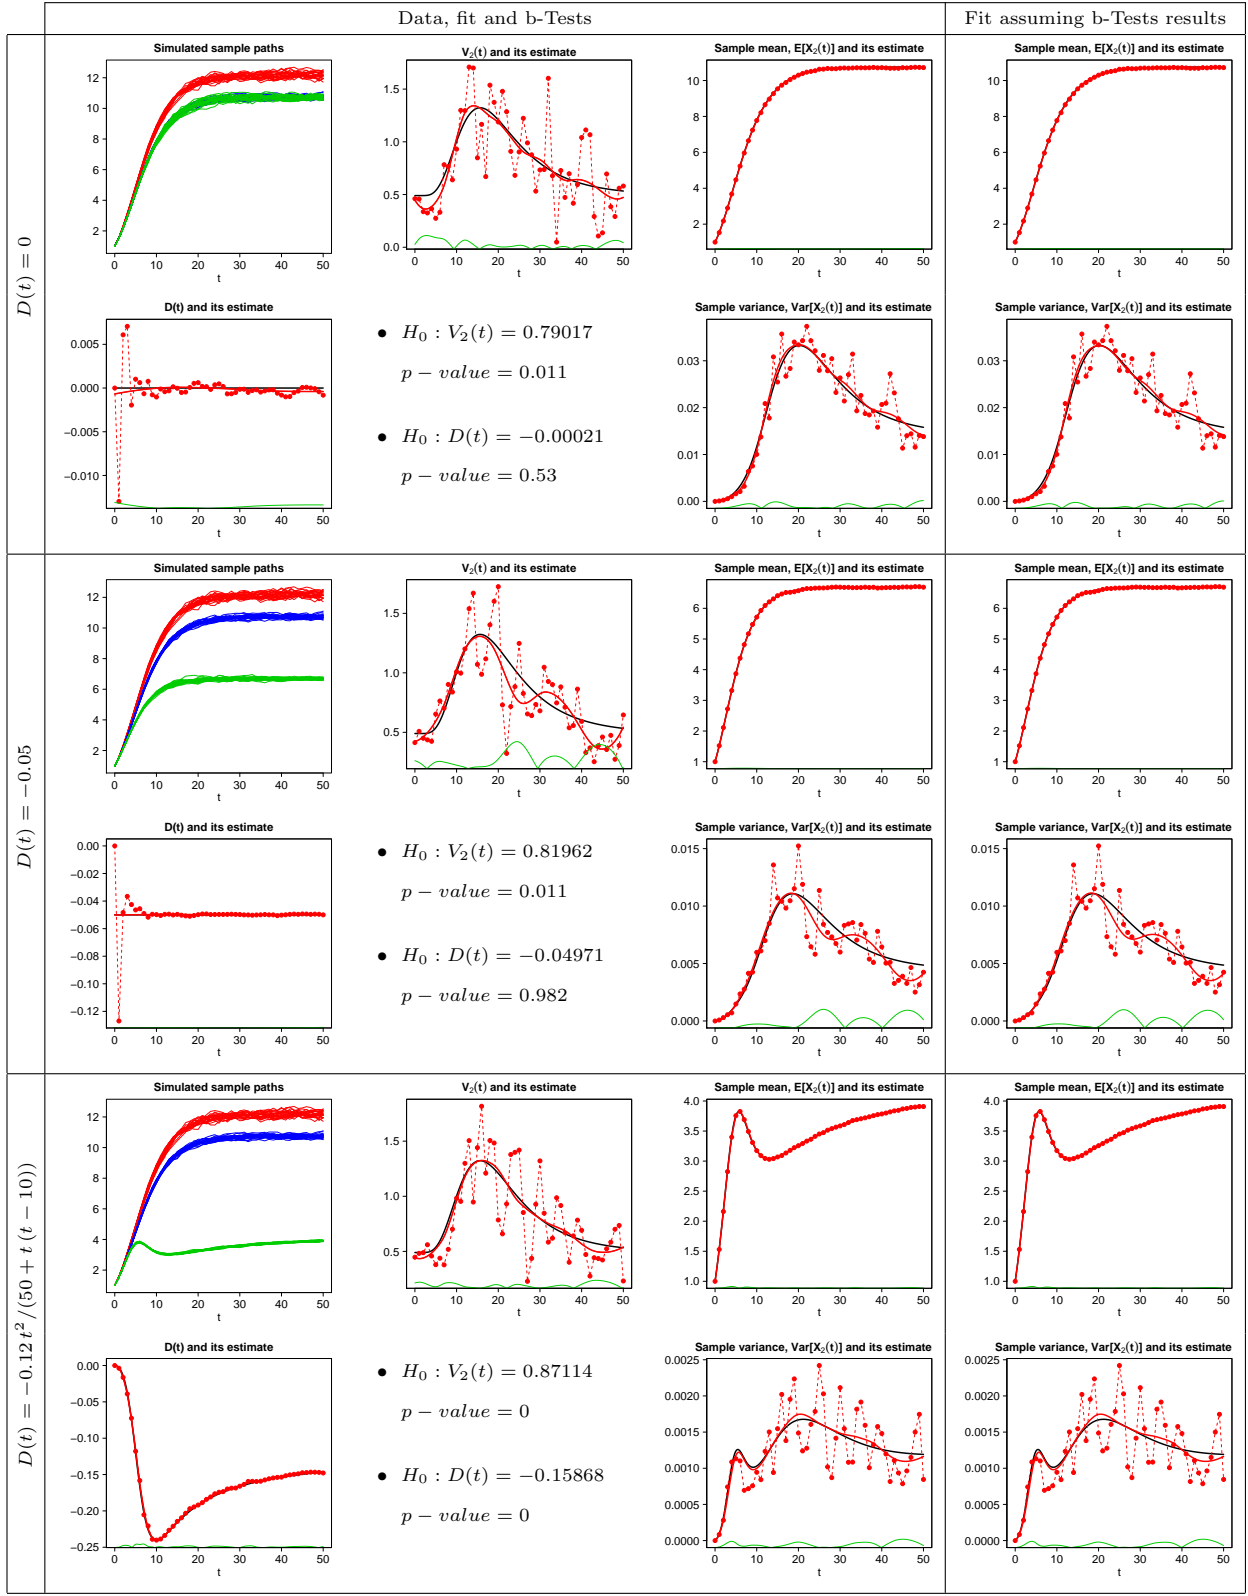

Table 22: Simulated data of the models (12), (13) and (15) (in red, blue and green, respectively) with  $\alpha = 0.5$ ,  $\beta = 0.2$ ,  $\sigma = 0.01$ ,  $V_1(t) = 0.49$ ,  $C(t) = 0.025$ ,  $V_2(t) = (0.7+10\Lambda(t, 3, 0.5))^2$  and different types of functions  $D(t)$ , estimates of  $D(t)$  and  $V_2(t)$  in model (15); concatenated bootstrap tests (b-Tests); and fit of simulated data of model (15).

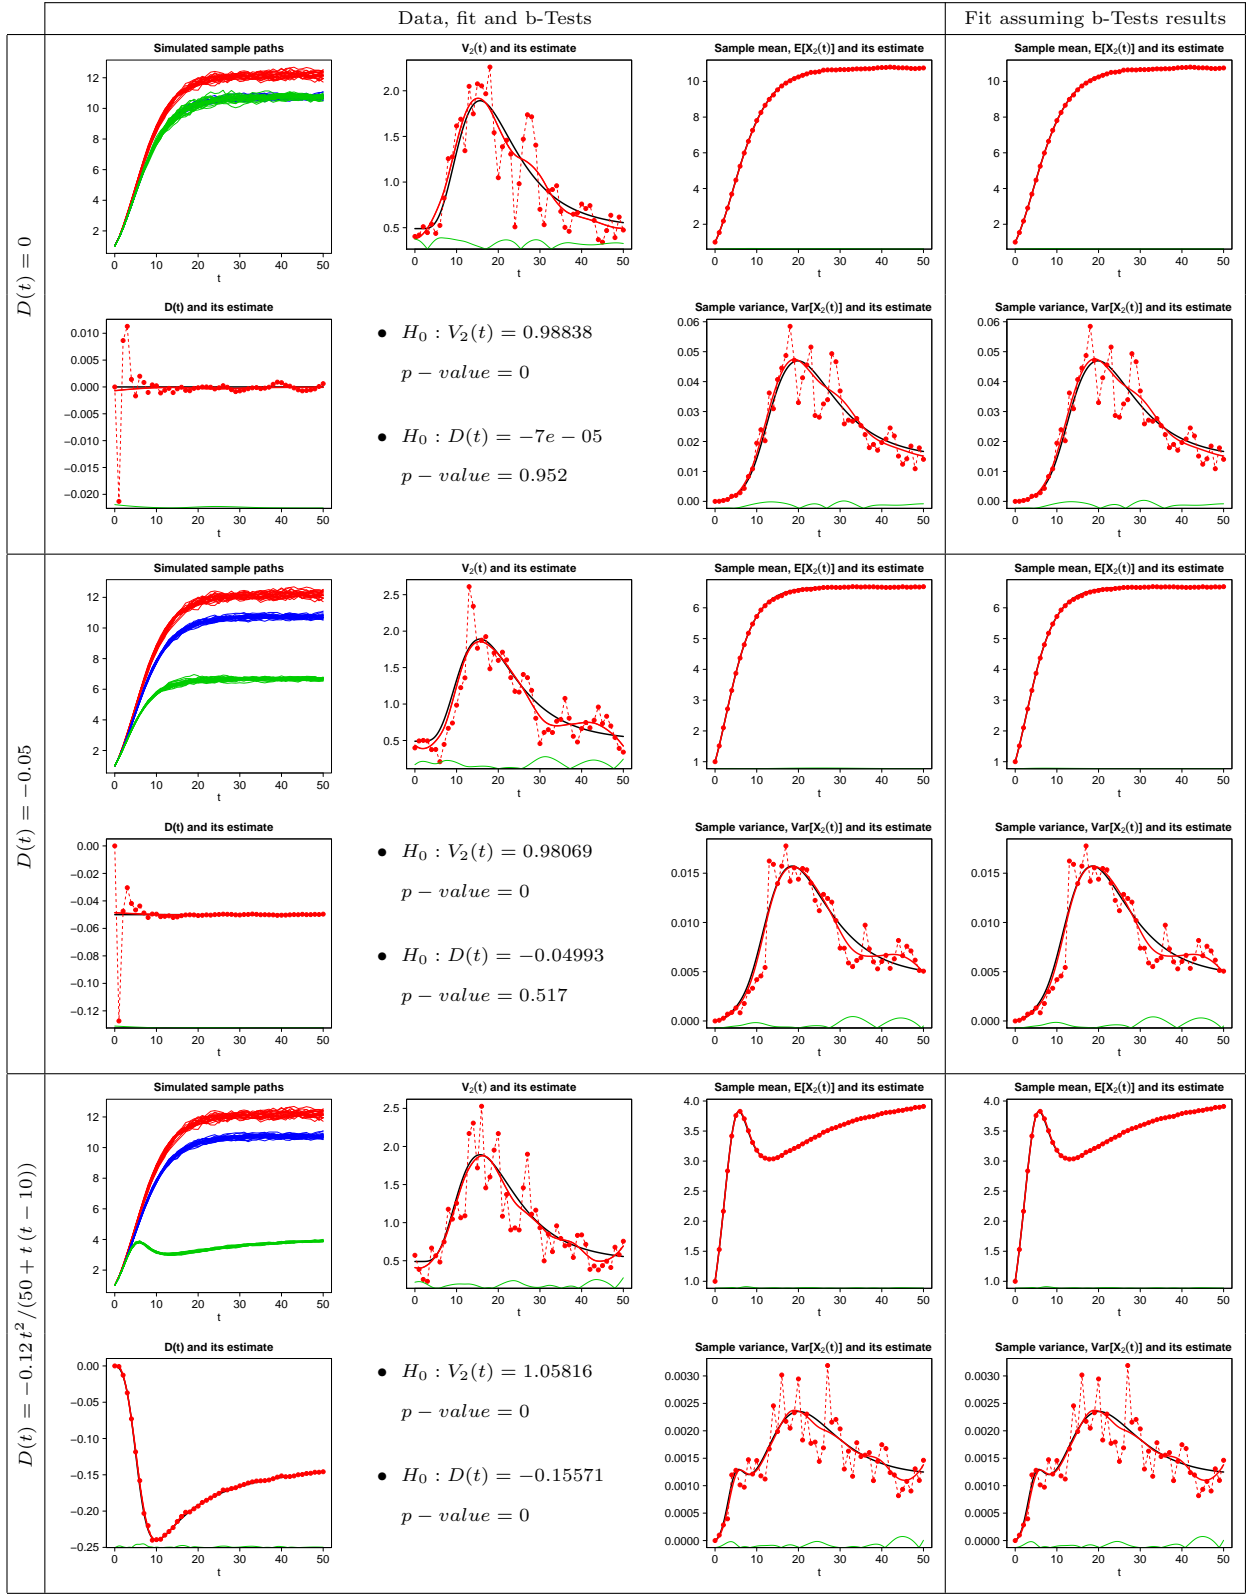

Table 23: Simulated data of the models (12), (13) and (15) (in red, blue and green, respectively) with  $\alpha = 0.5$ ,  $\beta = 0.2$ ,  $\sigma = 0.01$ ,  $V_1(t) = 0.49$ ,  $C(t) = 0.025$ ,  $V_2(t) = (0.7 + 15 \Lambda(t, 3, 0.5))^2$  and different types of functions  $D(t)$ , estimates of  $D(t)$  and  $V_2(t)$  in model (15); concatenated bootstrap tests (b-Tests); and fit of simulated data of model (15).

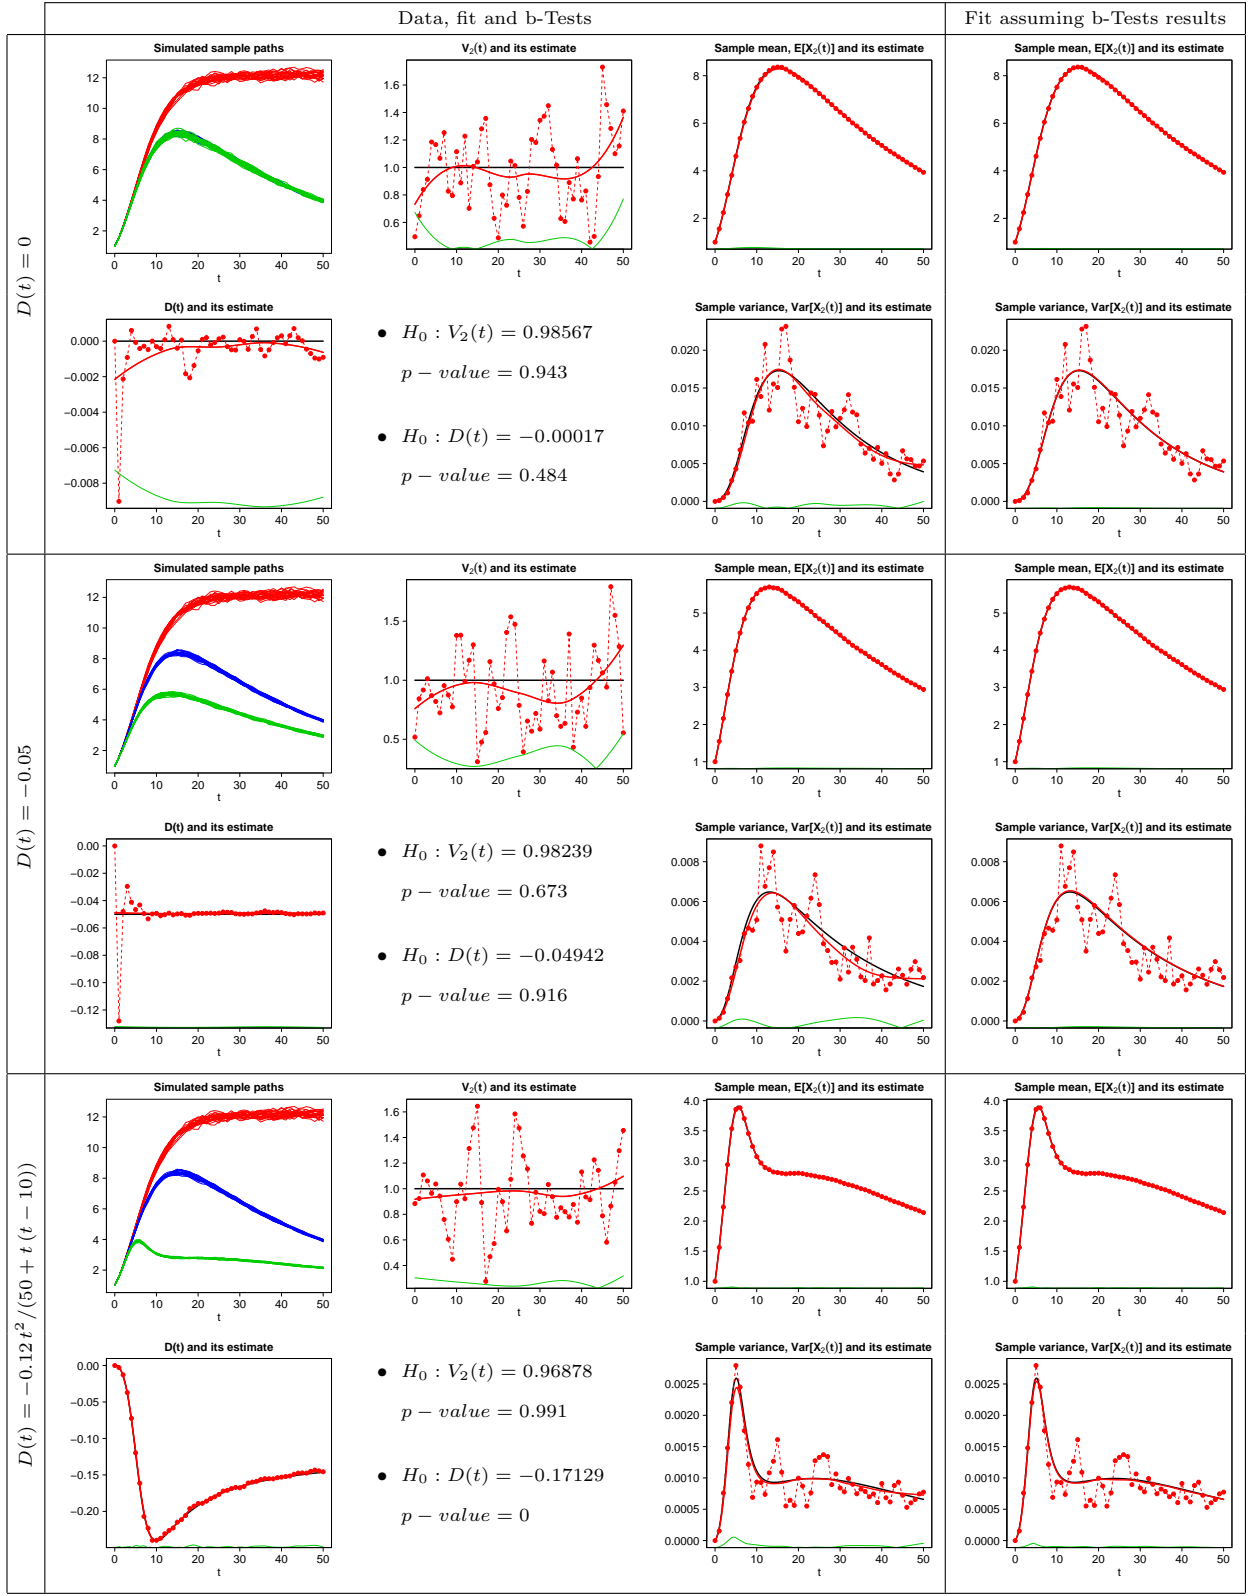

Table 24: Simulated data of the models (12), (13) and (15) (in red, blue and green, respectively) with  $\alpha = 0.5$ ,  $\beta = 0.2$ ,  $\sigma = 0.01$ ,  $V_1(t) = 0.49$ ,  $C(t) = 0.005t$ ,  $V_2(t) = 1$  and different types of functions  $D(t)$ , estimates of  $D(t)$  and  $V_2(t)$  in model (15); concatenated bootstrap tests (b-Tests); and fit of simulated data of model (15).

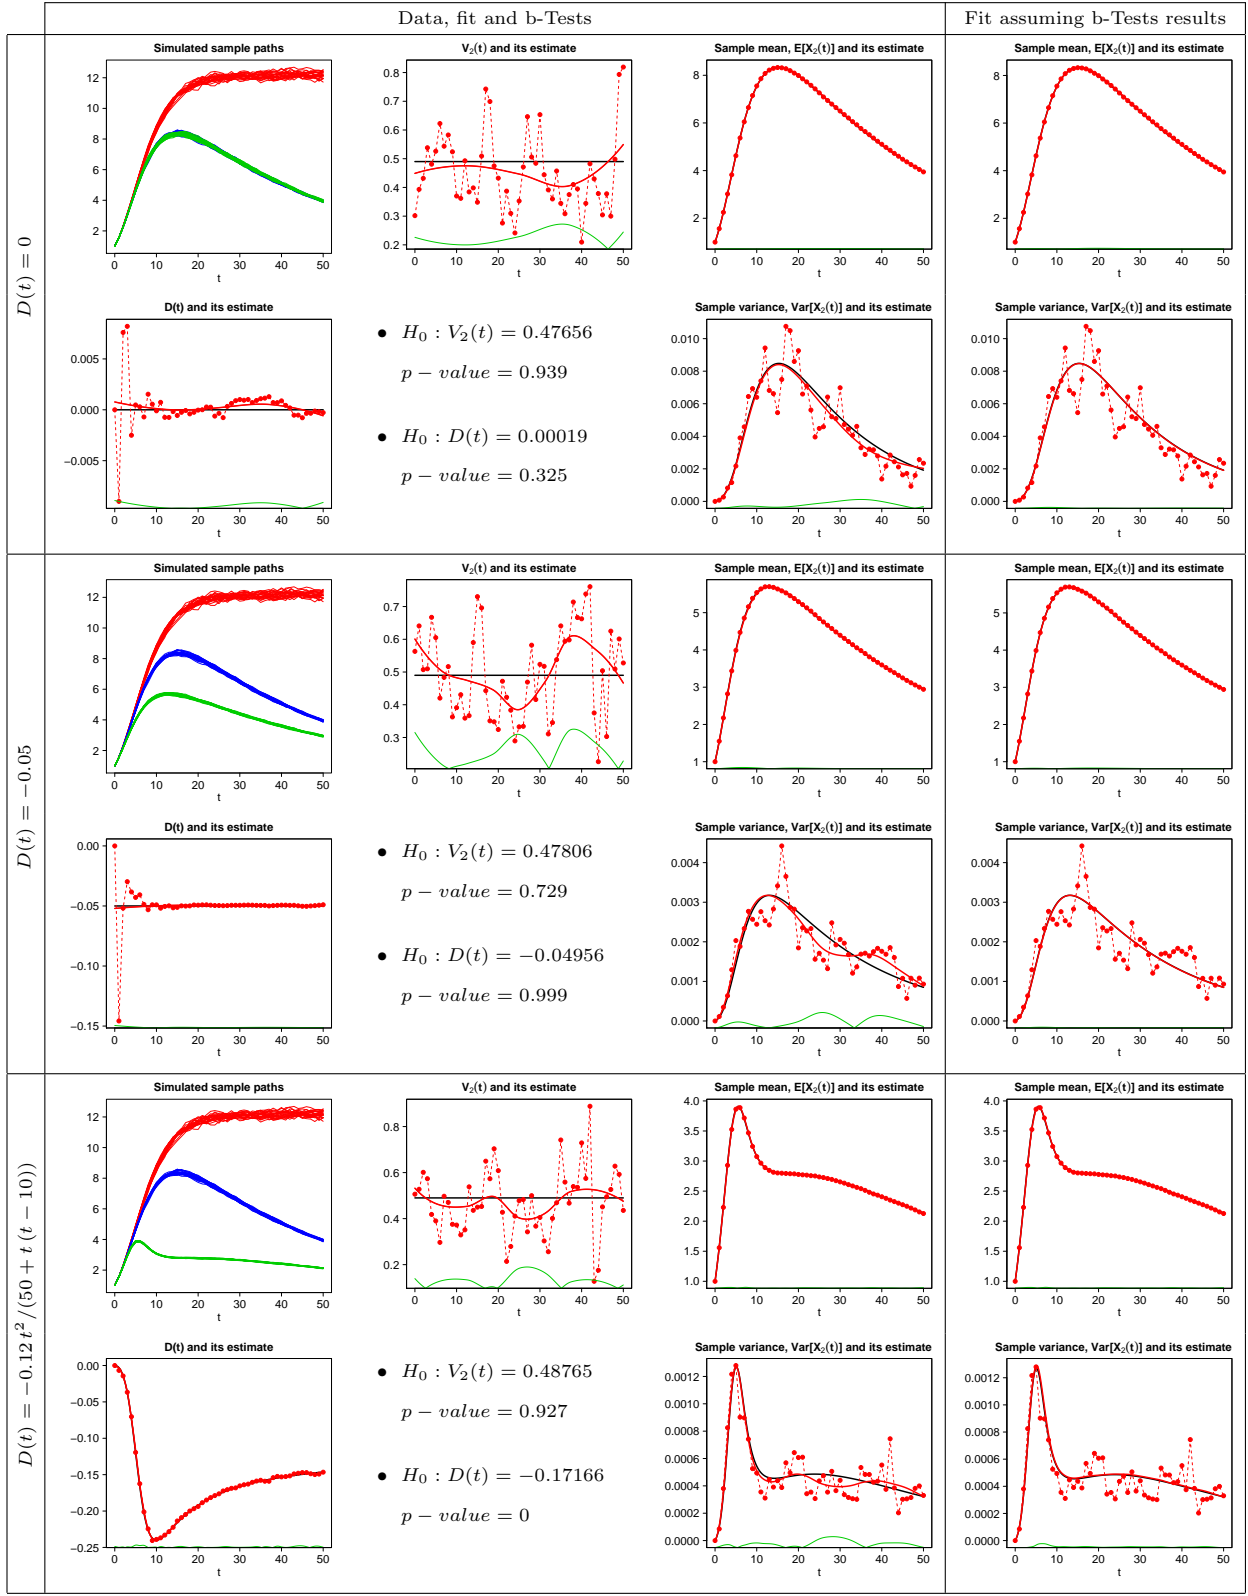

Table 25: Simulated data of the models (12), (13) and (15) (in red, blue and green, respectively) with  $\alpha = 0.5$ ,  $\beta = 0.2$ ,  $\sigma = 0.01$ ,  $V_1(t) = 0.49$ ,  $C(t) = 0.005t$ ,  $V_2(t) = 0.49$  and different types of functions  $D(t)$ , estimates of  $D(t)$  and  $V_2(t)$  in model (15); concatenated bootstrap tests (b-Tests); and fit of simulated data of model (15).

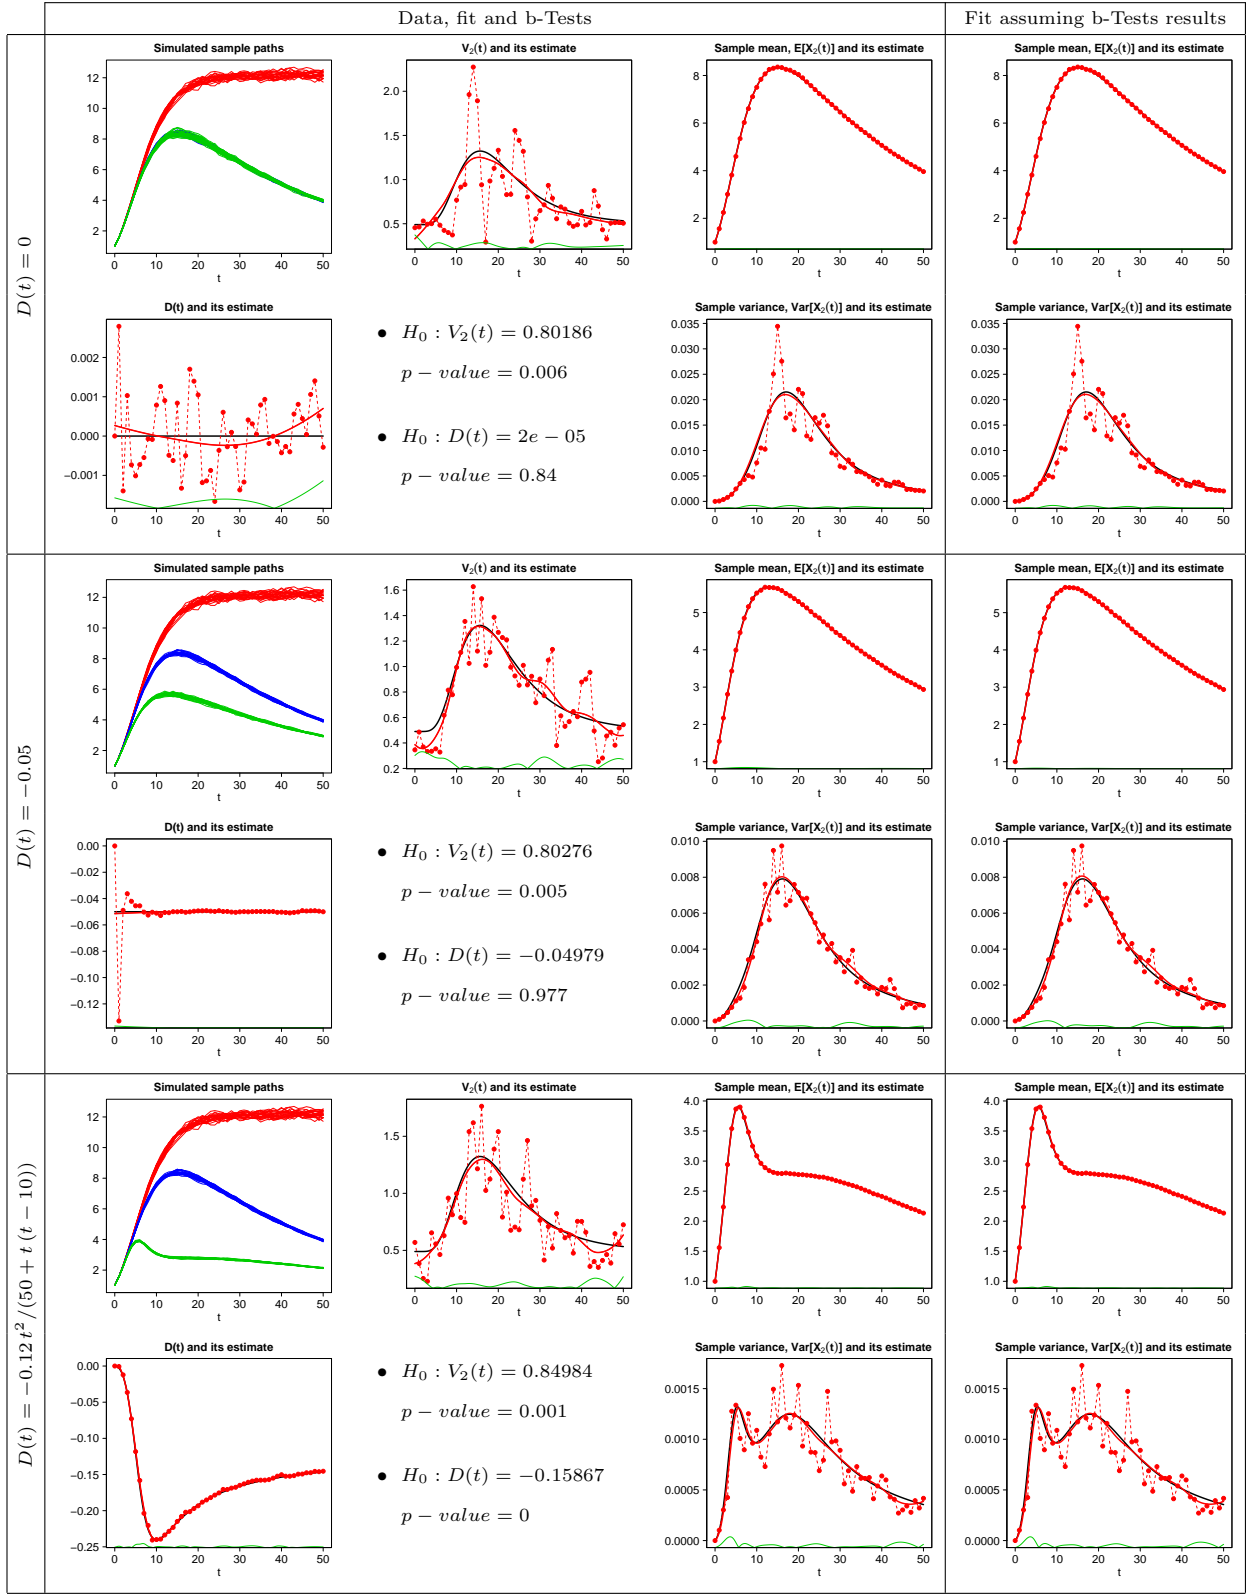

Table 26: Simulated data of the models (12), (13) and (15) (in red, blue and green, respectively) with  $\alpha = 0.5$ ,  $\beta = 0.2$ ,  $\sigma = 0.01$ ,  $V_1(t) = 0.49$ ,  $C(t) = 0.005t$ ,  $V_2(t) = (0.7 + 10\Lambda(t, 3, 0.5))^2$  and different types of functions  $D(t)$ , estimates of  $D(t)$  and  $V_2(t)$  in model (15); concatenated bootstrap tests (b-Tests); and fit of simulated data of model (15).

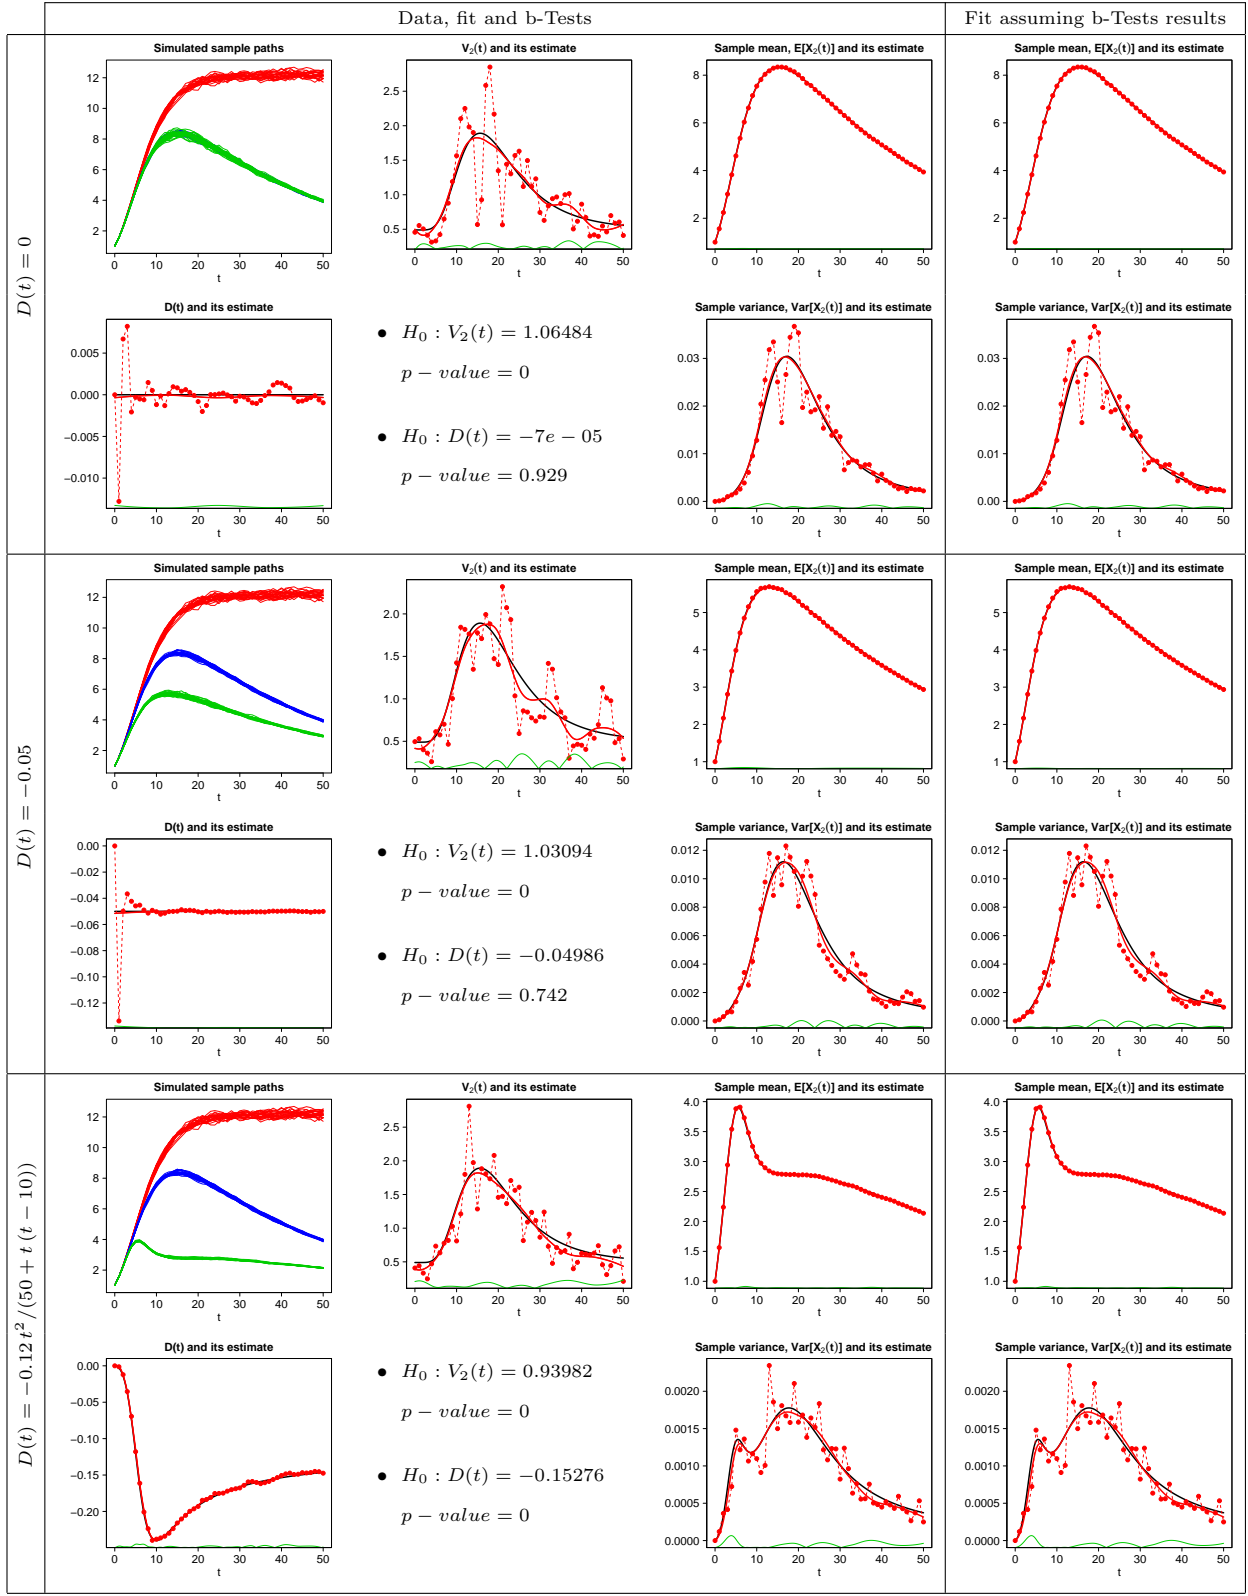

Table 27: Simulated data of the models (12), (13) and (15) (in red, blue and green, respectively) with  $\alpha = 0.5$ ,  $\beta = 0.2$ ,  $\sigma = 0.01$ ,  $V_1(t) = 0.49$ ,  $C(t) = 0.005t$ ,  $V_2(t) = (0.7 + 15\Lambda(t, 3, 0.5))^2$  and different types of functions  $D(t)$ , estimates of  $D(t)$  and  $V_2(t)$  in model (15); concatenated bootstrap tests (b-Tests); and fit of simulated data of model (15).

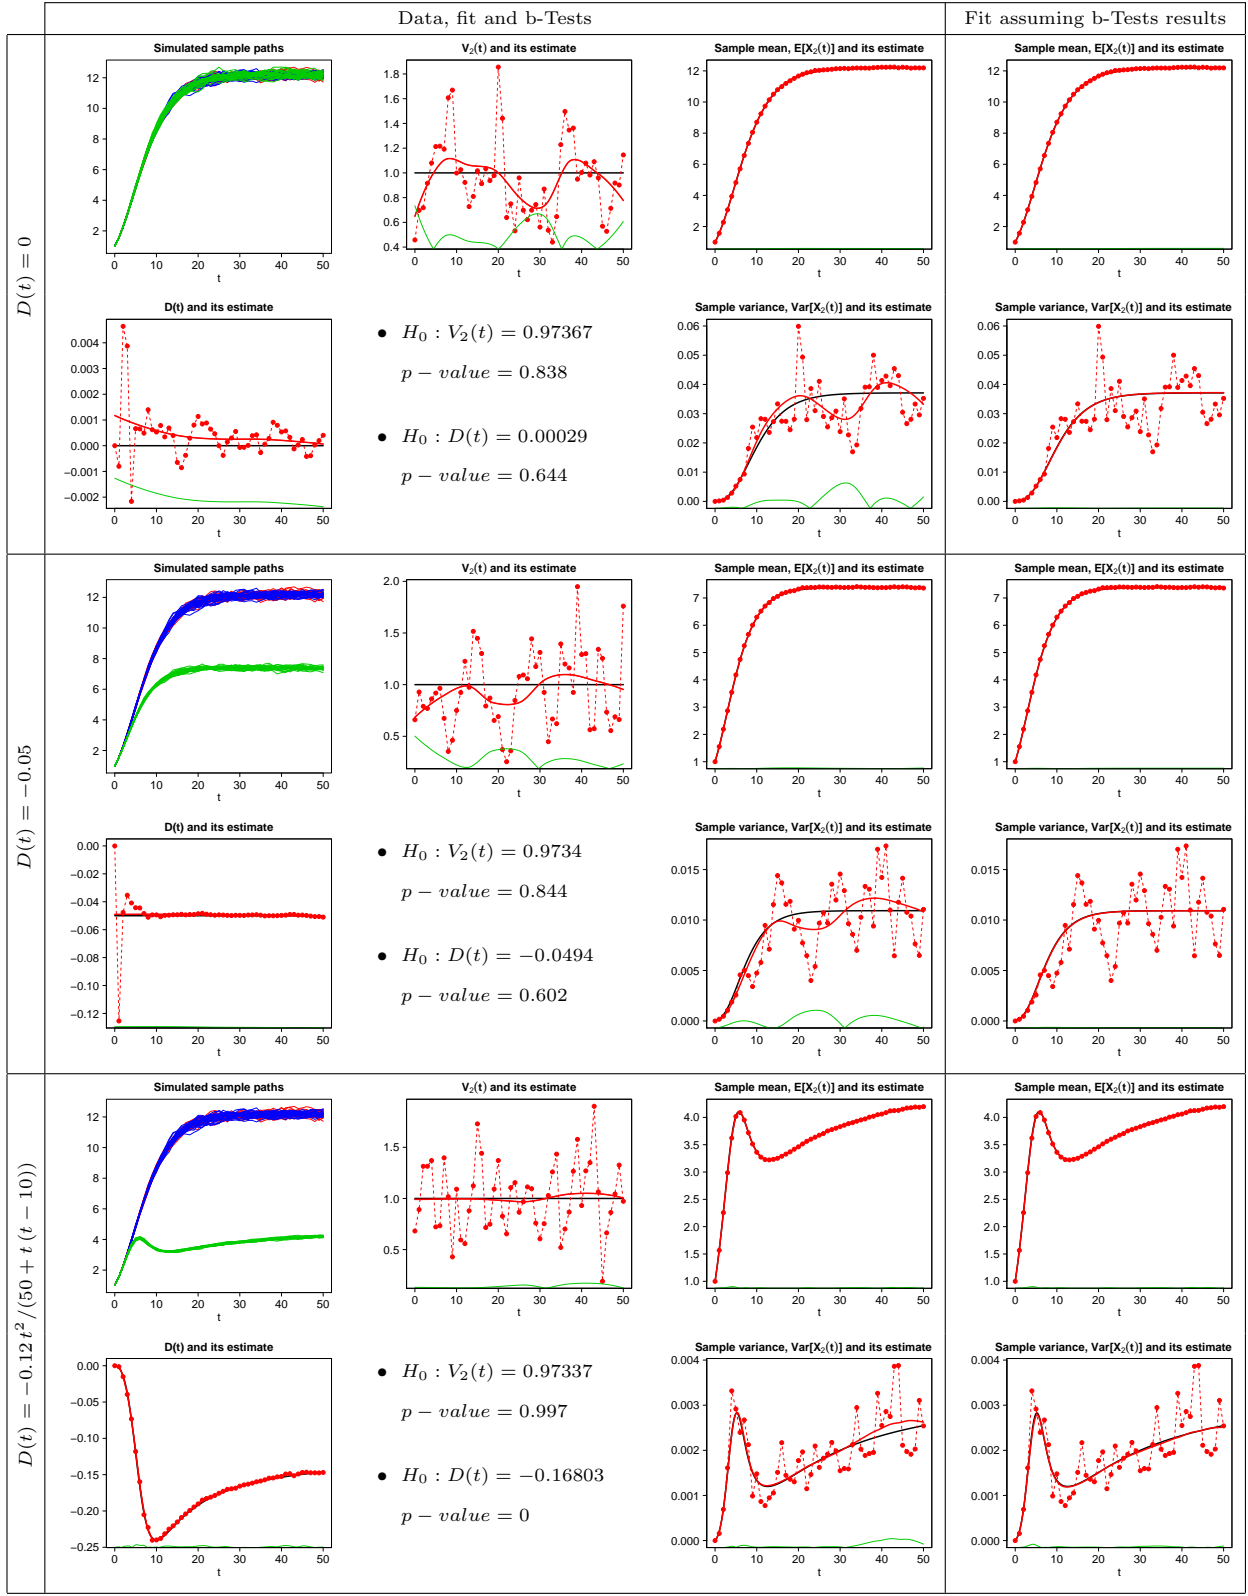

Table 28: Simulated data of the models (12), (13) and (15) (in red, blue and green, respectively) with  $\alpha = 0.5$ ,  $\beta = 0.2$ ,  $\sigma = 0.01$ ,  $V_1(t) = (0.7 + 10\Lambda(t, 3, 0.5))^2$ ,  $C(t) = 0$ ,  $V_2(t) = 1$  and different types of functions  $D(t)$ , estimates of  $D(t)$  and  $V_2(t)$  in model (15); concatenated bootstrap tests (b-Tests); and fit of simulated data of model (15).

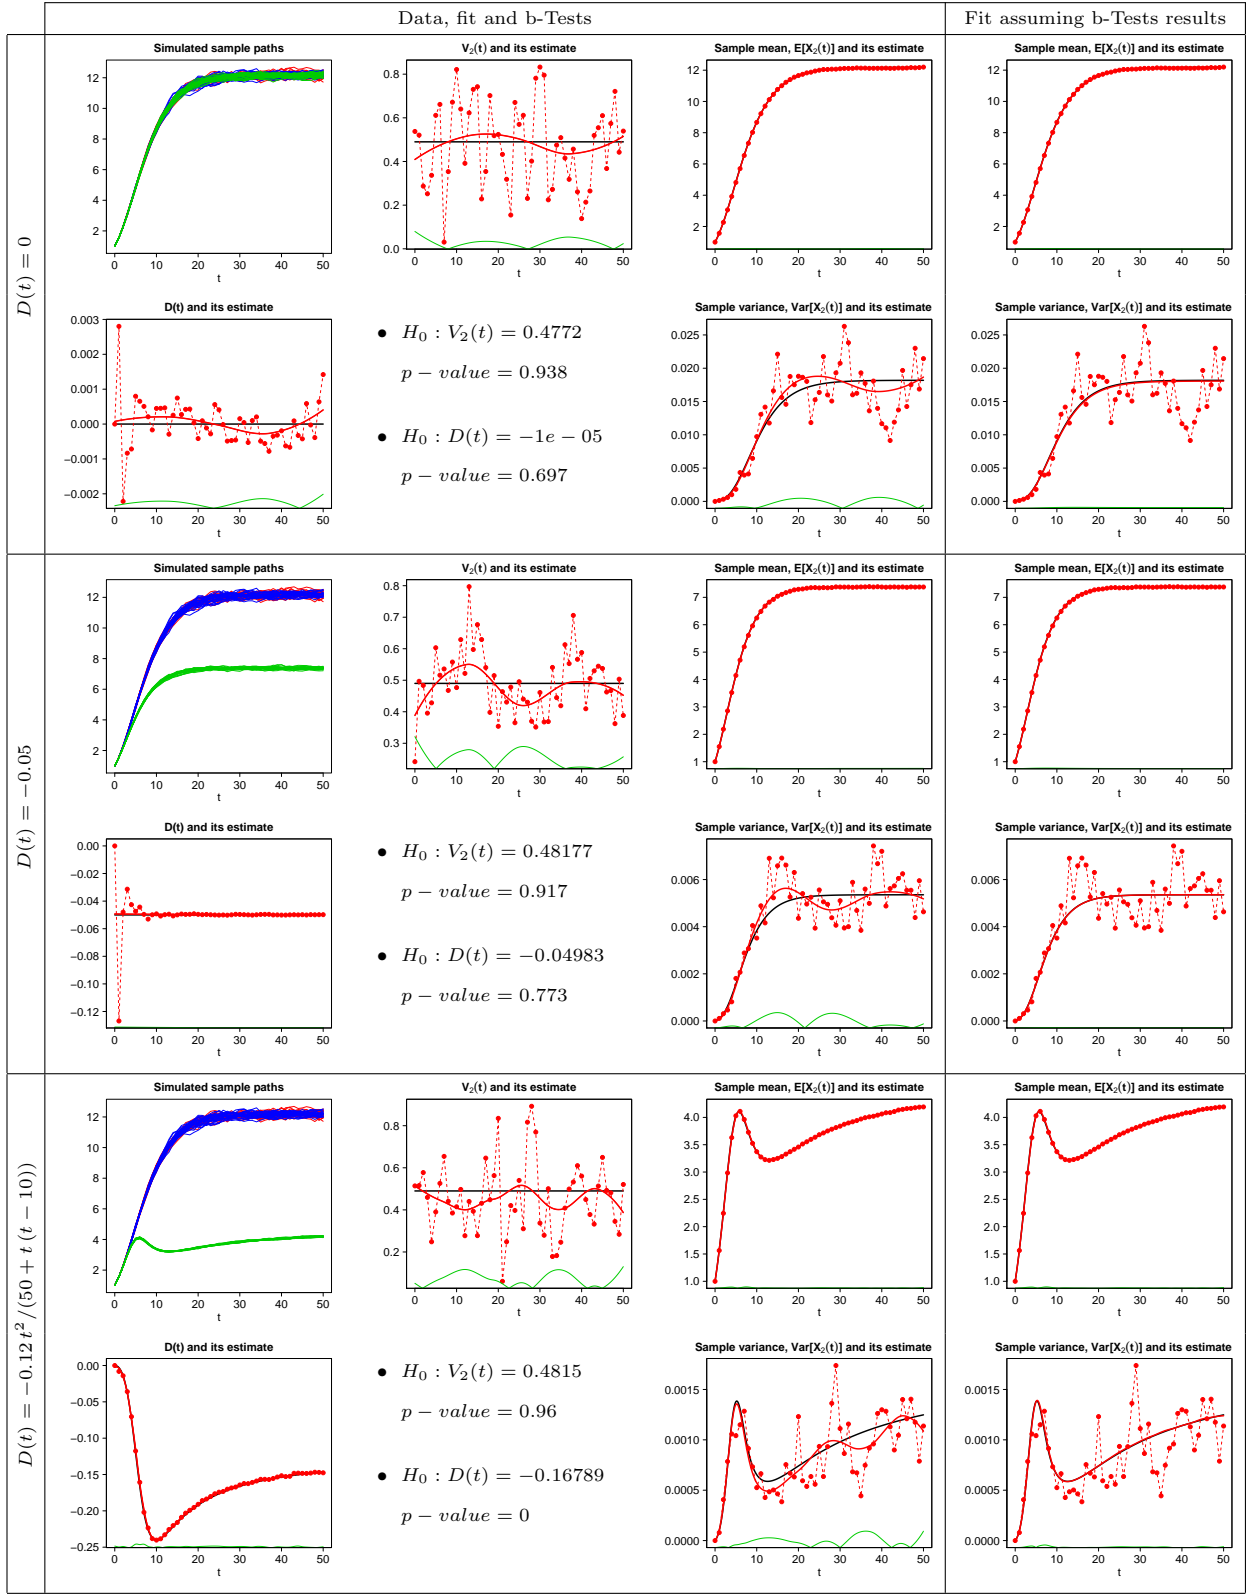

Table 29: Simulated data of the models (12), (13) and (15) (in red, blue and green, respectively) with  $\alpha = 0.5$ ,  $\beta = 0.2$ ,  $\sigma = 0.01$ ,  $V_1(t) = (0.7 + 10\Lambda(t, 3, 0.5))^2$ ,  $C(t) = 0$ ,  $V_2(t) = 0.49$  and different types of functions  $D(t)$ , estimates of  $D(t)$  and  $V_2(t)$  in model (15); concatenated bootstrap tests (b-Tests); and fit of simulated data of model (15).

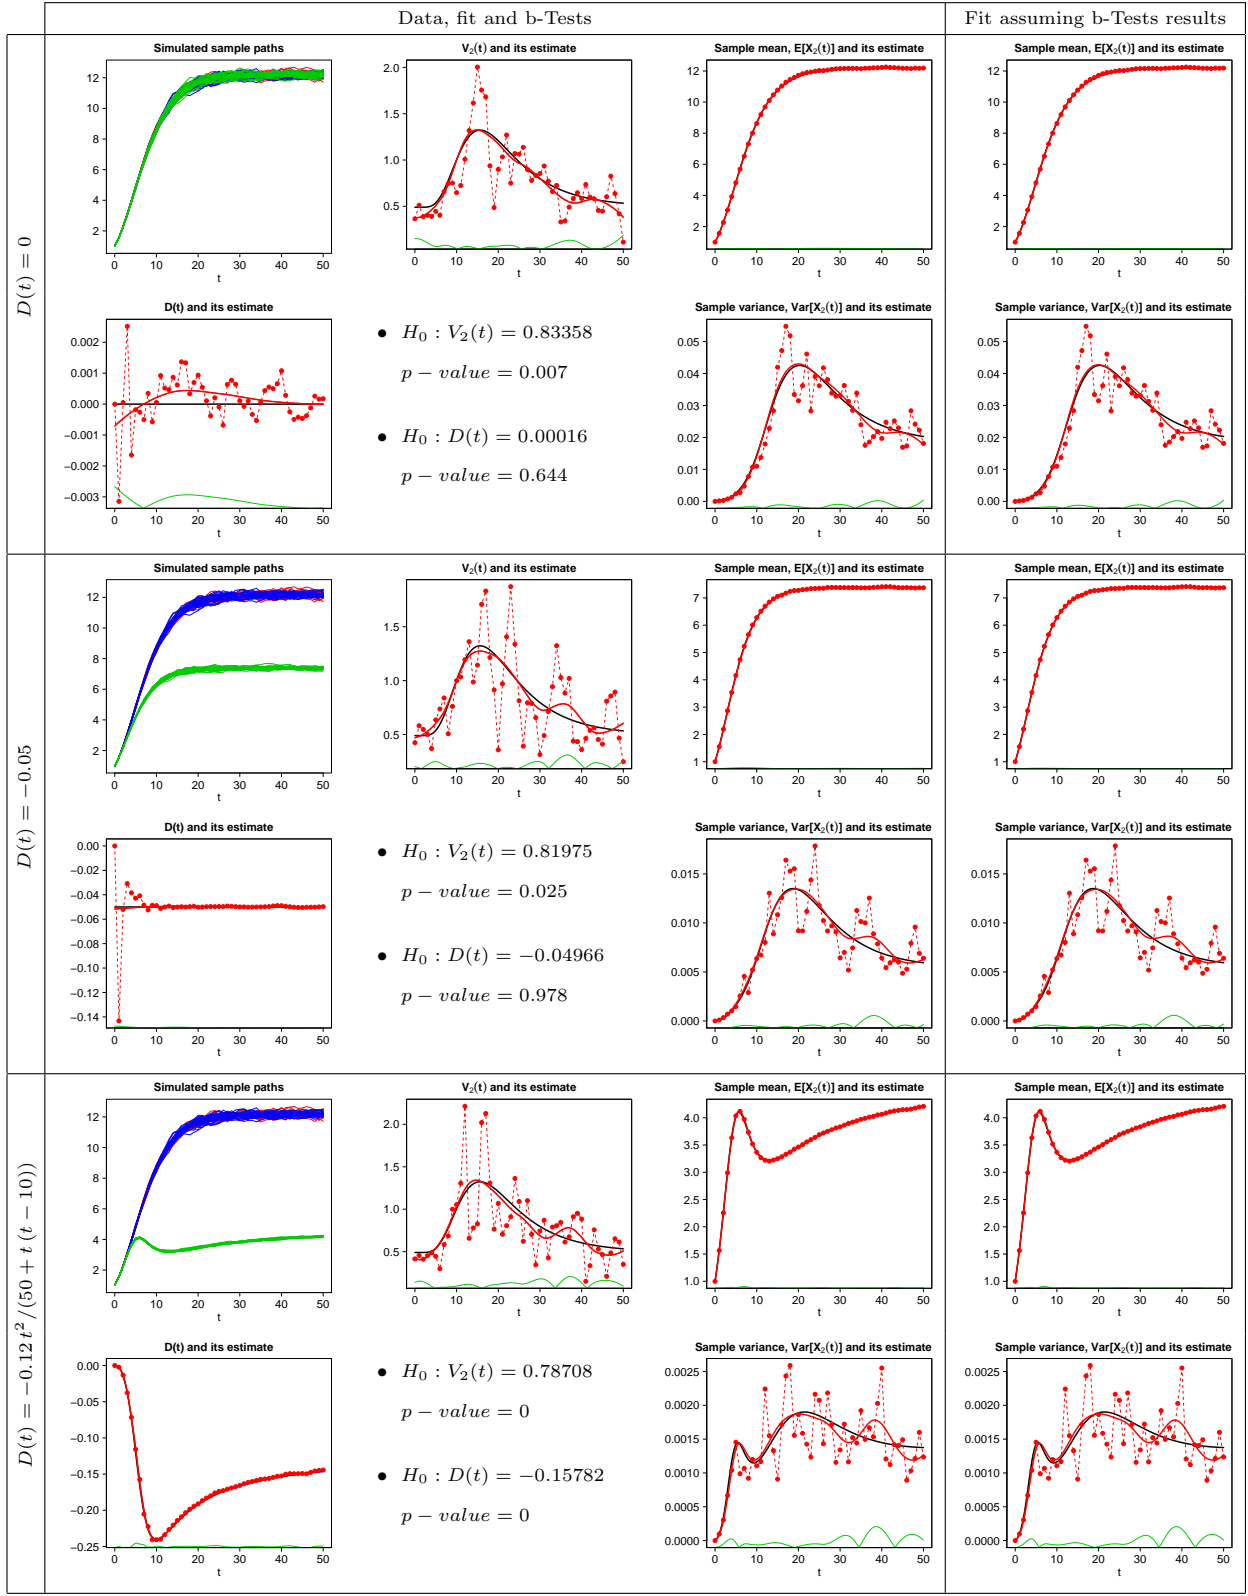

Table 30: Simulated data of the models (12), (13) and (15) (in red, blue and green, respectively) with  $\alpha = 0.5$ ,  $\beta = 0.2$ ,  $\sigma = 0.01$ ,  $V_1(t) = (0.7 + 10 \Lambda(t, 3, 0.5))^2$ ,  $C(t) = 0$ ,  $V_2(t) = (0.7 + 10 \Lambda(t, 3, 0.5))^2$  and different types of functions  $D(t)$ , estimates of  $D(t)$  and  $V_2(t)$  in model (15); concatenated bootstrap tests (b-Tests); and fit of simulated data of model (15).

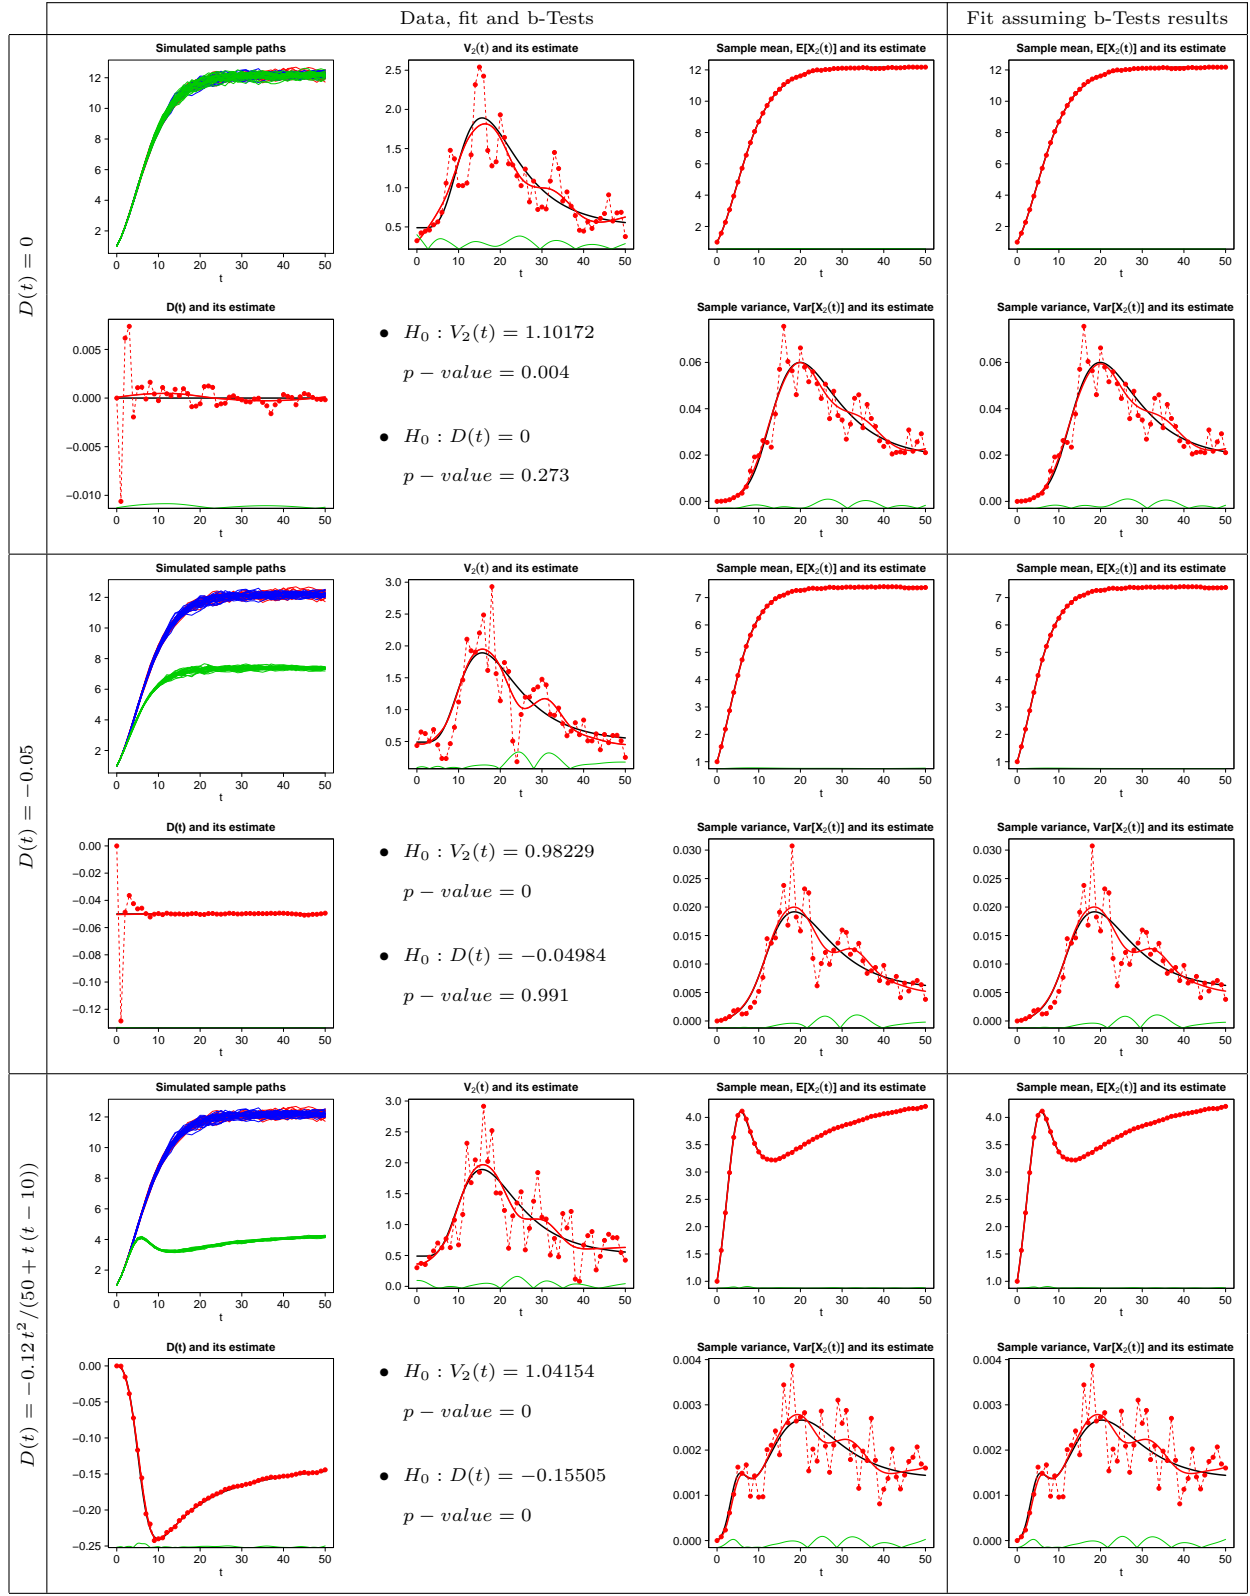

Table 31: Simulated data of the models (12), (13) and (15) (in red, blue and green, respectively) with  $\alpha = 0.5$ ,  $\beta = 0.2$ ,  $\sigma = 0.01$ ,  $V_1(t) = (0.7 + 10\Lambda(t, 3, 0.5))^2$ ,  $C(t) = 0$ ,  $V_2(t) = (0.7 + 15\Lambda(t, 3, 0.5))^2$  and different types of functions  $D(t)$ , estimates of  $D(t)$  and  $V_2(t)$  in model (15); concatenated bootstrap tests (b-Tests); and fit of simulated data of model (15).

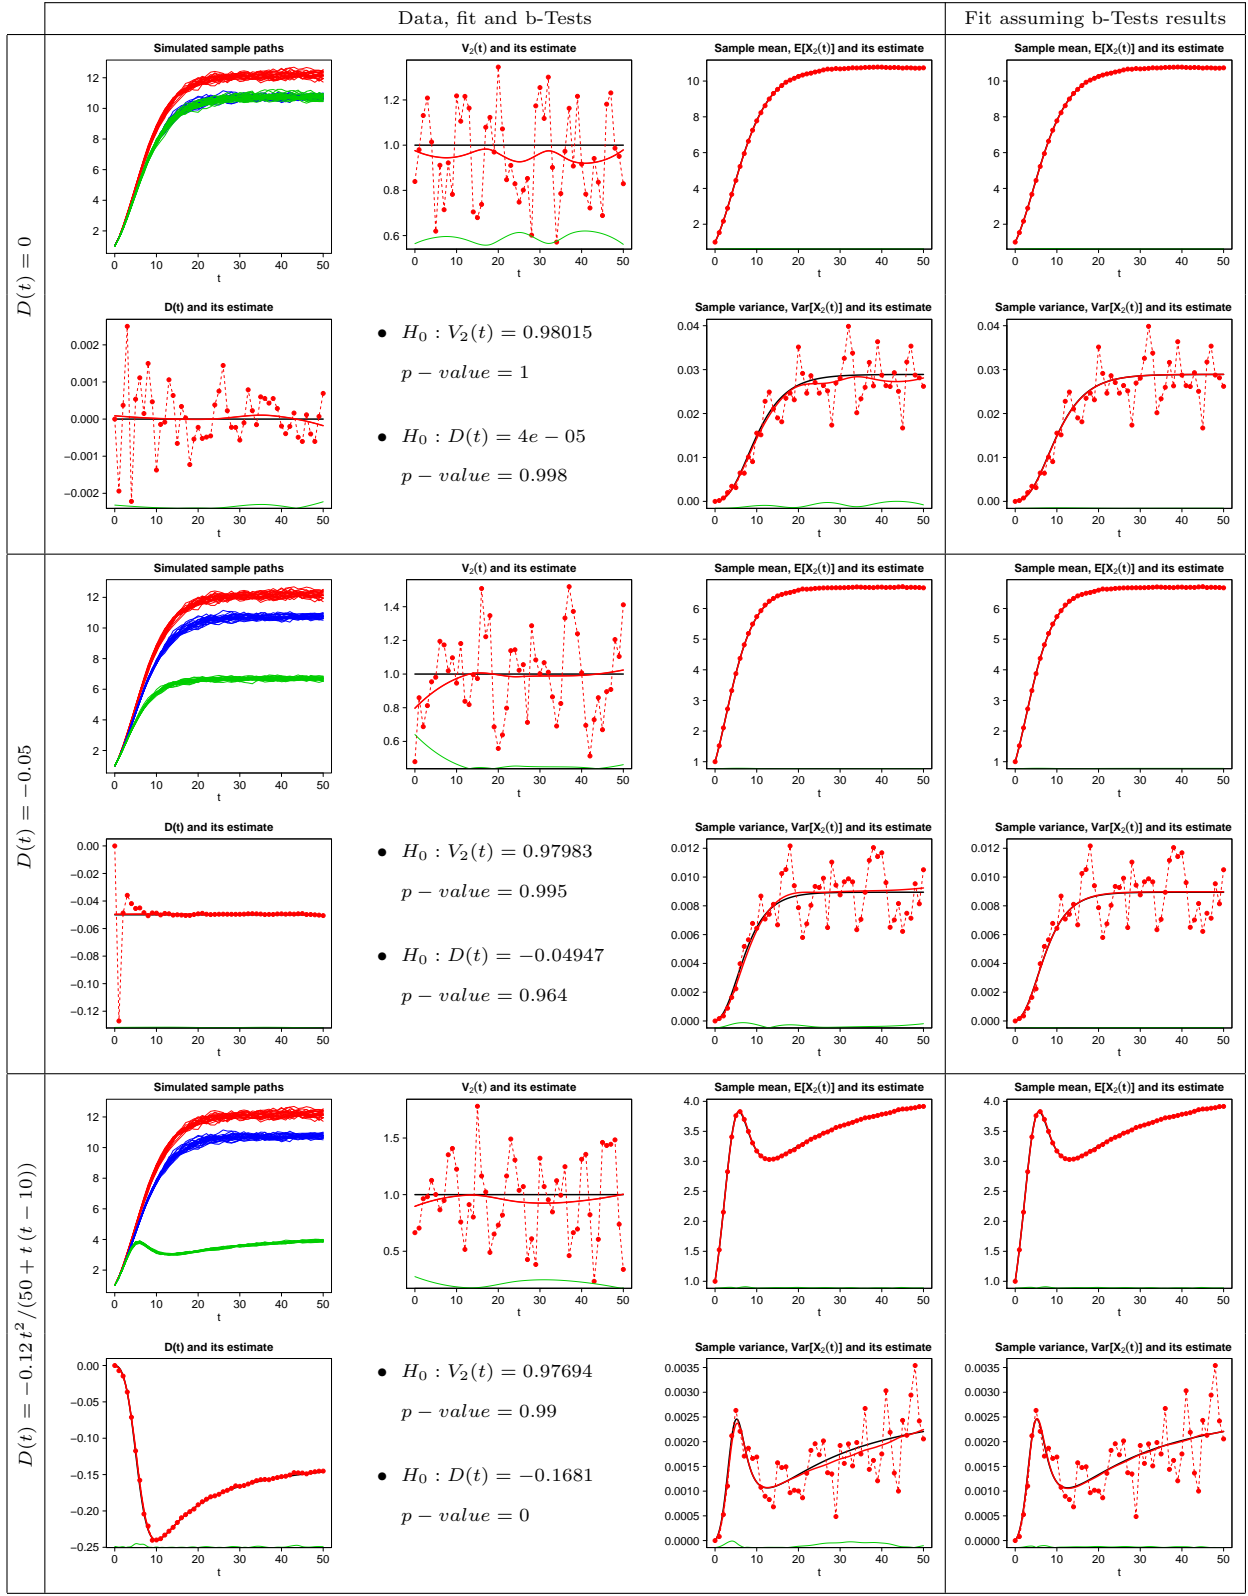

Table 32: Simulated data of the models (12), (13) and (15) (in red, blue and green, respectively) with  $\alpha = 0.5$ ,  $\beta = 0.2$ ,  $\sigma = 0.01$ ,  $V_1(t) = (0.7 + 10 \Lambda(t, 3, 0.5))^2$ ,  $C(t) = 0.025$ ,  $V_2(t) = 1$  and different types of functions  $D(t)$ , estimates of  $D(t)$  and  $V_2(t)$  in model (15); concatenated bootstrap tests (b-Tests); and fit of simulated data of model (15).

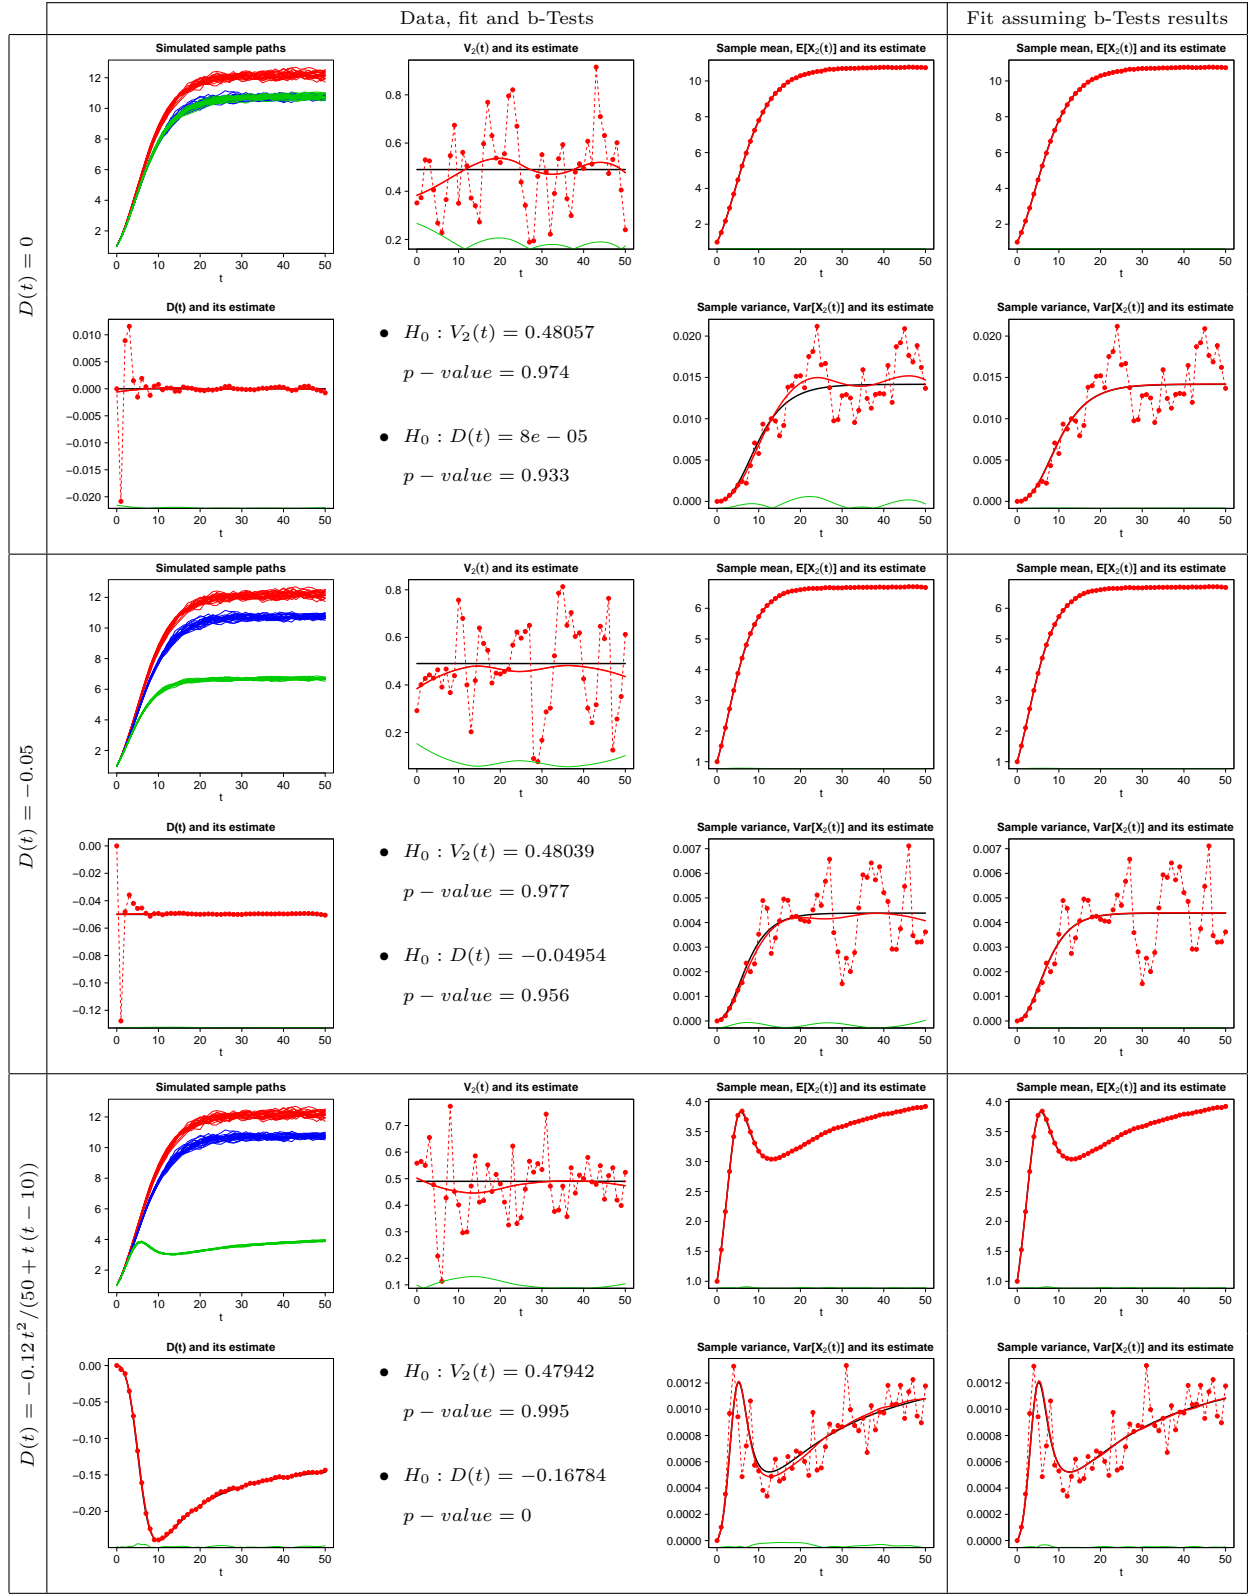

Table 33: Simulated data of the models (12), (13) and (15) (in red, blue and green, respectively) with  $\alpha = 0.5$ ,  $\beta = 0.2$ ,  $\sigma = 0.01$ ,  $V_1(t) = (0.7 + 10 \Lambda(t, 3, 0.5))^2$ ,  $C(t) = 0.025$ ,  $V_2(t) = 0.49$  and different types of functions  $D(t)$ , estimates of  $D(t)$  and  $V_2(t)$  in model (15); concatenated bootstrap tests (b-Tests); and fit of simulated data of model (15).

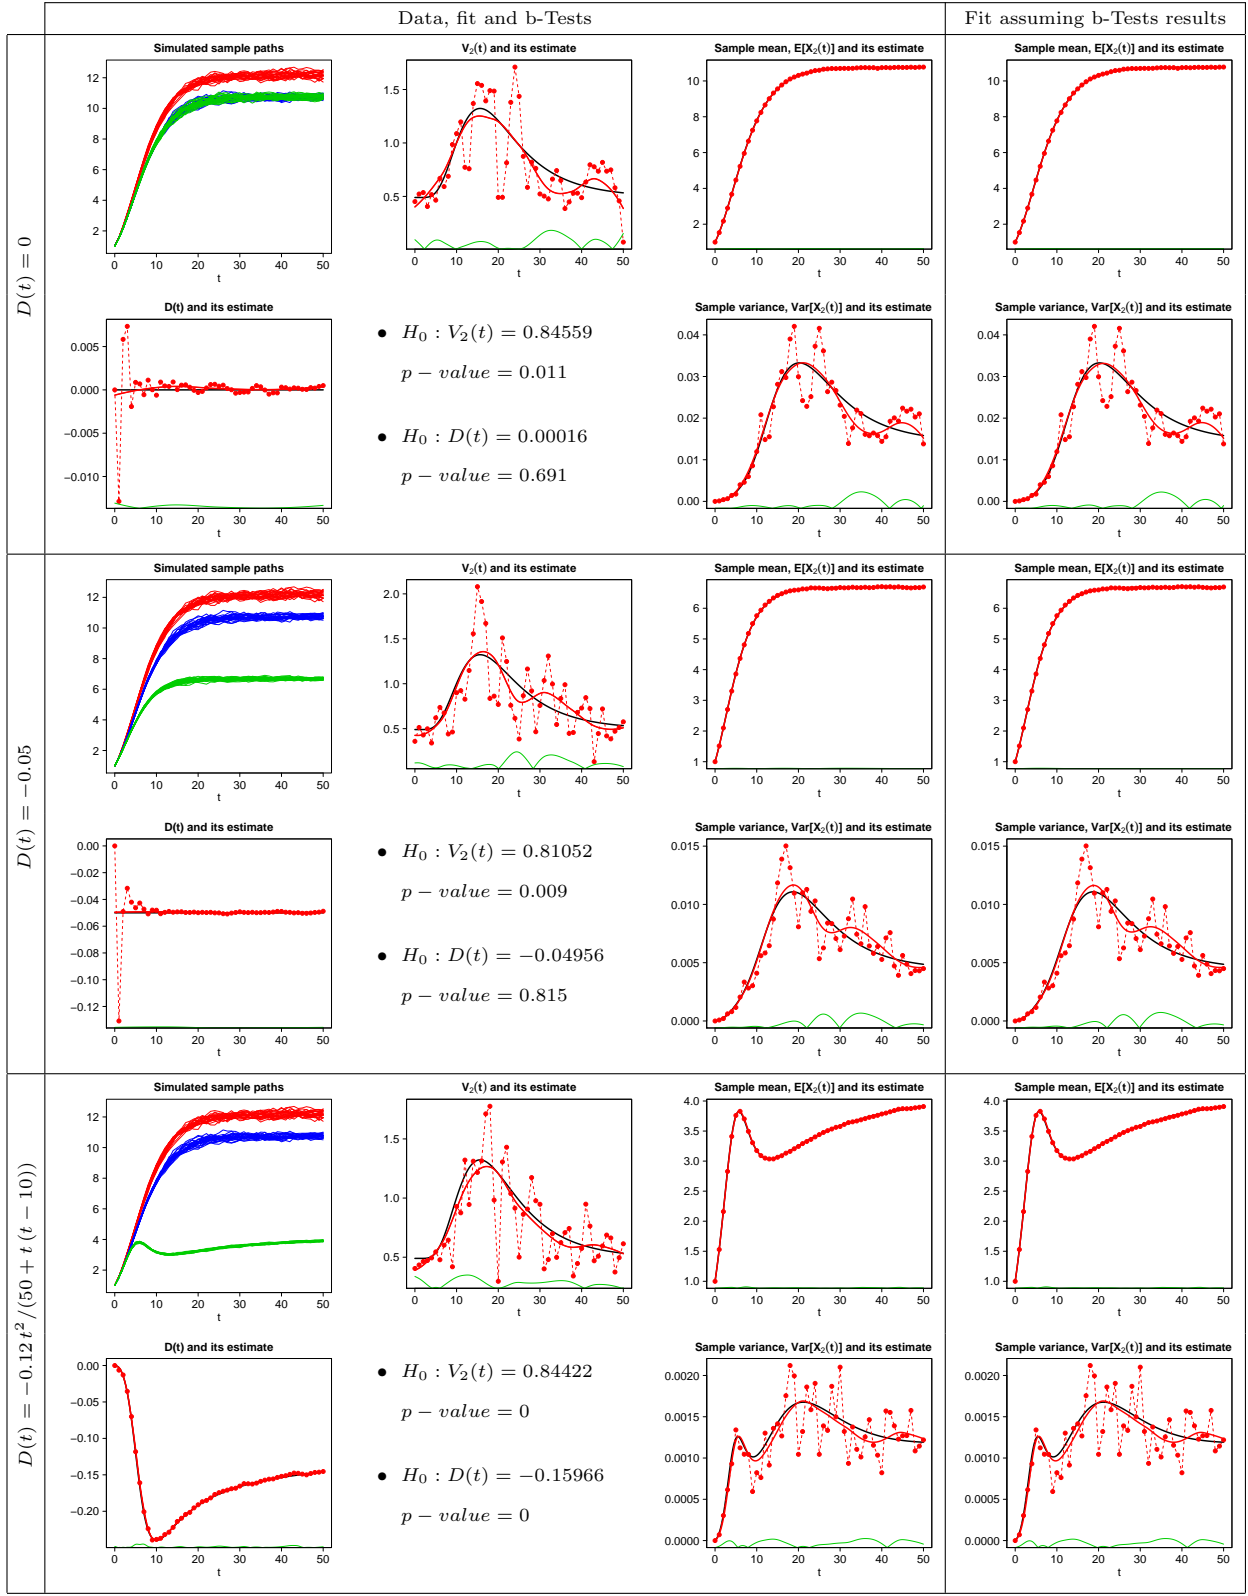

Table 34: Simulated data of the models (12), (13) and (15) (in red, blue and green, respectively) with  $\alpha = 0.5$ ,  $\beta = 0.2$ ,  $\sigma = 0.01$ ,  $V_1(t) = (0.7 + 10\Lambda(t, 3, 0.5))^2$ ,  $C(t) = 0.025$ ,  $V_2(t) = (0.7 + 10\Lambda(t, 3, 0.5))^2$  and different types of functions  $D(t)$ , estimates of  $D(t)$  and  $V_2(t)$  in model (15); concatenated bootstrap tests (b-Tests); and fit of simulated data of model (15).

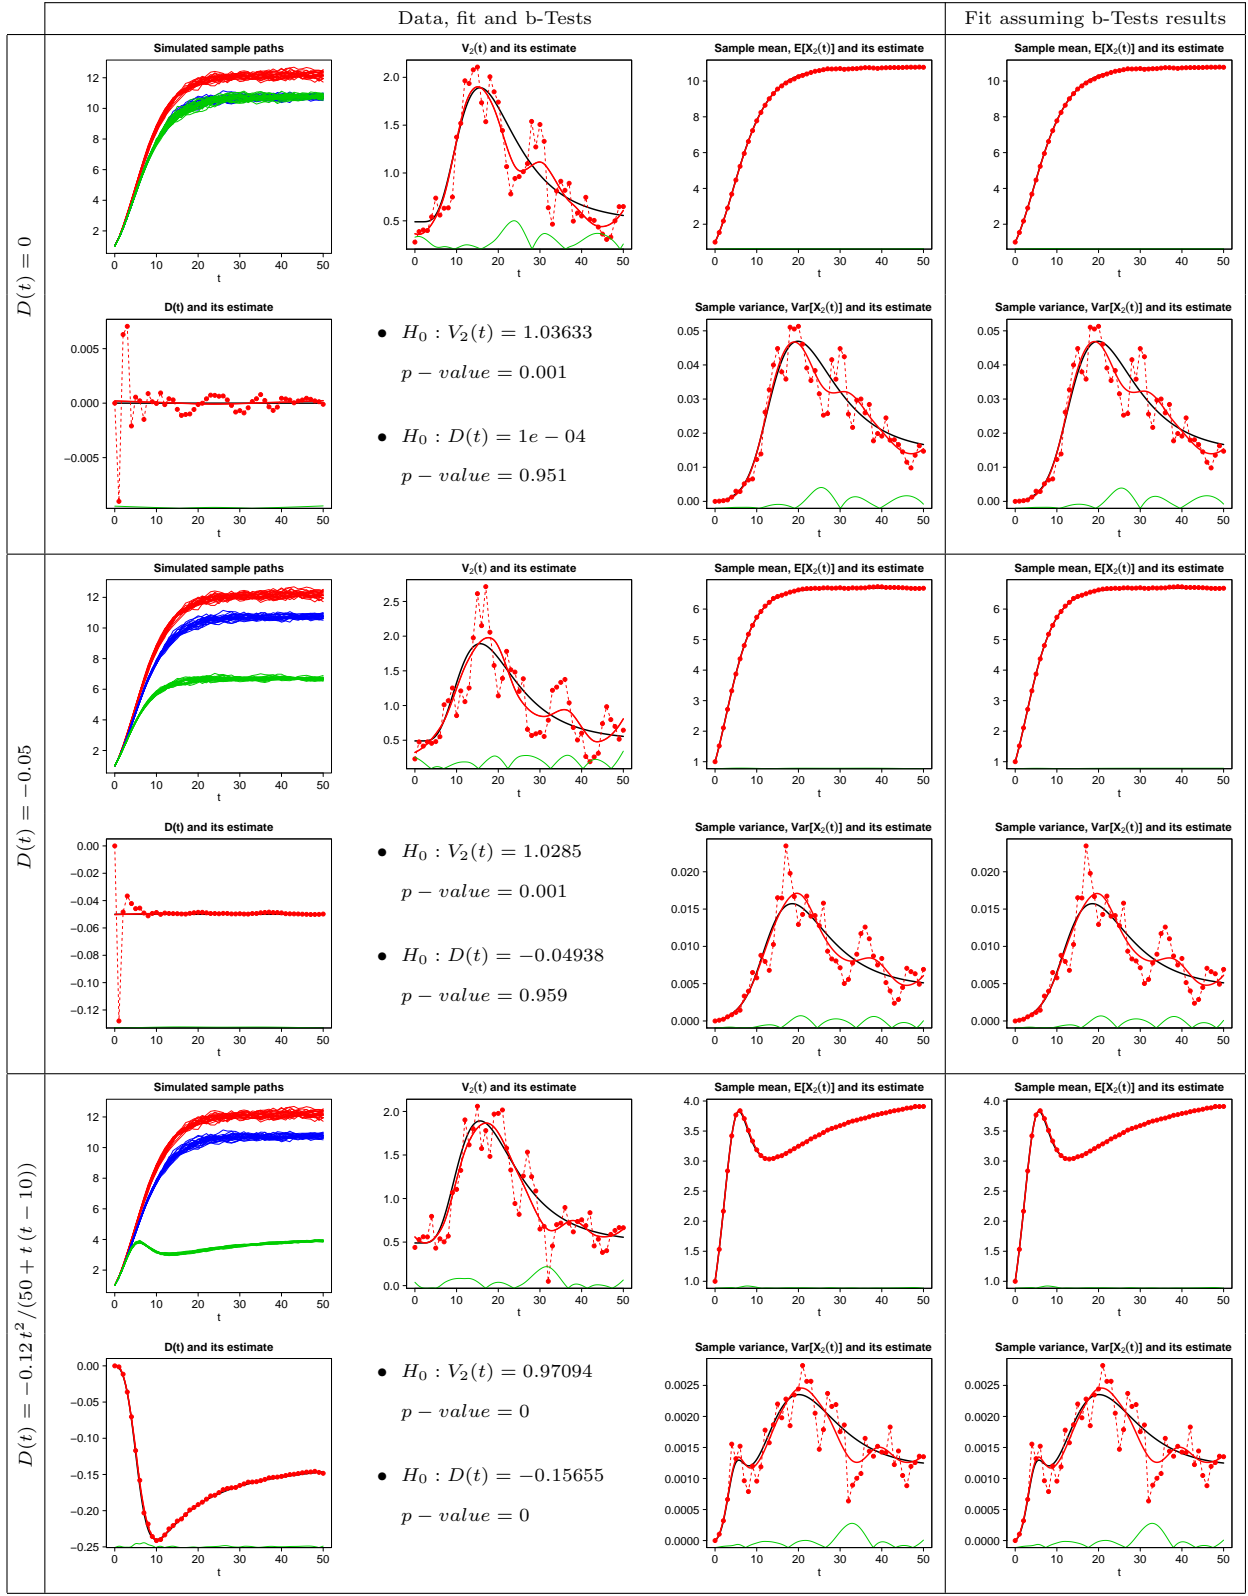

Table 35: Simulated data of the models (12), (13) and (15) (in red, blue and green, respectively) with  $\alpha = 0.5$ ,  $\beta = 0.2$ ,  $\sigma = 0.01$ ,  $V_1(t) = (0.7 + 10\Lambda(t, 3, 0.5))^2$ ,  $C(t) = 0.025$ ,  $V_2(t) = (0.7 + 15\Lambda(t, 3, 0.5))^2$  and different types of functions  $D(t)$ , estimates of  $D(t)$  and  $V_2(t)$  in model (15); concatenated bootstrap tests (b-Tests); and fit of simulated data of model (15).

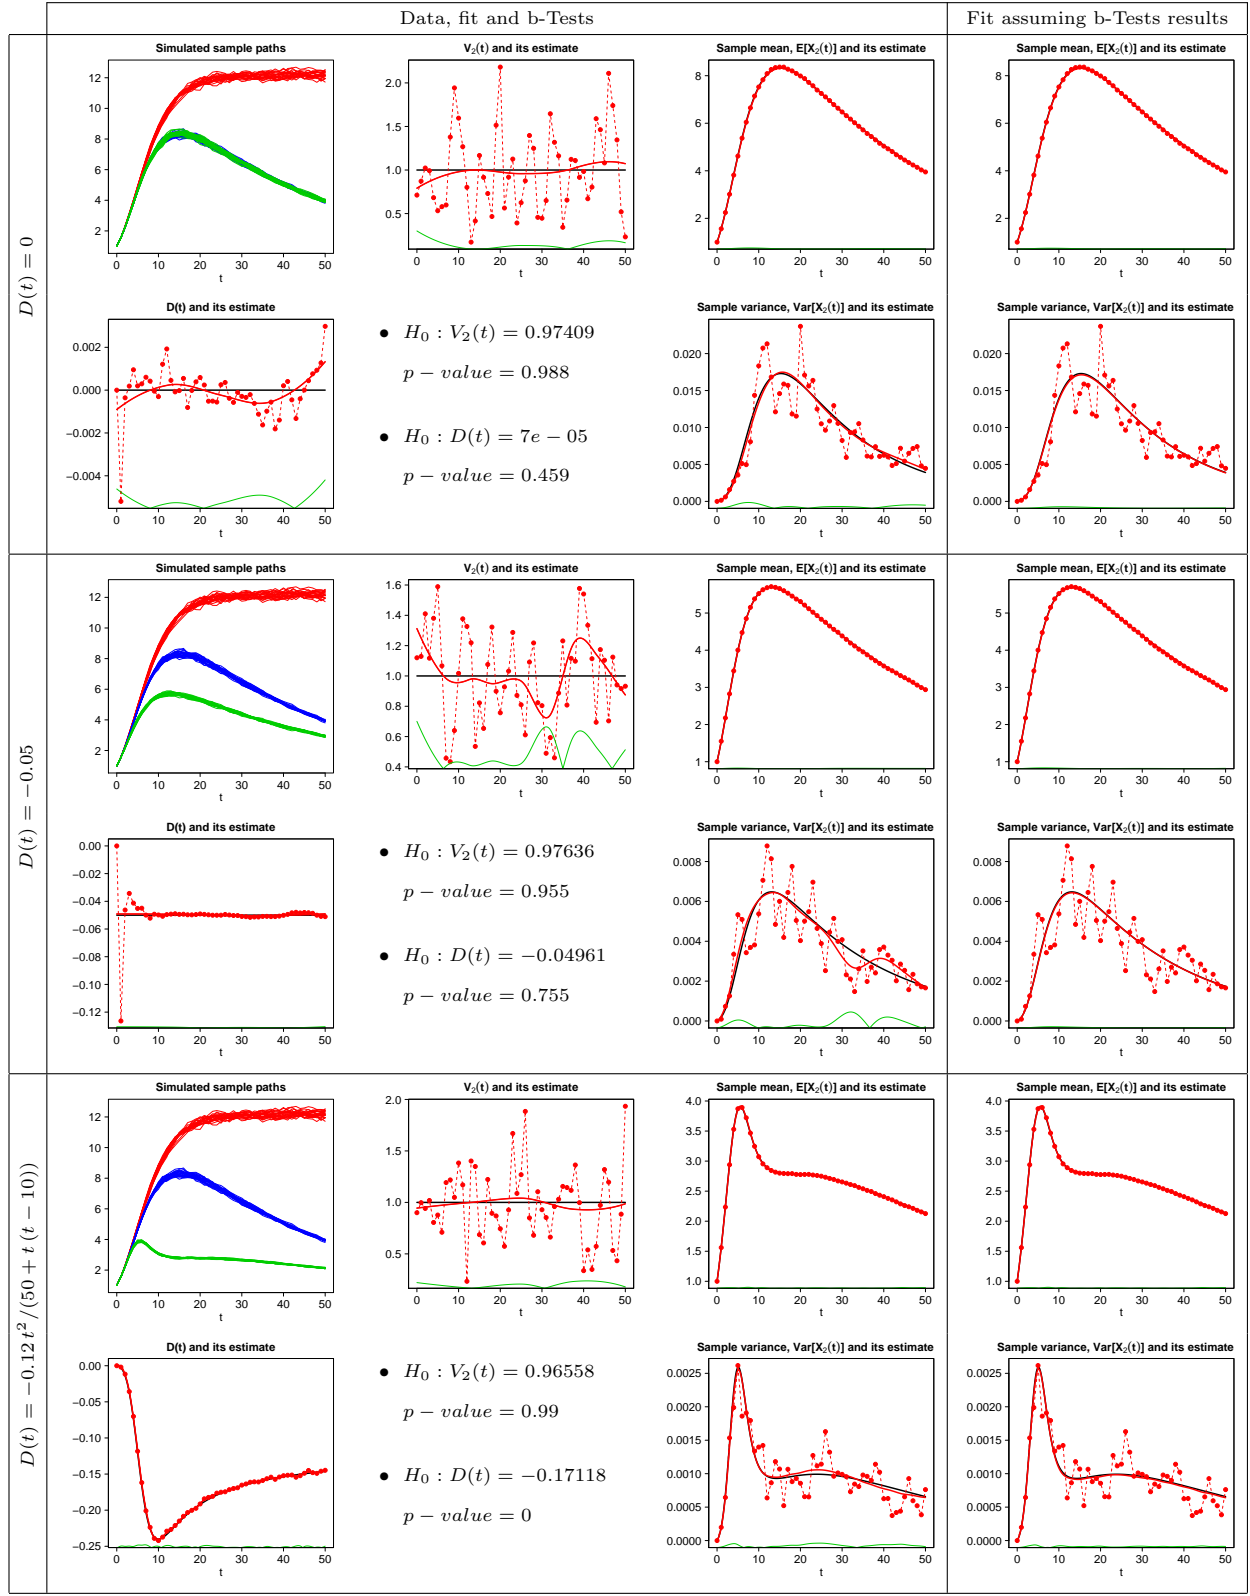

Table 36: Simulated data of the models (12), (13) and (15) (in red, blue and green, respectively) with  $\alpha = 0.5$ ,  $\beta = 0.2$ ,  $\sigma = 0.01$ ,  $V_1(t) = (0.7 + 10\Lambda(t, 3, 0.5))^2$ ,  $C(t) = 0.005t$ ,  $V_2(t) = 1$  and different types of functions  $D(t)$ , estimates of  $D(t)$  and  $V_2(t)$  in model (15); concatenated bootstrap tests (b-Tests); and fit of simulated data of model (15).

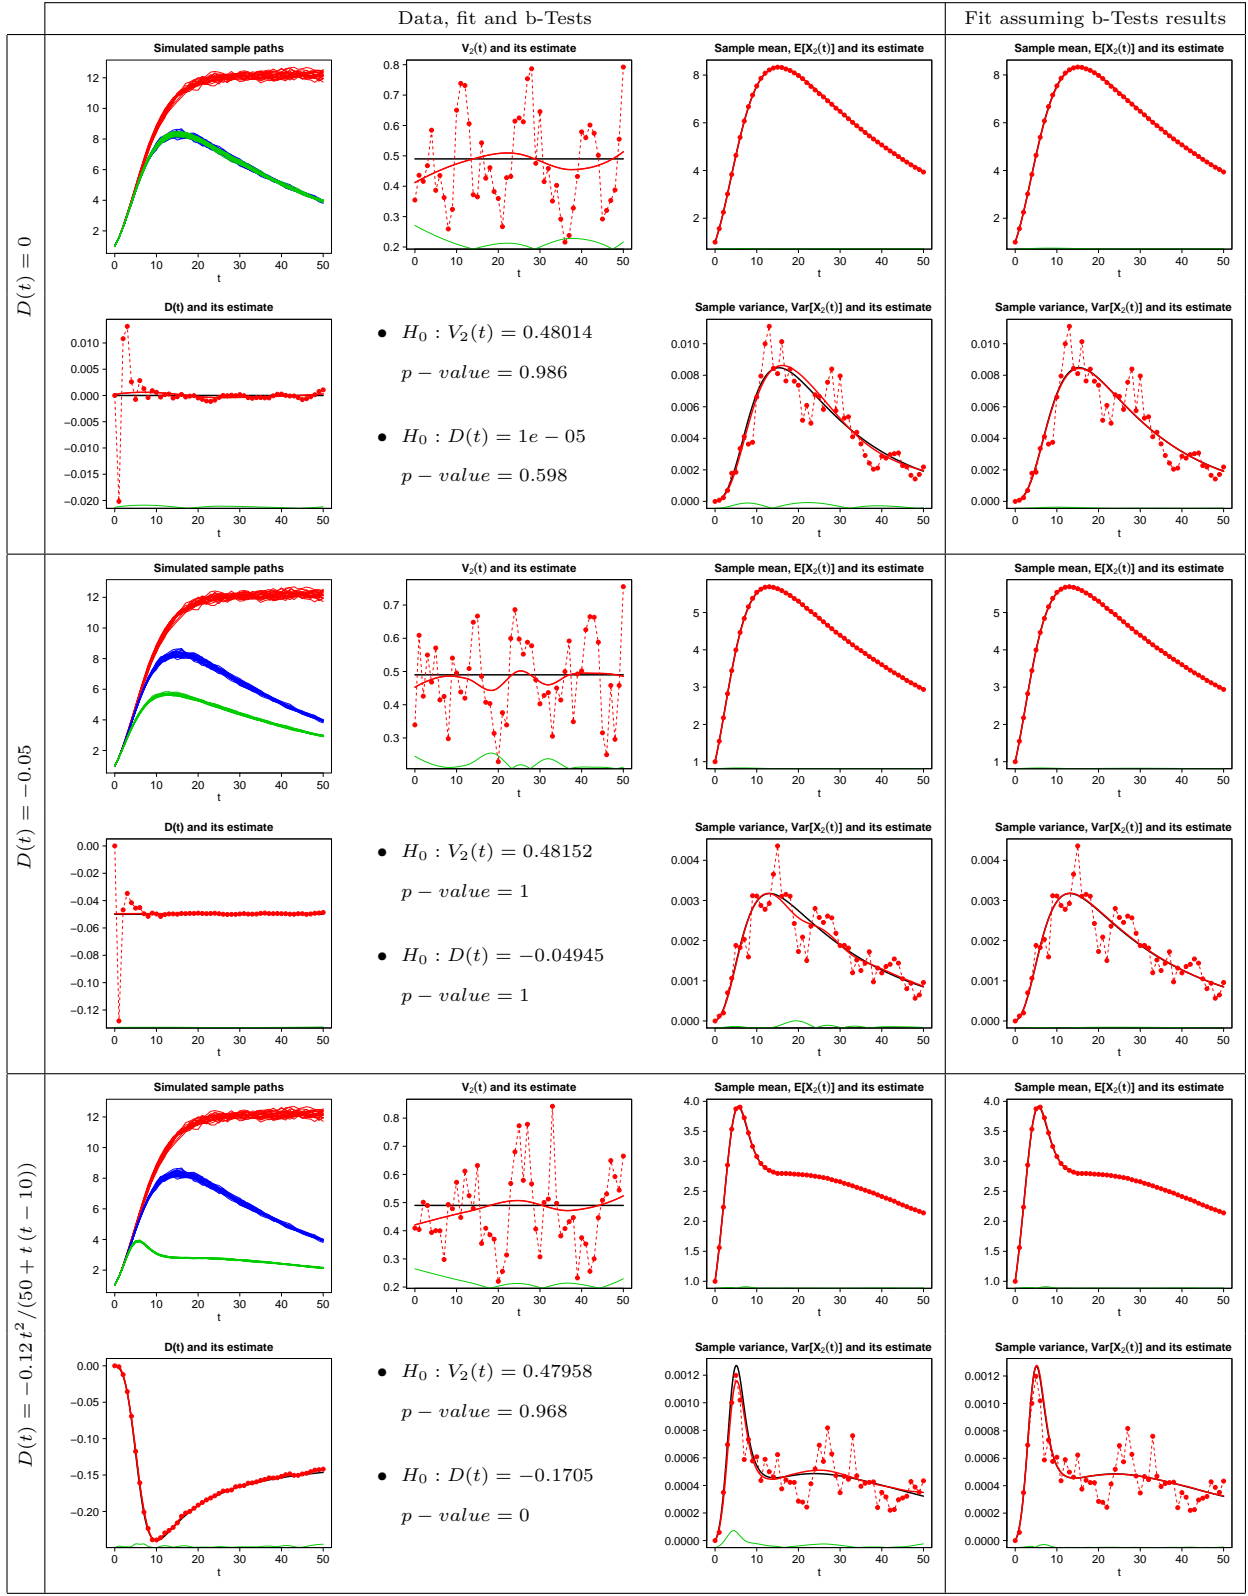

Table 37: Simulated data of the models (12), (13) and (15) (in red, blue and green, respectively) with  $\alpha = 0.5$ ,  $\beta = 0.2$ ,  $\sigma = 0.01$ ,  $V_1(t) = (0.7 + 10 \Lambda(t, 3, 0.5))^2$ ,  $C(t) = 0.005t$ ,  $V_2(t) = 0.49$  and different types of functions  $D(t)$ , estimates of  $D(t)$  and  $V_2(t)$  in model (15); concatenated bootstrap tests (b-Tests); and fit of simulated data of model (15).

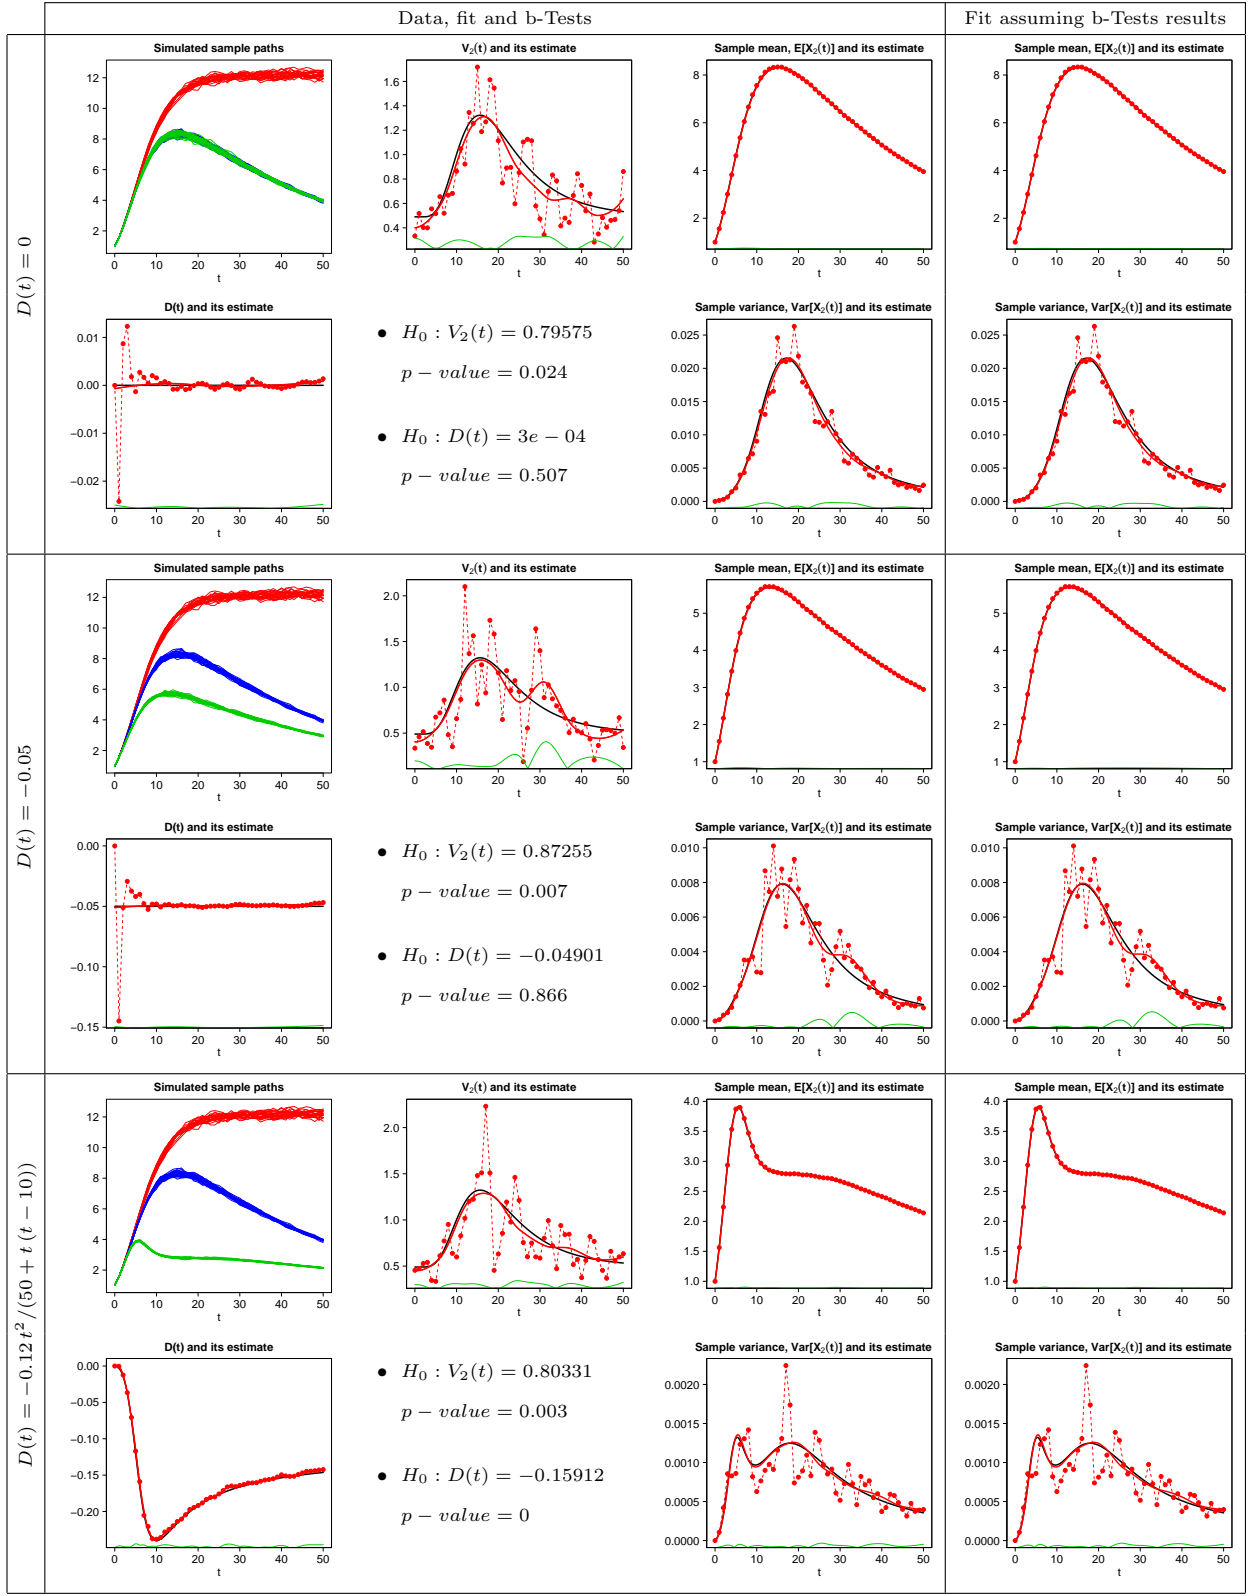

Table 38: Simulated data of the models (12), (13) and (15) (in red, blue and green, respectively) with  $\alpha = 0.5$ ,  $\beta = 0.2$ ,  $\sigma = 0.01$ ,  $V_1(t) = (0.7 + 10 \Lambda(t, 3, 0.5))^2$ ,  $C(t) = 0.005t$ ,  $V_2(t) = (0.7 + 10 \Lambda(t, 3, 0.5))^2$  and different types of functions  $D(t)$ , estimates of  $D(t)$  and  $V_2(t)$  in model (15); concatenated bootstrap tests (b-Tests); and fit of simulated data of model (15).

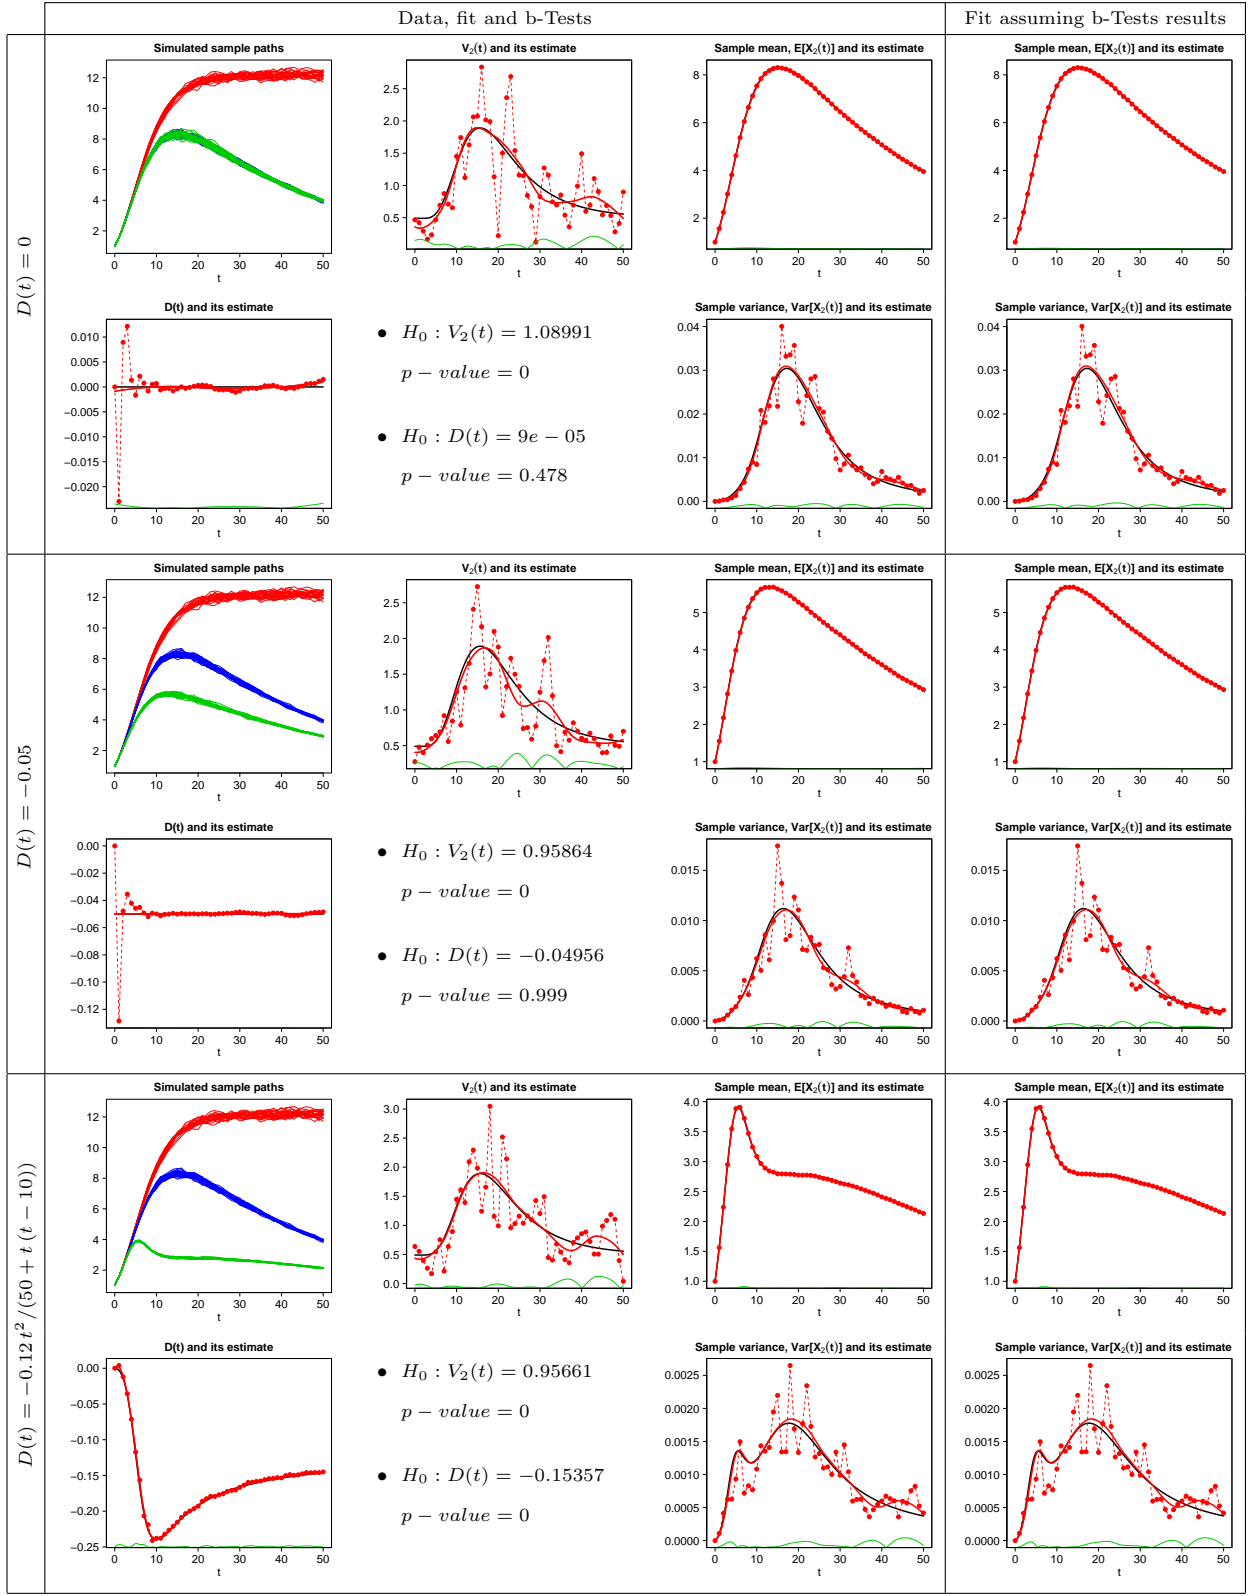

Table 39: Simulated data of the models (12), (13) and (15) (in red, blue and green, respectively) with  $\alpha = 0.5$ ,  $\beta = 0.2$ ,  $\sigma = 0.01$ ,  $V_1(t) = (0.7 + 10 \Lambda(t, 3, 0.5))^2$ ,  $C(t) = 0.005t$ ,  $V_2(t) = (0.7 + 15 \Lambda(t, 3, 0.5))^2$  and different types of functions  $D(t)$ , estimates of  $D(t)$  and  $V_2(t)$  in model (15); concatenated bootstrap tests (b-Tests); and fit of simulated data of model (15).
